# Supplementary material for: Homogeneous almost complex structures in dimension 6 with semi-simple isotropy
Source: arXiv:1401.8187 ancillary file (2014-02-12)
Supplement: Supplementary file 1 [file AKW_C-derivations.pdf]

We shall calculate the symmetries of the almost complex structure which comes in tables for isotropy  $su(2)$  and  $su(1,1)$ , rep  $W+C$ .  
 We calculate the derivations (inner+outer) and for the whole collection we check which commute with  $J$ . In this way we find  $Der\_C = \{A \in Der : AJ = JA\}$ .

## Section A1.1: isotropy $su(2)$ , rep $W+C$ .

```
> restart : with(DifferentialGeometry) : with(LieAlgebras) : with(Tensor) : with(Tools) :
with(ListTools) :
```

```
> StructureEquations := [ [ee, ii] = α * e, [jj, kk] = -α * e, [ee, ie] = ε/2 * ee + r * ii, [ii, ie] = ε/2
* ii - r * ee, [jj, ie] = ε/2 * jj - r * kk, [kk, ie] = ε/2 * kk + r * jj, [e, ie] = ε * e ], [ee, ii, jj,
kk, e, ie] :
```

```
> LI := LieAlgebraData(StructureEquations, VC);
LI := [ [e1, e2] = α e5, [e1, e6] = e1 ε + e2 r, [e2, e6] = -e1 r + e2 ε, [e3, e4] = -α e5, [e3,
e6] = e3 ε - e4 r, [e4, e6] = e3 r + e4 ε, [e5, e6] = 2 ε e5 ] (1.1)
```

```
> DGsetup(LI, [e], [f]) :
```

```
> Query( {α, r, ε}, "Jacobi");
true, {0}, [ {α = α, ε = ε, r = r} ], [ [ [e1, e2] = α e5, [e1, e6] = e1 ε + e2 r, [e2, e6] = -e1 r
+ e2 ε, [e3, e4] = -α e5, [e3, e6] = e3 ε - e4 r, [e4, e6] = e3 r + e4 ε, [e5, e6] = 2 ε e5 ]
] (1.2)
```

```
> LD := LeviDecomposition( )
LD := [ [e1, e2, e3, e4, e5, e6], [ ] ] (1.3)
```

We shall exclude the possibility that  $r=0$ . We also have  $\varepsilon=0 \vee \varepsilon=1$ .

```
> J := Matrix( [ [0, -cos(a) sin(b), -sin(a) sin(b), -cos(b), 0, 0], [cos(a) sin(b), 0,
cos(b), -sin(a) sin(b), 0, 0], [sin(a) sin(b), -cos(b), 0, cos(a) sin(b), 0, 0],
cos(a) sin(b), 0, 0], [cos(b), sin(a) sin(b), -cos(a) sin(b), 0, 0, 0], [0, 0, 0, 0, 0, -1],
[0, 0, 0, 0, 1, 0]]);
```

$$J := \begin{bmatrix} 0 & -\cos(a) \sin(b) & -\sin(a) \sin(b) & -\cos(b) & 0 & 0 \\ \cos(a) \sin(b) & 0 & \cos(b) & -\sin(a) \sin(b) & 0 & 0 \\ \sin(a) \sin(b) & -\cos(b) & 0 & \cos(a) \sin(b) & 0 & 0 \\ \cos(b) & \sin(a) \sin(b) & -\cos(a) \sin(b) & 0 & 0 & 0 \\ 0 & 0 & 0 & 0 & 0 & -1 \\ 0 & 0 & 0 & 0 & 1 & 0 \end{bmatrix} \quad (1.4)$$

```
> deri := Derivations("Full");
```



$$\begin{bmatrix} 0 & 0 & 0 & 0 & 0 & 0 \\ 0 & 0 & 0 & 0 & 0 & 0 \\ 0 & 0 & 0 & 0 & 0 & 0 \\ 0 & 0 & 0 & 0 & 0 & 0 \\ 0 & 0 & 0 & 0 & 0 & 1 \\ 0 & 0 & 0 & 0 & 0 & 0 \end{bmatrix}$$

$\triangleright R := \text{add}(r||u \cdot \text{deri}[u], u = 1 \dots \text{nops}(\text{deri}));$

$$R := \begin{bmatrix} r1, r2, r3, r4, 0, r5, \\ \begin{bmatrix} -r2, r1, r4, -r3, 0, r6 \end{bmatrix}, \\ \begin{bmatrix} -r3, -r4, r1, r7, 0, r8 \end{bmatrix}, \\ \begin{bmatrix} -r4, r3, -r7, r1, 0, r9 \end{bmatrix}, \\ \begin{bmatrix} \frac{r5 r \alpha}{\epsilon^2 + r^2} - \frac{r6 \alpha \epsilon}{\epsilon^2 + r^2}, \frac{r5 \alpha \epsilon}{\epsilon^2 + r^2} + \frac{r6 r \alpha}{\epsilon^2 + r^2}, \frac{r8 r \alpha}{\epsilon^2 + r^2} + \frac{r9 \alpha \epsilon}{\epsilon^2 + r^2}, -\frac{r8 \alpha \epsilon}{\epsilon^2 + r^2} + \frac{r9 r \alpha}{\epsilon^2 + r^2}, \\ 2 r1, r10 \end{bmatrix}, \\ \begin{bmatrix} 0, 0, 0, 0, 0, 0 \end{bmatrix} \end{bmatrix} \quad (1.6)$$

$\triangleright \text{com} := R.J - J.R :$

$\triangleright \text{eq} := \{\text{seq}(\text{seq}(\text{com}[u, o], u = 1 \dots 6), o = 1 \dots 6)\};$

$$\text{eq} := \left\{ 0, r10, r5, r6, r8, r9, -2 r1, -r10, r2 \cos(b) - r7 \cos(b), r7 \cos(b) - r2 \cos(b), \right. \quad (1.7)$$

$$\left. -r2 \sin(a) \sin(b) + r7 \sin(a) \sin(b), r2 \sin(a) \sin(b) - r7 \sin(a) \sin(b), -\frac{r5 r \alpha}{\epsilon^2 + r^2} \right.$$

$$\left. + \frac{r6 \alpha \epsilon}{\epsilon^2 + r^2}, -\frac{r5 \alpha \epsilon}{\epsilon^2 + r^2} - \frac{r6 r \alpha}{\epsilon^2 + r^2}, -\frac{r8 r \alpha}{\epsilon^2 + r^2} - \frac{r9 \alpha \epsilon}{\epsilon^2 + r^2}, \frac{r8 \alpha \epsilon}{\epsilon^2 + r^2} - \frac{r9 r \alpha}{\epsilon^2 + r^2}, \right.$$

$$\left. -\left(\frac{r5 r \alpha}{\epsilon^2 + r^2} - \frac{r6 \alpha \epsilon}{\epsilon^2 + r^2}\right) \cos(b) - \left(\frac{r5 \alpha \epsilon}{\epsilon^2 + r^2} + \frac{r6 r \alpha}{\epsilon^2 + r^2}\right) \sin(a) \sin(b) + \left(\frac{r8 r \alpha}{\epsilon^2 + r^2} \right.$$

$$\left. + \frac{r9 \alpha \epsilon}{\epsilon^2 + r^2}\right) \cos(a) \sin(b), -\cos(b) r5 - \sin(a) \sin(b) r6 + \cos(a) \sin(b) r8,$$

$$\begin{aligned}
& - \left( \frac{r^5 r \alpha}{\epsilon^2 + r^2} - \frac{r^6 \alpha \epsilon}{\epsilon^2 + r^2} \right) \cos(a) \sin(b) - \left( \frac{r^8 r \alpha}{\epsilon^2 + r^2} + \frac{r^9 \alpha \epsilon}{\epsilon^2 + r^2} \right) \cos(b) + \left( - \frac{r^8 \alpha \epsilon}{\epsilon^2 + r^2} \right. \\
& + \left. \frac{r^9 r \alpha}{\epsilon^2 + r^2} \right) \sin(a) \sin(b), - \left( \frac{r^5 r \alpha}{\epsilon^2 + r^2} - \frac{r^6 \alpha \epsilon}{\epsilon^2 + r^2} \right) \sin(a) \sin(b) + \left( \frac{r^5 \alpha \epsilon}{\epsilon^2 + r^2} \right. \\
& + \left. \frac{r^6 r \alpha}{\epsilon^2 + r^2} \right) \cos(b) - \left( - \frac{r^8 \alpha \epsilon}{\epsilon^2 + r^2} + \frac{r^9 r \alpha}{\epsilon^2 + r^2} \right) \cos(a) \sin(b), \left( \frac{r^5 \alpha \epsilon}{\epsilon^2 + r^2} \right. \\
& + \left. \frac{r^6 r \alpha}{\epsilon^2 + r^2} \right) \cos(a) \sin(b) + \left( \frac{r^8 r \alpha}{\epsilon^2 + r^2} + \frac{r^9 \alpha \epsilon}{\epsilon^2 + r^2} \right) \sin(a) \sin(b) + \left( - \frac{r^8 \alpha \epsilon}{\epsilon^2 + r^2} \right. \\
& + \left. \frac{r^9 r \alpha}{\epsilon^2 + r^2} \right) \cos(b), -\cos(a) \sin(b) r^5 - \cos(b) r^8 + \sin(a) \sin(b) r^9, \\
& \cos(a) \sin(b) r^6 + \sin(a) \sin(b) r^8 + \cos(b) r^9, -\sin(a) \sin(b) r^5 + \cos(b) r^6 \\
& - \cos(a) \sin(b) r^9 \}
\end{aligned}$$

> *derisol* := solve(eq, {seq(r||u, u = 1..nops(deri)), a, b, α, r, ε});

*derisol* := {a = a, α = α, b = b, ε = ε, r = r, r1 = 0, r10 = 0, r2 = r7, r3 = r3, r4 = r4, r5 = 0, r6 = 0, r7 = r7, r8 = 0, r9 = 0}, {a = 0, α = α, b =  $\frac{1}{2} \pi$ , ε = ε, r = r, r1 = 0, r10 = 0, r2 = r2, r3 = r3, r4 = r4, r5 = 0, r6 = 0, r7 = r7, r8 = 0, r9 = 0}

(1.8)

> subs(*derisol*[1], R);

$$\begin{bmatrix}
0 & r7 & r3 & r4 & 0 & 0 \\
-r7 & 0 & r4 & -r3 & 0 & 0 \\
-r3 & -r4 & 0 & r7 & 0 & 0 \\
-r4 & r3 & -r7 & 0 & 0 & 0 \\
0 & 0 & 0 & 0 & 0 & 0 \\
0 & 0 & 0 & 0 & 0 & 0
\end{bmatrix}$$

(1.9)

> subs(*derisol*[2], R);

$$\begin{bmatrix}
0 & r2 & r3 & r4 & 0 & 0 \\
-r2 & 0 & r4 & -r3 & 0 & 0 \\
-r3 & -r4 & 0 & r7 & 0 & 0 \\
-r4 & r3 & -r7 & 0 & 0 & 0 \\
0 & 0 & 0 & 0 & 0 & 0 \\
0 & 0 & 0 & 0 & 0 & 0
\end{bmatrix}$$

(1.10)

>

> Conclusion: for A1.1 the Symmetry algebra of the model is 3+6=9 dimensional, as expected.

>

### Section A3.1: isotropy $su(1,1)$ , rep $W+C$ .

> restart : with(DifferentialGeometry) : with(LieAlgebras) : with(Tensor) : with(Tools) :  
with(ListTools) :

> StructureEquations :=  $\left[ [x, y] = p1 \cdot e, [ix, iy] = p2 \cdot e, [x, ie] = \frac{\varepsilon}{2} \cdot x + \frac{ix}{p2}, [ix, ie] = \frac{\varepsilon}{2} \cdot ix - \frac{x}{p1}, [y, ie] = \frac{\varepsilon}{2} \cdot y + \frac{iy}{p2}, [iy, ie] = \frac{\varepsilon}{2} \cdot iy - \frac{y}{p1}, [e, ie] = \varepsilon \cdot e \right], [x, ix, y, iy, e, ie] :$

> L1 := LieAlgebraData(StructureEquations, VC);

$$L1 := \left[ [e1, e3] = p1 e5, [e1, e6] = \frac{e2}{p2} + \frac{1}{2} \varepsilon e1, [e2, e4] = p2 e5, [e2, e6] = \frac{1}{2} \varepsilon e2 - \frac{e1}{p1}, [e3, e6] = \frac{e4}{p2} + \frac{1}{2} \varepsilon e3, [e4, e6] = \frac{1}{2} \varepsilon e4 - \frac{e3}{p1}, [e5, e6] = \varepsilon e5 \right] \quad (2.1)$$

> DGsetup(L1, [e], [f]) :

> Query({p1, p2, ε}, "Jacobi");

$$\begin{aligned} & true, \{0\}, \left[ \left\{ \varepsilon = \varepsilon, p1 = p1, p2 = p2 \right\}, \left[ \left[ [e1, e3] = p1 e5, [e1, e6] = \frac{e2}{p2} + \frac{1}{2} \varepsilon e1, [e2, e4] \right. \right. \right. \\ & \quad \left. \left. \left. = p2 e5, [e2, e6] = \frac{1}{2} \varepsilon e2 - \frac{e1}{p1}, [e3, e6] = \frac{e4}{p2} + \frac{1}{2} \varepsilon e3, [e4, e6] = \frac{1}{2} \varepsilon e4 - \frac{e3}{p1}, \right. \right. \right. \\ & \quad \left. \left. \left. [e5, e6] = \varepsilon e5 \right] \right] \right] \quad (2.2) \end{aligned}$$

> LD := LeviDecomposition( )

$$LD := [[e1, e2, e3, e4, e5, e6], [ ]] \quad (2.3)$$

>

We shall exclude the possibility that  $r=0$ . We also have  $\varepsilon=0 \vee \varepsilon=1$ .

>

> J := Matrix([ [ r, -(r^2 + 1)/t, 0, 0, 0, 0], [t, -r, 0, 0, 0, 0], [0, 0, r, -(r^2 + 1)/t, 0, 0], [0, 0, t, -r, 0, 0], [0, 0, 0, 0, 0, -1], [0, 0, 0, 0, 1, 0]]);

$$J := \begin{bmatrix} r & -\frac{r^2+1}{t} & 0 & 0 & 0 & 0 \\ t & -r & 0 & 0 & 0 & 0 \\ 0 & 0 & r & -\frac{r^2+1}{t} & 0 & 0 \\ 0 & 0 & t & -r & 0 & 0 \\ 0 & 0 & 0 & 0 & 0 & -1 \\ 0 & 0 & 0 & 0 & 1 & 0 \end{bmatrix} \quad (2.4)$$

> deri := Derivations("Full");

(2.5)

$$\begin{aligned}
\text{deri} := & \begin{bmatrix} \begin{bmatrix} 1 & 0 & 0 & 0 & 0 & 0 \\ 0 & 1 & 0 & 0 & 0 & 0 \\ 0 & 0 & 0 & 0 & 0 & 0 \\ 0 & 0 & 0 & 0 & 0 & 0 \\ 0 & 0 & 0 & 0 & 1 & 0 \\ 0 & 0 & 0 & 0 & 0 & 0 \end{bmatrix}, \begin{bmatrix} 0 & 1 & 0 & 0 & 0 & 0 \\ -\frac{pl}{p^2} & 0 & 0 & 0 & 0 & 0 \\ 0 & 0 & 0 & 1 & 0 & 0 \\ 0 & 0 & -\frac{pl}{p^2} & 0 & 0 & 0 \\ 0 & 0 & 0 & 0 & 0 & 0 \\ 0 & 0 & 0 & 0 & 0 & 0 \end{bmatrix}, \begin{bmatrix} 0 & 0 & 1 & 0 & 0 & 0 \\ 0 & 0 & 0 & 1 & 0 & 0 \\ 0 & 0 & 0 & 0 & 0 & 0 \\ 0 & 0 & 0 & 0 & 0 & 0 \\ 0 & 0 & 0 & 0 & 0 & 0 \\ 0 & 0 & 0 & 0 & 0 & 0 \end{bmatrix}, \\
& \begin{bmatrix} 0 & 0 & 0 & 0 & 0 & 1 \\ 0 & 0 & 0 & 0 & 0 & 0 \\ 0 & 0 & 0 & 0 & 0 & 0 \\ 0 & 0 & 0 & 0 & 0 & 0 \\ 0 & 0 & \frac{2 \varepsilon pl^2 p2}{\varepsilon^2 pl p2 + 4} & -\frac{4 pl p2}{\varepsilon^2 pl p2 + 4} & 0 & 0 \\ 0 & 0 & 0 & 0 & 0 & 0 \end{bmatrix}, \\
& \begin{bmatrix} 0 & 0 & 0 & 0 & 0 & 0 \\ 0 & 0 & 0 & 0 & 0 & 1 \\ 0 & 0 & 0 & 0 & 0 & 0 \\ 0 & 0 & 0 & 0 & 0 & 0 \\ 0 & 0 & \frac{4 pl p2}{\varepsilon^2 pl p2 + 4} & \frac{2 \varepsilon p2^2 pl}{\varepsilon^2 pl p2 + 4} & 0 & 0 \\ 0 & 0 & 0 & 0 & 0 & 0 \end{bmatrix}, \begin{bmatrix} 0 & 0 & 0 & 0 & 0 & 0 \\ 0 & 0 & 0 & 0 & 0 & 0 \\ 1 & 0 & 0 & 0 & 0 & 0 \\ 0 & 1 & 0 & 0 & 0 & 0 \\ 0 & 0 & 0 & 0 & 0 & 0 \\ 0 & 0 & 0 & 0 & 0 & 0 \end{bmatrix}, \begin{bmatrix} 0 & 0 & 0 & 0 & 0 & 0 \\ 0 & 0 & 0 & 0 & 0 & 0 \\ 0 & 0 & 1 & 0 & 0 & 0 \\ 0 & 0 & 0 & 1 & 0 & 0 \\ 0 & 0 & 0 & 0 & 1 & 0 \\ 0 & 0 & 0 & 0 & 0 & 0 \end{bmatrix}, \\
& \begin{bmatrix} 0 & 0 & 0 & 0 & 0 & 0 \\ 0 & 0 & 0 & 0 & 0 & 0 \\ 0 & 0 & 0 & 0 & 0 & 1 \\ 0 & 0 & 0 & 0 & 0 & 0 \\ -\frac{2 \varepsilon pl^2 p2}{\varepsilon^2 pl p2 + 4} & \frac{4 pl p2}{\varepsilon^2 pl p2 + 4} & 0 & 0 & 0 & 0 \\ 0 & 0 & 0 & 0 & 0 & 0 \end{bmatrix}
\end{aligned}
\tag{2.5}$$

$$\begin{bmatrix} 0 & 0 & 0 & 0 & 0 & 0 \\ 0 & 0 & 0 & 0 & 0 & 0 \\ 0 & 0 & 0 & 0 & 0 & 0 \\ 0 & 0 & 0 & 0 & 0 & 1 \\ -\frac{4 p_1 p_2}{\epsilon^2 p_1 p_2 + 4} & -\frac{2 \epsilon p_2^2 p_1}{\epsilon^2 p_1 p_2 + 4} & 0 & 0 & 0 & 0 \\ 0 & 0 & 0 & 0 & 0 & 0 \end{bmatrix}, \begin{bmatrix} 0 & 0 & 0 & 0 & 0 & 0 \\ 0 & 0 & 0 & 0 & 0 & 0 \\ 0 & 0 & 0 & 0 & 0 & 0 \\ 0 & 0 & 0 & 0 & 0 & 0 \\ 0 & 0 & 0 & 0 & 0 & 1 \\ 0 & 0 & 0 & 0 & 0 & 0 \end{bmatrix}$$

$\triangleright R := \text{add}(r || u \cdot \text{deri}[u], u = 1 \dots \text{nops}(\text{deri}));$

$$R := \begin{bmatrix} r_1, r_2, r_3, 0, 0, r_4 \\ -\frac{r_2 p_1}{p_2}, r_1, 0, r_3, 0, r_5 \\ r_6, 0, r_7, r_2, 0, r_8 \\ 0, r_6, -\frac{r_2 p_1}{p_2}, r_7, 0, r_9 \\ -\frac{2 r_8 \epsilon p_1^2 p_2}{\epsilon^2 p_1 p_2 + 4} - \frac{4 r_9 p_1 p_2}{\epsilon^2 p_1 p_2 + 4}, \frac{4 r_8 p_1 p_2}{\epsilon^2 p_1 p_2 + 4} - \frac{2 r_9 \epsilon p_2^2 p_1}{\epsilon^2 p_1 p_2 + 4}, \frac{2 r_4 \epsilon p_1^2 p_2}{\epsilon^2 p_1 p_2 + 4} \\ + \frac{4 r_5 p_1 p_2}{\epsilon^2 p_1 p_2 + 4}, -\frac{4 r_4 p_1 p_2}{\epsilon^2 p_1 p_2 + 4} + \frac{2 r_5 \epsilon p_2^2 p_1}{\epsilon^2 p_1 p_2 + 4}, r_1 + r_7, r_{10} \\ 0, 0, 0, 0, 0, 0 \end{bmatrix} \quad (2.6)$$

$\triangleright \text{com} := R J - J R :$

$\triangleright \text{eq} := \{\text{seq}(\text{seq}(\text{com}[u, o], u = 1 \dots 6), o = 1 \dots 6)\};$

$$\text{eq} := \left\{ 0, r_{10}, r_4, r_5, r_8, r_9, -r_{10}, -2 r_2 r, -\frac{2 r_2 p_1 r}{p_2}, -r_1 - r_7, -r r_4 + \frac{(r^2 + 1) r_5}{t}, -r r_8 \right. \quad (2.7)$$

$$+ \frac{(r^2 + 1) r_9}{t}, r_2 t - \frac{r_2 p_1 (r^2 + 1)}{p_2 t}, \left( \frac{2 r_4 \epsilon p_1^2 p_2}{\epsilon^2 p_1 p_2 + 4} + \frac{4 r_5 p_1 p_2}{\epsilon^2 p_1 p_2 + 4} \right) r + \left( \right.$$

$$\left. -\frac{4 r_4 p_1 p_2}{\epsilon^2 p_1 p_2 + 4} + \frac{2 r_5 \epsilon p_2^2 p_1}{\epsilon^2 p_1 p_2 + 4} \right) t, \left( -\frac{2 r_8 \epsilon p_1^2 p_2}{\epsilon^2 p_1 p_2 + 4} - \frac{4 r_9 p_1 p_2}{\epsilon^2 p_1 p_2 + 4} \right) r$$

$$\begin{aligned}
& + \left( \frac{4 r 8 p l p 2}{\epsilon^2 p l p 2 + 4} - \frac{2 r 9 \epsilon p 2^2 p l}{\epsilon^2 p l p 2 + 4} \right) t, - \frac{\left( \frac{2 r 4 \epsilon p l^2 p 2}{\epsilon^2 p l p 2 + 4} + \frac{4 r 5 p l p 2}{\epsilon^2 p l p 2 + 4} \right) (r^2 + 1)}{t} \\
& - \left( - \frac{4 r 4 p l p 2}{\epsilon^2 p l p 2 + 4} + \frac{2 r 5 \epsilon p 2^2 p l}{\epsilon^2 p l p 2 + 4} \right) r, \\
& - \frac{\left( - \frac{2 r 8 \epsilon p l^2 p 2}{\epsilon^2 p l p 2 + 4} - \frac{4 r 9 p l p 2}{\epsilon^2 p l p 2 + 4} \right) (r^2 + 1)}{t} - \left( \frac{4 r 8 p l p 2}{\epsilon^2 p l p 2 + 4} \right. \\
& \left. - \frac{2 r 9 \epsilon p 2^2 p l}{\epsilon^2 p l p 2 + 4} \right) r, \frac{4 r 4 p l p 2}{\epsilon^2 p l p 2 + 4} - \frac{2 r 5 \epsilon p 2^2 p l}{\epsilon^2 p l p 2 + 4}, - \frac{4 r 8 p l p 2}{\epsilon^2 p l p 2 + 4} + \frac{2 r 9 \epsilon p 2^2 p l}{\epsilon^2 p l p 2 + 4}, \\
& \frac{r 2 p l (r^2 + 1)}{p 2 t} - r 2 t, - \frac{2 r 4 \epsilon p l^2 p 2}{\epsilon^2 p l p 2 + 4} - \frac{4 r 5 p l p 2}{\epsilon^2 p l p 2 + 4}, \frac{2 r 8 \epsilon p l^2 p 2}{\epsilon^2 p l p 2 + 4} \\
& + \frac{4 r 9 p l p 2}{\epsilon^2 p l p 2 + 4}, r r 5 - r 4 t, r r 9 - r 8 t \}
\end{aligned}$$

> *derisol* := solve(*eq*, {seq(*r*||*u*, *u* = 1 ..nops(*deri*)), *p1*, *p2*, *r*, *t*, *ε*});

*derisol* := {*ε* = *ε*, *p1* = *p1*, *p2* = *p2*, *r* = 0, *r1* = -*r7*, *r10* = 0, *r2* = *r2*, *r3* = *r3*, *r4* = 0, *r5* = 0, *r6* = *r6*, *r7* = *r7*, *r8* = 0, *r9* = 0, *t* = RootOf(*Z*<sup>2</sup> *p2* - *p1*)}, {*ε* = *ε*, *p1* = *p1*, *p2* = *p2*, *r* = *r*, *r1* = -*r7*, *r10* = 0, *r2* = 0, *r3* = *r3*, *r4* = 0, *r5* = 0, *r6* = *r6*, *r7* = *r7*, *r8* = 0, *r9* = 0, *t* = *t*}

> subs(*derisol*[1], *R*);

$$\begin{bmatrix}
-r7 & r2 & r3 & 0 & 0 & 0 \\
-\frac{r2 p l}{p2} & -r7 & 0 & r3 & 0 & 0 \\
r6 & 0 & r7 & r2 & 0 & 0 \\
0 & r6 & -\frac{r2 p l}{p2} & r7 & 0 & 0 \\
0 & 0 & 0 & 0 & 0 & 0 \\
0 & 0 & 0 & 0 & 0 & 0
\end{bmatrix}$$

> subs(*derisol*[2], *R*);

(2.10)



$$\begin{bmatrix} -r7 & 0 & r3 & 0 & 0 & 0 \\ 0 & -r7 & 0 & r3 & 0 & 0 \\ r6 & 0 & r7 & 0 & 0 & 0 \\ 0 & r6 & 0 & r7 & 0 & 0 \\ 0 & 0 & 0 & 0 & 0 & 0 \\ 0 & 0 & 0 & 0 & 0 & 0 \end{bmatrix} \quad (2.10)$$

Conclusion: for A3.1 the Symmetry algebra of the model is 3+6=9 dimensional, as expected.

### Section A3.2: isotropy $su(1,1)$ , rep $W+C$ . For $r \neq 0$

> restart : with(DifferentialGeometry) : with(LieAlgebras) : with(Tensor) : with(Tools) :  
with(ListTools) :

> StructureEquations :=  $\left[ \begin{aligned} &[x, ix] = p \cdot e, [x, y] = -p \cdot e, [ix, iy] = -p \cdot e, [y, iy] = p \cdot e, [x, e] = r \cdot (ix \\ &+ y), [ix, e] = r \cdot (-x + iy), [y, e] = r \cdot (x - iy), [iy, e] = r \cdot (ix + y), [x, ie] = \epsilon \cdot x - \frac{\epsilon}{2} \\ &\cdot iy, [ix, ie] = \epsilon \cdot ix + \frac{\epsilon}{2} \cdot y, [y, ie] = \epsilon \cdot y + \frac{\epsilon}{2} \cdot ix, [iy, ie] = \epsilon \cdot iy - \frac{\epsilon}{2} \cdot x, [e, ie] = \epsilon \cdot e \end{aligned} \right]$   
, [x, ix, y, iy, e, ie] :

> L1 := LieAlgebraData(StructureEquations, VC);

$$L1 := \left[ \begin{aligned} &[e1, e2] = p \cdot e5, [e1, e3] = -p \cdot e5, [e1, e5] = e2 \cdot r + e3 \cdot r, [e1, e6] = -\frac{1}{2} \epsilon \cdot e4 + \epsilon \cdot e1, \\ &[e2, e4] = -p \cdot e5, [e2, e5] = -e1 \cdot r + e4 \cdot r, [e2, e6] = \frac{1}{2} \epsilon \cdot e3 + \epsilon \cdot e2, [e3, e4] = p \cdot e5, [e3, \\ &e5] = e1 \cdot r - e4 \cdot r, [e3, e6] = \epsilon \cdot e3 + \frac{1}{2} \epsilon \cdot e2, [e4, e5] = e2 \cdot r + e3 \cdot r, [e4, e6] = \epsilon \cdot e4 \\ &- \frac{1}{2} \epsilon \cdot e1, [e5, e6] = \epsilon \cdot e5 \end{aligned} \right] \quad (3.1)$$

> DGsetup(L1, [e], [f]) :

> Query({p, r, ε}, "Jacobi");

$$\begin{aligned} &true, \{0\}, \left\{ \left\{ \epsilon = \epsilon, p = p, r = r \right\} \right\}, \left[ \left[ \begin{aligned} &[e1, e2] = p \cdot e5, [e1, e3] = -p \cdot e5, [e1, e5] = e2 \cdot r + e3 \cdot r, \\ &[e1, e6] = -\frac{1}{2} \epsilon \cdot e4 + \epsilon \cdot e1, [e2, e4] = -p \cdot e5, [e2, e5] = -e1 \cdot r + e4 \cdot r, [e2, e6] = \frac{1}{2} \epsilon \cdot e3 \\ &+ \epsilon \cdot e2, [e3, e4] = p \cdot e5, [e3, e5] = e1 \cdot r - e4 \cdot r, [e3, e6] = \epsilon \cdot e3 + \frac{1}{2} \epsilon \cdot e2, [e4, e5] = e2 \cdot r \\ &+ e3 \cdot r, [e4, e6] = \epsilon \cdot e4 - \frac{1}{2} \epsilon \cdot e1, [e5, e6] = \epsilon \cdot e5 \end{aligned} \right] \right] \end{aligned} \quad (3.2)$$

> LD := LeviDecomposition( )

$$LD := [[e1, e2, e3, e4, e5, e6], [ ]] \quad (3.3)$$

>

We shall exclude the possibility that  $p=0$ . We also have  $\varepsilon=0 \vee \varepsilon=1$ .

>

>  $J := \text{Matrix}([ [0, -((1 + s^2 + t^2)/(2t)), -((1 + s^2 - t^2)/(2t)), -s, 0, 0], [ (1 + s^2 + t^2)/(2t), 0, s, -((1 + s^2 - t^2)/(2t)), 0, 0], [ -((1 + s^2 - t^2)/(2t)), s, 0, (1 + s^2 + t^2)/(2t), 0, 0], [ -s, -((1 + s^2 - t^2)/(2t)), -((1 + s^2 + t^2)/(2t)), 0, 0, 0], [0, 0, 0, 0, 0, -1], [0, 0, 0, 0, 1, 0]]);$

$$J := \begin{bmatrix} 0 & -\frac{1}{2} \frac{s^2 + t^2 + 1}{t} & -\frac{1}{2} \frac{s^2 - t^2 + 1}{t} & -s & 0 & 0 \\ \frac{1}{2} \frac{s^2 + t^2 + 1}{t} & 0 & s & -\frac{1}{2} \frac{s^2 - t^2 + 1}{t} & 0 & 0 \\ -\frac{1}{2} \frac{s^2 - t^2 + 1}{t} & s & 0 & \frac{1}{2} \frac{s^2 + t^2 + 1}{t} & 0 & 0 \\ -s & -\frac{1}{2} \frac{s^2 - t^2 + 1}{t} & -\frac{1}{2} \frac{s^2 + t^2 + 1}{t} & 0 & 0 & 0 \\ 0 & 0 & 0 & 0 & 0 & -1 \\ 0 & 0 & 0 & 0 & 1 & 0 \end{bmatrix} \quad (3.4)$$

>  $\text{deri} := \text{Derivations}(\text{"Full"});$

$$\text{deri} := \begin{bmatrix} \begin{bmatrix} 1 & 0 & 0 & 0 & 0 & 0 \\ 0 & 1 & 1 & 0 & 0 & 0 \\ 0 & 1 & 1 & 0 & 0 & 0 \\ 0 & 0 & 0 & 1 & 0 & 0 \\ 0 & 0 & 0 & 0 & 1 & 0 \\ 0 & 0 & 0 & 0 & 0 & 0 \end{bmatrix} \begin{bmatrix} 0 & 1 & 0 & 0 & 0 & 0 \\ -1 & 0 & 0 & 0 & 0 & 0 \\ 0 & 0 & 0 & 1 & 0 & 0 \\ 0 & 0 & -1 & 0 & 0 & 0 \\ 0 & 0 & 0 & 0 & 0 & 0 \\ 0 & 0 & 0 & 0 & 0 & 0 \end{bmatrix} \begin{bmatrix} 0 & 0 & 1 & 0 & 0 & 0 \\ 0 & 0 & 0 & 0 & 0 & 0 \\ 1 & 0 & 0 & 1 & 0 & 0 \\ 0 & 0 & -1 & 0 & 0 & 0 \\ 0 & 0 & 0 & 0 & 0 & -\frac{1}{2} \frac{\varepsilon}{r} \\ 0 & 0 & 0 & 0 & 0 & 0 \end{bmatrix} \end{bmatrix}, \quad (3.5)$$

$$\begin{bmatrix} \begin{bmatrix} 0 & 0 & 0 & 1 & 0 & 0 \\ 0 & 0 & 1 & 0 & 0 & 0 \\ 0 & 1 & 0 & 0 & 0 & 0 \\ 1 & 0 & 0 & 0 & 0 & 0 \\ 0 & 0 & 0 & 0 & 0 & 0 \\ 0 & 0 & 0 & 0 & 0 & 0 \end{bmatrix} \begin{bmatrix} 0 & 0 & 0 & 0 & 1 & 0 \\ 0 & 0 & 0 & 0 & 0 & 0 \\ 0 & 0 & 0 & 0 & 0 & \frac{1}{2} \frac{\varepsilon}{r} \\ 0 & 0 & 0 & 0 & -1 & 0 \\ \frac{p}{r} & 0 & 0 & \frac{p}{r} & 0 & 0 \\ 0 & 0 & 0 & 0 & 0 & 0 \end{bmatrix} \begin{bmatrix} 0 & 0 & 0 & 0 & 0 & 1 \\ 0 & 0 & 0 & 0 & 0 & 0 \\ 0 & 0 & 0 & 0 & 0 & 0 \\ 0 & 0 & 0 & 0 & 0 & -1 \\ 0 & 0 & 0 & 0 & 0 & 0 \\ 0 & 0 & 0 & 0 & 0 & 0 \end{bmatrix} \end{bmatrix},$$

$$\begin{bmatrix} 0 & 0 & 0 & 0 & 0 & 0 \\ 0 & 0 & 0 & 1 & 0 & 0 \\ 0 & 0 & 0 & 1 & 0 & 0 \\ 0 & 1 & -1 & 0 & 0 & 0 \\ 0 & 0 & 0 & 0 & 0 & -\frac{1}{2} \frac{\epsilon}{r} \\ 0 & 0 & 0 & 0 & 0 & 0 \end{bmatrix}, \begin{bmatrix} 0 & 0 & 0 & 0 & 0 & 0 \\ 0 & 0 & 0 & 0 & 1 & 0 \\ 0 & 0 & 0 & 0 & 1 & 0 \\ 0 & 0 & 0 & 0 & 0 & \frac{1}{2} \frac{\epsilon}{r} \\ 0 & \frac{p}{r} & -\frac{p}{r} & 0 & 0 & 0 \\ 0 & 0 & 0 & 0 & 0 & 0 \end{bmatrix}, \begin{bmatrix} 0 & 0 & 0 & 0 & 0 & 0 \\ 0 & 0 & 0 & 0 & 0 & 1 \\ 0 & 0 & 0 & 0 & 0 & 1 \\ 0 & 0 & 0 & 0 & 0 & 1 \\ 0 & 0 & 0 & 0 & 0 & 0 \\ 0 & 0 & 0 & 0 & 0 & 0 \end{bmatrix}$$

>  $R := \text{add}(r||u \cdot \text{deri}[u], u = 1 \dots \text{nops}(\text{deri}))$ ;

$$R := \begin{bmatrix} r1 & r2 & r3 & r4 & r5 & r6 \\ -r2 & r1 & r1 + r4 & r7 & r8 & r9 \\ r3 & r1 + r4 & r1 & r2 + r3 + r7 & r8 & \frac{1}{2} \frac{r5 \epsilon}{r} + r9 \\ r4 & r7 & -r2 - r3 - r7 & r1 & -r5 & -r6 + \frac{1}{2} \frac{r8 \epsilon}{r} \\ \frac{r5 p}{r} & \frac{r8 p}{r} & -\frac{r8 p}{r} & \frac{r5 p}{r} & r1 & -\frac{1}{2} \frac{r3 \epsilon}{r} - \frac{1}{2} \frac{r7 \epsilon}{r} \\ 0 & 0 & 0 & 0 & 0 & 0 \end{bmatrix} \quad (3.6)$$

>  $\text{com} := R.J - J.R$ ;

>  $\text{eq} := \{\text{seq}(\text{seq}(\text{com}[u, o], u = 1 \dots 6), o = 1 \dots 6)\}$ ;

>  $\text{derisol} := [\text{solve}(\text{eq}, \{\text{seq}(r||u, u = 1 \dots \text{nops}(\text{deri})), p, r, t, \epsilon, s\})]$ ;

$$\begin{aligned} \text{derisol} := & \left[ \left\{ \epsilon = -\frac{4 r (s^2 + 1)}{t}, p = 0, r = r, r1 = 0, r2 = r2, r3 = -r7, r4 = r4, r5 = r5, r6 \right. \right. \\ & = \frac{r5 s t - r8 s^2 - r8}{t}, r7 = r7, r8 = r8, r9 = \frac{r5 s^2 + r8 s t + r5}{t}, s = s, t = t \left. \right\}, \left\{ \epsilon = \epsilon, p = p, \right. \\ & \left. \left. r = r, r1 = 0, r2 = r2, r3 = -r7, r4 = r4, r5 = 0, r6 = 0, r7 = r7, r8 = 0, r9 = 0, s = s, t = t \right\} \right] \end{aligned} \quad (3.7)$$

>  $\text{subs}(\text{derisol}[1], R)$ ;

(3.8)

$$\begin{bmatrix}
0 & r2 & -r7 & r4 & r5 & \frac{r5 s t - r8 s^2 - r8}{t} \\
-r2 & 0 & r4 & r7 & r8 & \frac{r5 s^2 + r8 s t + r5}{t} \\
-r7 & r4 & 0 & r2 & r8 & -\frac{2 r5 (s^2 + 1)}{t} + \frac{r5 s^2 + r8 s t + r5}{t} \\
r4 & r7 & -r2 & 0 & -r5 & -\frac{r5 s t - r8 s^2 - r8}{t} - \frac{2 r8 (s^2 + 1)}{t} \\
0 & 0 & 0 & 0 & 0 & 0 \\
0 & 0 & 0 & 0 & 0 & 0
\end{bmatrix} \quad (3.8)$$

> subs(derisol[2], R);

$$\begin{bmatrix}
0 & r2 & -r7 & r4 & 0 & 0 \\
-r2 & 0 & r4 & r7 & 0 & 0 \\
-r7 & r4 & 0 & r2 & 0 & 0 \\
r4 & r7 & -r2 & 0 & 0 & 0 \\
0 & 0 & 0 & 0 & 0 & 0 \\
0 & 0 & 0 & 0 & 0 & 0
\end{bmatrix} \quad (3.9)$$

> The first solution requires  $p=0$  which is excluded as it isn't NDG.

> Conclusion: for A3.2 the Symmetry algebra of the model is  $3+6=9$  dimensional, as expected.

### Section A3.2: isotropy $su(1,1)$ , rep $W+C$ . For $r=0$

> restart : with(DifferentialGeometry) : with(LieAlgebras) : with(Tensor) : with(Tools) :  
with(ListTools) :

> StructureEquations := [[x, ix]=p·e, [x, y]=-p·e, [ix, iy]=-p·e, [y, iy]=p·e, [x, ie]=s·x  
+ ((ε - 2·s)/2)·iy, [ix, ie]=s·ix - ((ε - 2·s)/2)·y, [y, ie]=s·y - ((ε - 2·s)/2)·ix, [iy, ie]=s·iy + ((ε - 2·s)/2)·x, [e, ie]=ε·e], [x, ix, y, iy, e, ie] :

> L1 := LieAlgebraData(StructureEquations, VC);

$$\begin{aligned}
L1 := & \left[ [e1, e2] = p e5, [e1, e3] = -p e5, [e1, e6] = \left( \frac{1}{2} \varepsilon - s \right) e4 + s e1, [e2, e4] = -p e5, \right. \\
& [e2, e6] = \left( -\frac{1}{2} \varepsilon + s \right) e3 + s e2, [e3, e4] = p e5, [e3, e6] = s e3 + \left( -\frac{1}{2} \varepsilon + s \right) e2, \\
& \left. [e4, e6] = s e4 + \left( \frac{1}{2} \varepsilon - s \right) e1, [e5, e6] = \varepsilon e5 \right] \quad (4.1)
\end{aligned}$$

> DGsetup(L1, [e], [f]) :

> Query({p, l, s}, "Jacobi");

(4.2)

$$\begin{aligned}
& \text{true}, \{0\}, [\{l=l, p=p, s=s\}], \left[ \left[ [e1, e2]=p e5, [e1, e3]=-p e5, [e1, e6]=\left(\frac{1}{2} \varepsilon - s\right) e4 \right. \right. \\
& \quad \left. \left. + s e1, [e2, e4]=-p e5, [e2, e6]=\left(-\frac{1}{2} \varepsilon + s\right) e3 + s e2, [e3, e4]=p e5, [e3, e6] \right. \right. \\
& \quad \left. \left. =s e3 + \left(-\frac{1}{2} \varepsilon + s\right) e2, [e4, e6]=s e4 + \left(\frac{1}{2} \varepsilon - s\right) e1, [e5, e6]=\varepsilon e5 \right] \right]
\end{aligned} \quad (4.2)$$

$$\begin{aligned}
& > LD := \text{LeviDecomposition}() \\
& \quad \quad \quad LD := [[e1, e2, e3, e4, e5, e6], []]
\end{aligned} \quad (4.3)$$

*We shall exclude the possibility that  $p=0$ . We also have  $\varepsilon=0 \vee \varepsilon=1$ .*

$$\begin{aligned}
& > J := \text{Matrix}([ [0, -((1 + r^2 + t^2)/(2t)), -((1 + r^2 - t^2)/(2t)), -r, 0, 0], [ ( \\
& \quad 1 + r^2 + t^2)/(2t), 0, r, -((1 + r^2 - t^2)/(2t)), 0, 0], [ -((1 + r^2 - t^2)/(2t)), r, 0, (1 + r^2 + t^2)/(2t), 0, 0], [ -r, -((1 + r^2 - t^2)/(2t)), -((1 + r^2 + t \\
& \quad ^2)/(2t)), 0, 0, 0], [0, 0, 0, 0, 0, -1], [0, 0, 0, 0, 1, 0]]);
\end{aligned}$$

$$J := \begin{bmatrix} 0 & -\frac{1}{2} \frac{r^2 + t^2 + 1}{t} & -\frac{1}{2} \frac{r^2 - t^2 + 1}{t} & -r & 0 & 0 \\ \frac{1}{2} \frac{r^2 + t^2 + 1}{t} & 0 & r & -\frac{1}{2} \frac{r^2 - t^2 + 1}{t} & 0 & 0 \\ -\frac{1}{2} \frac{r^2 - t^2 + 1}{t} & r & 0 & \frac{1}{2} \frac{r^2 + t^2 + 1}{t} & 0 & 0 \\ -r & -\frac{1}{2} \frac{r^2 - t^2 + 1}{t} & -\frac{1}{2} \frac{r^2 + t^2 + 1}{t} & 0 & 0 & 0 \\ 0 & 0 & 0 & 0 & 0 & -1 \\ 0 & 0 & 0 & 0 & 1 & 0 \end{bmatrix} \quad (4.4)$$

$$> \text{deri} := \text{Derivations}(\text{"Full"});$$

$$\text{deri} := \begin{bmatrix} \begin{bmatrix} 1 & 0 & 0 & 0 & 0 & 0 \\ 0 & 0 & 0 & 0 & 0 & 0 \\ 0 & 0 & 0 & 0 & 0 & 0 \\ 0 & 0 & 0 & 1 & 0 & 0 \\ 0 & 0 & 0 & 0 & 1 & 0 \\ 0 & 0 & 0 & 0 & 0 & 0 \end{bmatrix}, \begin{bmatrix} 0 & 1 & 0 & 0 & 0 & 0 \\ 0 & 0 & 0 & 0 & 0 & 0 \\ 0 & 0 & 0 & 0 & 0 & 0 \\ 0 & 0 & -1 & 0 & 0 & 0 \\ 0 & 0 & 0 & 0 & 0 & 0 \\ 0 & 0 & 0 & 0 & 0 & 0 \end{bmatrix}, \begin{bmatrix} 0 & 0 & 1 & 0 & 0 & 0 \\ 0 & 0 & 0 & 0 & 0 & 0 \\ 0 & 0 & 0 & 0 & 0 & 0 \\ 0 & -1 & 0 & 0 & 0 & 0 \\ 0 & 0 & 0 & 0 & 0 & 0 \\ 0 & 0 & 0 & 0 & 0 & 0 \end{bmatrix} \end{bmatrix}, \quad (4.5)$$

$$\begin{bmatrix} 0 & 0 & 0 & 1 & 0 & 0 \\ 0 & 0 & 0 & 0 & 0 & 0 \\ 0 & 0 & 0 & 0 & 0 & 0 \\ 1 & 0 & 0 & 0 & 0 & 0 \\ 0 & 0 & 0 & 0 & 1 & 0 \\ 0 & 0 & 0 & 0 & 0 & 0 \end{bmatrix}, \begin{bmatrix} 0 & 0 & 0 & 0 & 0 & 1 \\ 0 & 0 & 0 & 0 & 0 & 0 \\ 0 & 0 & 0 & 0 & 0 & 0 \\ 0 & 0 & 0 & 0 & 0 & 0 \\ 0 & \frac{p}{l+s} & -\frac{p}{l+s} & 0 & 0 & 0 \\ 0 & 0 & 0 & 0 & 0 & 0 \end{bmatrix}, \begin{bmatrix} 0 & 0 & 0 & 0 & 0 & 0 \\ 1 & 0 & 0 & 0 & 0 & 0 \\ 0 & 0 & 0 & -1 & 0 & 0 \\ 0 & 0 & 0 & 0 & 0 & 0 \\ 0 & 0 & 0 & 0 & 0 & 0 \\ 0 & 0 & 0 & 0 & 0 & 0 \end{bmatrix},$$

$$\begin{bmatrix} 0 & 0 & 0 & 0 & 0 & 0 \\ 0 & 1 & 0 & 0 & 0 & 0 \\ 0 & 0 & 1 & 0 & 0 & 0 \\ 0 & 0 & 0 & 0 & 0 & 0 \\ 0 & 0 & 0 & 0 & 1 & 0 \\ 0 & 0 & 0 & 0 & 0 & 0 \end{bmatrix}, \begin{bmatrix} 0 & 0 & 0 & 0 & 0 & 0 \\ 0 & 0 & 1 & 0 & 0 & 0 \\ 0 & 1 & 0 & 0 & 0 & 0 \\ 0 & 0 & 0 & 0 & 0 & 0 \\ 0 & 0 & 0 & 0 & -1 & 0 \\ 0 & 0 & 0 & 0 & 0 & 0 \end{bmatrix}, \begin{bmatrix} 0 & 0 & 0 & 0 & 0 & 0 \\ 0 & 0 & 0 & 1 & 0 & 0 \\ -1 & 0 & 0 & 0 & 0 & 0 \\ 0 & 0 & 0 & 0 & 0 & 0 \\ 0 & 0 & 0 & 0 & 0 & 0 \\ 0 & 0 & 0 & 0 & 0 & 0 \end{bmatrix},$$

$$\begin{bmatrix} 0 & 0 & 0 & 0 & 0 & 0 \\ 0 & 0 & 0 & 0 & 0 & 1 \\ 0 & 0 & 0 & 0 & 0 & 0 \\ 0 & 0 & 0 & 0 & 0 & 0 \\ -\frac{p}{l+s} & 0 & 0 & -\frac{p}{l+s} & 0 & 0 \\ 0 & 0 & 0 & 0 & 0 & 0 \end{bmatrix}, \begin{bmatrix} 0 & 0 & 0 & 0 & 0 & 0 \\ 0 & 0 & 0 & 0 & 0 & 0 \\ 0 & 0 & 0 & 0 & 0 & 1 \\ 0 & 0 & 0 & 0 & 0 & 0 \\ \frac{p}{l+s} & 0 & 0 & \frac{p}{l+s} & 0 & 0 \\ 0 & 0 & 0 & 0 & 0 & 0 \end{bmatrix},$$

$$\begin{bmatrix} 0 & 0 & 0 & 0 & 0 & 0 \\ 0 & 0 & 0 & 0 & 0 & 0 \\ 0 & 0 & 0 & 0 & 0 & 0 \\ 0 & 0 & 0 & 0 & 0 & 1 \\ 0 & \frac{p}{l+s} & -\frac{p}{l+s} & 0 & 0 & 0 \\ 0 & 0 & 0 & 0 & 0 & 0 \end{bmatrix}, \begin{bmatrix} 0 & 0 & 0 & 0 & 0 & 0 \\ 0 & 0 & 0 & 0 & 0 & 0 \\ 0 & 0 & 0 & 0 & 0 & 0 \\ 0 & 0 & 0 & 0 & 0 & 0 \\ 0 & 0 & 0 & 0 & 0 & 1 \\ 0 & 0 & 0 & 0 & 0 & 0 \end{bmatrix}$$

$\triangleright R := \text{add}(r||u \cdot \text{deri}[u], u = 1 \dots \text{nops}(\text{deri}));$

$$R := \begin{bmatrix} r1, r2, r3, r4, 0, r5 \end{bmatrix},$$

$$\begin{bmatrix} r6, r7, r8, r9, 0, r10 \end{bmatrix},$$

$$\begin{bmatrix} -r9, r8, r7, -r6, 0, r11 \end{bmatrix},$$

(4.6)

$$\begin{aligned} & \left[ r4, -r3, -r2, r1, 0, r12 \right], \\ & \left[ -\frac{r10p}{l+s} + \frac{r11p}{l+s}, \frac{r5p}{l+s} + \frac{r12p}{l+s}, -\frac{r5p}{l+s} - \frac{r12p}{l+s}, -\frac{r10p}{l+s} + \frac{r11p}{l+s}, r1 + r4 \right. \\ & \quad \left. + r7 - r8, r13 \right], \\ & \left[ 0, 0, 0, 0, 0, 0 \right] \end{aligned}$$

>  $com := R.J - J.R :$

>  $eq := \{seq(seq(com[u, o], u = 1 .. 6), o = 1 .. 6) \} :$

>  $derisol := [solve(eq, \{seq(r||u, u = 1 .. nops(deri)), p, r, t, s, l\})];$

$derisol := [ \{ \epsilon = \epsilon, l = l, p = p, r = r, r1 = 0, r10 = 0, r11 = 0, r12 = 0, r13 = 0, r2 = -r6, r3 = -r9, r4 = r8, r5 = 0, r6 = r6, r7 = 0, r8 = r8, r9 = r9, s = s, t = t \} ]$  (4.7)

>  $subs(derisol[1], R);$

$$\begin{bmatrix} 0 & -r6 & -r9 & r8 & 0 & 0 \\ r6 & 0 & r8 & r9 & 0 & 0 \\ -r9 & r8 & 0 & -r6 & 0 & 0 \\ r8 & r9 & r6 & 0 & 0 & 0 \\ 0 & 0 & 0 & 0 & 0 & 0 \\ 0 & 0 & 0 & 0 & 0 & 0 \end{bmatrix}$$

(4.8)

>

> *Conclusion: for A3.2 the Symmetry algebra of the model is 3+6=9 dimensional, as expected.*

>
