# Supplementary material for: Homogeneous almost complex structures in dimension 6 with semi-simple isotropy
Source: arXiv:1401.8187 ancillary file (2014-02-12)
Supplement: Supplementary file 2 [file GH-Unified.pdf]

## Gray

### –Hervella types of 6 D homogeneous almost Hermitian structures with semisimple isotropy

We investigate which of the sixteen classes of almost Hermitian structures are realized on our 6D homogeneous spaces. It is easy to see by inspecting our tables that strict type W2 is not realized, so this is skipped. For details about the classes, see the paper by Gray and Hervella. All 6D Lie algebras and their left invariant Hermitian structures in this document have additional  $\mathfrak{su}(2)$ -symmetry, such that the dimensions of the symmetry algebras of these structures are at least 9.

#### ▼ A1.1

```
> restart : with(DifferentialGeometry) : with(LieAlgebras) : with(Tensor) : with(Tools) :
with(LinearAlgebra) :
```

```
> StructureEquations := [ [ee, ii] = α * e, [jj, kk] = -α * e, [ee, ie] =  $\frac{\epsilon}{2}$  * ee + r * ii, [ii, ie] =  $\frac{\epsilon}{2}$ 
* ii - r * ee, [jj, ie] =  $\frac{\epsilon}{2}$  * jj - r * kk, [kk, ie] =  $\frac{\epsilon}{2}$  * kk + r * jj, [e, ie] = ε * e ], [ee, ii, jj,
kk, e, ie] :
```

```
L := LieAlgebraData(StructureEquations, VC);
```

```
L := [ [e1, e2] = α e5, [e1, e6] = r e2 +  $\frac{1}{2}$  ε e1, [e2, e6] =  $\frac{1}{2}$  ε e2 - r e1, [e3, e4] = -α e5, (1.1)
[e3, e6] = -r e4 +  $\frac{1}{2}$  ε e3, [e4, e6] =  $\frac{1}{2}$  ε e4 + r e3, [e5, e6] = ε e5 ]
```

```
> DGsetup(L, [e], [f]) :
```

```
> g := evalDG((f1 &t f1 + f2 &t f2 + f3 &t f3 + f4 &t f4) + t*(f5 &t f5 + f6 &t f6));
g := f1 f1 + f2 f2 + f3 f3 + f4 f4 + t f5 f5 + t f6 f6 (1.2)
```

```
> J0 := Matrix([ [0, -cos(a) sin(b), -sin(a) sin(b), -cos(b), 0, 0], [cos(a) sin(b), 0,
cos(b), -sin(a) sin(b), 0, 0], [sin(a) sin(b), -cos(b), 0, cos(a) sin(b), 0, 0],
cos(a) sin(b), 0, 0], [cos(b), sin(a) sin(b), -cos(a) sin(b), 0, 0, 0], [0, 0, 0, 0, 0, -1],
[0, 0, 0, 0, 1, 0]]);
```

$$J0 := \begin{bmatrix} 0 & -\cos(a) \sin(b) & -\sin(a) \sin(b) & -\cos(b) & 0 & 0 \\ \cos(a) \sin(b) & 0 & \cos(b) & -\sin(a) \sin(b) & 0 & 0 \\ \sin(a) \sin(b) & -\cos(b) & 0 & \cos(a) \sin(b) & 0 & 0 \\ \cos(b) & \sin(a) \sin(b) & -\cos(a) \sin(b) & 0 & 0 & 0 \\ 0 & 0 & 0 & 0 & 0 & -1 \\ 0 & 0 & 0 & 0 & 1 & 0 \end{bmatrix} \quad (1.3)$$

```
> J := convert(J0, DGtensor, [ ["con_bas", "cov_bas"], [ ]]);
```

```
J := -cos(a) sin(b) e1 f2 - sin(a) sin(b) e1 f3 - cos(b) e1 f4 + cos(a) sin(b) e2 f1
+ cos(b) e2 f3 - sin(a) sin(b) e2 f4 + sin(a) sin(b) e3 f1 - cos(b) e3 f2
+ cos(a) sin(b) e3 f4 + cos(b) e4 f1 + sin(a) sin(b) e4 f2 - cos(a) sin(b) e4 f3 (1.4)
```

$$\begin{aligned}
& -e5 f6 + e6 f5 \\
> w := \text{ContractIndices}(J, g, [[1, 1]]); \\
w := & \cos(a) \sin(b) f1 f2 + \sin(a) \sin(b) f1 f3 + \cos(b) f1 f4 - \cos(a) \sin(b) f2 f1 \\
& - \cos(b) f2 f3 + \sin(a) \sin(b) f2 f4 - \sin(a) \sin(b) f3 f1 + \cos(b) f3 f2 \\
& - \cos(a) \sin(b) f3 f4 - \cos(b) f4 f1 - \sin(a) \sin(b) f4 f2 + \cos(a) \sin(b) f4 f3 \\
& + t f5 f6 - t f6 f5
\end{aligned} \tag{1.5}$$

$$\begin{aligned}
> W := \text{convert}(w, \text{DGform}); \\
W := & \cos(a) \sin(b) f1 \wedge f2 + \sin(a) \sin(b) f1 \wedge f3 + \cos(b) f1 \wedge f4 - \cos(b) f2 \wedge f3 \\
& + \sin(a) \sin(b) f2 \wedge f4 - \cos(a) \sin(b) f3 \wedge f4 + t f5 \wedge f6
\end{aligned} \tag{1.6}$$

$$\begin{aligned}
> \text{Nabla} := \text{Christoffel}(g); \\
> Nw := \text{RearrangeIndices}(\text{CovariantDerivative}(w, \text{Nabla}), [2, 3, 1]); \\
> NJ := \text{TensorBrackets}(J, J, \text{"Frolicher-Nijenhuis"}); \\
> \text{delta}W := \text{HodgeStar}(g, \text{ExteriorDerivative}(\text{HodgeStar}(g, W))) : \\
> Lee := \text{convert}\left(\text{evalDG}\left(-\frac{1}{2} \cdot \text{ContractIndices}(J, \text{HodgeStar}(g, \right. \right. \\
& \left. \left. \text{ExteriorDerivative}(\text{HodgeStar}(g, W))) , [[1, 1]]\right), \text{DGform}\right); \\
& Lee := (t \alpha \cos(a) \sin(b) - \varepsilon) f6
\end{aligned} \tag{1.7}$$

$$\begin{aligned}
> \text{part2} := \text{SymmetrizeIndices}(\text{evalDG}(g \&t \text{delta}W), [2, 3], \text{"SkewSymmetric"}); \\
> \text{part3} := \text{SymmetrizeIndices}(\text{RearrangeIndices}(\text{ContractIndices}(J, \\
& \text{ContractIndices}(\text{evalDG}(g \&t \text{delta}W), J, [[3, 1]]), [[1, 2]]), [2, 1, 3]), [2, 3], \\
& \text{"SkewSymmetric"}); \\
> \mu := \text{evalDG}\left(Nw + \frac{1}{2} \cdot (\text{part2} - \text{part3})\right);
\end{aligned}$$

**0**

$$\begin{aligned}
> \text{cond0} := \text{DGinfo}(Nw, \text{"CoefficientSet"}); \\
> \text{sol0} := \text{solve}(\{op(\text{cond0}), t \neq 0\}); \\
\text{sol0} := & \left\{a = a, \alpha = 0, b = b, \varepsilon = 0, r = 0, t = t\right\}, \left\{a = 0, \alpha = \alpha, b = \frac{1}{2} \pi, \varepsilon = t \alpha, r = r, t = t\right\}, \tag{1.1.1} \\
& \left\{a = 0, \alpha = \alpha, b = -\frac{1}{2} \pi, \varepsilon = -t \alpha, r = r, t = t\right\}, \left\{a = \pi, \alpha = \alpha, b = \frac{1}{2} \pi, \varepsilon = -t \alpha, r = r, t \right. \\
& \left. = t\right\}, \left\{a = \pi, \alpha = \alpha, b = -\frac{1}{2} \pi, \varepsilon = t \alpha, r = r, t = t\right\} \\
> \text{Neg0} := \text{add}(\text{cond0}[i]^2, i = 1 .. \text{nops}(\text{cond0}));
\end{aligned}$$

**W1**

$$\begin{aligned}
> \text{SNw} := \text{SymmetrizeIndices}(Nw, [1, 2, 3], \text{"SkewSymmetric"}); \\
> \text{condw1} := \text{DGinfo}(\text{evalDG}(Nw - \text{SNw}), \text{"CoefficientSet"}); \\
> \text{solve}(\{op(\text{condw1}), t \neq 0, \text{Neg0} \neq 0\}); \\
& \left\{a = 0, \alpha = 0, b = \frac{1}{2} \pi, \varepsilon = 0, r = r, t = t\right\}, \left\{a = 0, \alpha = 0, b = -\frac{1}{2} \pi, \varepsilon = 0, r = r, t = t\right\} \tag{1.2.1} \\
> \text{Negw1} := \text{add}(\text{condw1}[i]^2, i = 1 .. \text{nops}(\text{condw1}));
\end{aligned}$$

$$\left[ \begin{array}{l} \text{> } \text{simplify}\left(\text{subs}\left(\left\{a=0, b=\frac{1}{2}\pi, r=r, t=t, \alpha=0, \varepsilon=0\right\}, \text{Neg0}\right)\right); \\ \phantom{\text{> }} 0 \end{array} \right] \quad (1.2.2)$$

### W3

$$\left[ \begin{array}{l} \text{> } \text{condw3} := \{op(DGinfo(deltaW, "CoefficientSet")), op(DGinfo(NJ, \\ \phantom{\text{> }} "CoefficientSet"))\}; \\ \text{> } \text{solve}(\{op(condw3), t \neq 0, \text{Neg0} \neq 0\}) \\ \text{> } \text{Negw3} := \text{add}(condw3[i]^2, i = 1 .. nops(condw3)) : \end{array} \right]$$

### W4

$$\left[ \begin{array}{l} \text{> } \text{condw4} := DGinfo(mu, "CoefficientSet") : \\ \text{> } \text{solve}(\{op(condw4), t \neq 0, \text{Neg0} \neq 0\}); \\ \phantom{\text{> }} \left\{a=0, \alpha=0, b=\frac{1}{2}\pi, \varepsilon=0, r=r, t=t\right\}, \left\{a=0, \alpha=0, b=-\frac{1}{2}\pi, \varepsilon=0, r=r, t=t\right\} \\ \text{> } \text{Negw4} := \text{add}(condw4[i]^2, i = 1 .. nops(condw4)) : \end{array} \right] \quad (1.4.1)$$

### W1+W2

$$\left[ \begin{array}{l} \text{> } \text{condw12} := DGinfo(DG\text{simplify}(\text{simplify}(\text{evalDG}(\text{Nw} \\ \phantom{\text{> }} + \text{RearrangeIndices}(\text{ContractIndices}(J, \text{ContractIndices}(J, \text{Nw}, [[1, 1]]), [[1, \\ \phantom{\text{> }} 3]]), [3, 1, 2])))), "CoefficientSet") : \\ \text{> } \text{use RealDomain in solve}(\{op(condw12), t \neq 0, \text{Neg0} \neq 0, \text{Negw1} \neq 0, \text{Negw2} \neq 0\}) \\ \phantom{\text{> }} \text{end use} \\ \text{> } \text{Negw12} := \text{add}(condw12[i]^2, i = 1 .. nops(condw12)) : \end{array} \right]$$

### W1+W3

$$\left[ \begin{array}{l} \text{> } \text{condw13} := \{op(DGinfo(deltaW, "CoefficientSet")), \\ \phantom{\text{> }} op(DGinfo(\text{SymmetrizeIndices}(\text{evalDG}(\text{Nw} - \text{ContractIndices}(J, \\ \phantom{\text{> }} \text{RearrangeIndices}(\text{ContractIndices}(J, \text{Nw}, [[1, 3]]), [3, 1, 2]), [[1, 1]])), [1, 3], \\ \phantom{\text{> }} "Symmetric"), "CoefficientSet"))\}; \\ \text{> } \text{use RealDomain in solve}(\{op(condw13), t \neq 0, \text{Neg0} \neq 0, \text{Negw1} \neq 0, \text{Negw3} \neq 0\}) \\ \phantom{\text{> }} \text{end use}; \\ \text{> } \text{Negw13} := \text{add}(condw13[i]^2, i = 1 .. nops(condw13)) : \\ \text{> } \end{array} \right]$$

### W1+W4

$$\left[ \begin{array}{l} \text{> } \text{condw14} := DGinfo(\text{SymmetrizeIndices}(mu, [1, 2], "Symmetric"), "CoefficientSet") : \\ \text{> } \text{solve}(\{op(condw14), t \neq 0, \text{Neg0} \neq 0, \text{Negw1} \neq 0, \text{Negw4} \neq 0\}); \\ \phantom{\text{> }} \left\{a=0, \alpha=0, b=\frac{1}{2}\pi, \varepsilon=0, r=r, t=t\right\}, \left\{a=0, \alpha=0, b=-\frac{1}{2}\pi, \varepsilon=0, r=r, t=t\right\} \\ \text{> } \text{Negw14} := \text{add}(condw14[i]^2, i = 1 .. nops(condw14)) : \end{array} \right] \quad (1.7.1)$$

$$\text{VC} > \text{simplify}\left(\text{subs}\left(\left\{a=0, b=-\frac{1}{2}\pi, r=r, t=t, \alpha=0, \varepsilon=0\right\}, \text{Neg0}\right)\right)$$

0

(1.7.2)

### W2+W3

```
> part1 := evalDG(Nw-ContractIndices(J, RearrangeIndices(ContractIndices(J, Nw, [[1,
2]]), [2, 1, 3]), [[1, 1]])) :
> condw23 := {op(DGinfo(deltaW, "CoefficientSet")), op(DGinfo(evalDG(part1
+ RearrangeIndices(part1, [3, 1, 2]) + RearrangeIndices(part1, [2, 3, 1])),
"CoefficientSet"))} :
> solve({op(condw23), t ≠ 0, Neg0 ≠ 0, Negw2 ≠ 0, Negw3 ≠ 0});
> Negw23 := add(condw23[i]^2, i = 1..nops(condw23)) :
```

### W2+W4

```
> condw24 := DGinfo(evalDG(ExteriorDerivative(W) - W &w Lee), "CoefficientSet") :
> solve({op(condw24), t ≠ 0, Neg0 ≠ 0, Negw2 ≠ 0, Negw4 ≠ 0});
> Negw24 := add(condw24[i]^2, i = 1..nops(condw24)) :
```

### W3+W4

```
> condw34 := DGinfo(NJ, "CoefficientSet") :
> solve({op(condw34), t ≠ 0, Neg0 ≠ 0, Negw3 ≠ 0, Negw4 ≠ 0})
{a=a, α=0, b=b, ε=ε, r=0, t=t}, {a=0, α=α, b=1/2 π, ε=ε, r=r, t=t}, {a=0, α(1.10.1)
=α, b=-1/2 π, ε=ε, r=r, t=t}
```

```
> Negw34 := add(condw34[i]^2, i = 1..nops(condw34)) :
> simplify(subs({a=a, b=b, r=0, t=t, α=0, ε=ε}, Neg0), trig)
ε2
(1.10.2)
```

```
VC > simplify(subs({a=0, b=1/2 π, r=r, t=t, α=α, ε=ε}, Neg0), trig);
2(-1/2 ε + 1/2 α t)2 + 2(1/2 ε - 1/2 α t)2
(1.10.3)
```

```
VC > simplify(subs({a=0, b=-1/2 π, r=r, t=t, α=α, ε=ε}, Neg0), trig);
2(-1/2 ε - 1/2 α t)2 + 2(1/2 ε + 1/2 α t)2
(1.10.4)
```

### W1+W2+W3

```
> condw123 := DGinfo(deltaW, "CoefficientSet") :
> solve({op(condw123), t ≠ 0, Neg0 ≠ 0, Negw1 ≠ 0, Negw3 ≠ 0, Negw12 ≠ 0, Negw13
≠ 0, Negw23 ≠ 0})
```

(1.11.1)

$$\{a = a, \alpha = \alpha, b = b, \varepsilon = t \alpha \cos(a) \sin(b), r = r, t = t\} \quad (1.11.1)$$

### W1+W2+W4

```
> condw124 := DGinfo(evalDG(mu + ContractIndices(J,
  RearrangeIndices(ContractIndices(J, mu, [[1, 2]]), [2, 1, 3]), [[1, 1]])),
  "CoefficientSet") :
> solve({op(condw124), t ≠ 0, Neg0 ≠ 0, Negw1 ≠ 0, Negw4 ≠ 0, Negw12 ≠ 0, Negw14
  ≠ 0, Negw24 ≠ 0});
```

### W1+W3+W4

```
> part1 := SymmetrizeIndices(Nw, [1, 2], "Symmetric") :
> condw134 := DGinfo(evalDG(part1 - ContractIndices(J,
  RearrangeIndices(ContractIndices(J, part1, [[1, 2]]), [2, 1, 3]), [[1, 1]])),
  "CoefficientSet") :
> use RealDomain in solve({op(condw134), t ≠ 0, Neg0 ≠ 0}) end use
{a = a, α = 0, b = b, ε = ε, r = 0, t = t}, {a = 0, α = α, b = 1/2 π, ε = ε, r = r, t = t}, {a = 0, α = α,
  = α, b = -1/2 π, ε = ε, r = r, t = t}, {a = π, α = α, b = 1/2 π, ε = ε, r = r, t = t}, {a = π, α
  = α, b = -1/2 π, ε = ε, r = r, t = t}
> simplify(subs({a = a, α = 0, b = b, ε = ε, r = 0, t = t}, Negw34), trig)
0
```

(1.13.2)

### W2+W3+W4

```
> part1 := evalDG(Nw - ContractIndices(J, RearrangeIndices(ContractIndices(J, Nw,
  [[1, 2]]), [2, 1, 3]), [[1, 1]])) :
> condw234 := DGinfo(evalDG(part1 + RearrangeIndices(part1, [3, 1, 2])
  + RearrangeIndices(part1, [2, 3, 1])), "CoefficientSet") :
> use RealDomain in solve({op(condw234), t ≠ 0, Neg0 ≠ 0, Negw3 ≠ 0, Negw4 ≠ 0,
  Negw23 ≠ 0, Negw24 ≠ 0, Negw34 ≠ 0}) end use
```

## A1.2

[This algebra contains a free quaternion parameter. We parameterize this as  $p = M*i + L*j + K*k$

```
> restart : with(DifferentialGeometry) : with(LieAlgebras) : with(Tensor) : with(Tools) :
  with(LinearAlgebra) :
```

```
> StructureEquations := [[ee, ii] = e + M*ie, [ee, jj] = L*ie, [ee, kk] = K*ie, [ii, jj] = -K*ie,
  [ii, kk] = L*ie, [jj, kk] = -e - M*ie], [ee, ii, jj, kk, e, ie] :
```

```
LL := LieAlgebraData(StructureEquations, VC);
```

```
LL := [[e1, e2] = M e6 + e5, [e1, e3] = L e6, [e1, e4] = K e6, [e2, e3] = -K e6, [e2, e4]
  = L e6, [e3, e4] = -M e6 - e5] (2.1)
```

```
> DGsetup(LL, [e], [f]) :
```

```
> Query("Jacobi");
```

(2.2)

*true*

(2.2)

> g := evalDG((f1 &t f1 + f2 &t f2 + f3 &t f3 + f4 &t f4) + t·(f5 &t f5 + f6 &t f6));

*g := f1 f1 + f2 f2 + f3 f3 + f4 f4 + t f5 f5 + t f6 f6*

(2.3)

> J0 := Matrix([ [0, -cos(a) sin(b), -sin(a) sin(b), -cos(b), 0, 0], [cos(a) sin(b), 0, cos(b), -sin(a) sin(b), 0, 0], [sin(a) sin(b), -cos(b), 0, cos(a) sin(b), 0, 0], [cos(b), sin(a) sin(b), -cos(a) sin(b), 0, 0, 0], [0, 0, 0, 0, 0, -1], [0, 0, 0, 0, 1, 0]]);

$$J0 := \begin{bmatrix} 0 & -\cos(a) \sin(b) & -\sin(a) \sin(b) & -\cos(b) & 0 & 0 \\ \cos(a) \sin(b) & 0 & \cos(b) & -\sin(a) \sin(b) & 0 & 0 \\ \sin(a) \sin(b) & -\cos(b) & 0 & \cos(a) \sin(b) & 0 & 0 \\ \cos(b) & \sin(a) \sin(b) & -\cos(a) \sin(b) & 0 & 0 & 0 \\ 0 & 0 & 0 & 0 & 0 & -1 \\ 0 & 0 & 0 & 0 & 1 & 0 \end{bmatrix}$$

(2.4)

> J := convert(J0, DGtensor, [[ "con\_bas", "cov\_bas"], [ ]]);

*J := -cos(a) sin(b) e1 f2 - sin(a) sin(b) e1 f3 - cos(b) e1 f4 + cos(a) sin(b) e2 f1 + cos(b) e2 f3 - sin(a) sin(b) e2 f4 + sin(a) sin(b) e3 f1 - cos(b) e3 f2 + cos(a) sin(b) e3 f4 + cos(b) e4 f1 + sin(a) sin(b) e4 f2 - cos(a) sin(b) e4 f3 - e5 f6 + e6 f5*

(2.5)

> w := ContractIndices(J, g, [[1, 1]]);

*w := cos(a) sin(b) f1 f2 + sin(a) sin(b) f1 f3 + cos(b) f1 f4 - cos(a) sin(b) f2 f1 - cos(b) f2 f3 + sin(a) sin(b) f2 f4 - sin(a) sin(b) f3 f1 + cos(b) f3 f2 - cos(a) sin(b) f3 f4 - cos(b) f4 f1 - sin(a) sin(b) f4 f2 + cos(a) sin(b) f4 f3 + t f5 f6 - t f6 f5*

(2.6)

> W := convert(w, DGform);

*W := cos(a) sin(b) f1 ∧ f2 + sin(a) sin(b) f1 ∧ f3 + cos(b) f1 ∧ f4 - cos(b) f2 ∧ f3 + sin(a) sin(b) f2 ∧ f4 - cos(a) sin(b) f3 ∧ f4 + t f5 ∧ f6*

(2.7)

> Nabla := Christoffel(g) :

> Nw := RearrangeIndices(CovariantDerivative(w, Nabla), [2, 3, 1]) :

> NJ := TensorBrackets(J, J, "Frolicher-Nijenhuis") :

> deltaW := HodgeStar(g, ExteriorDerivative(HodgeStar(g, W))) :

> Lee := convert( evalDG( - 1/2 · ContractIndices(J, HodgeStar(g, ExteriorDerivative(HodgeStar(g, W)))) ), DGform );

*Lee := -t (L sin(a) sin(b) + M cos(a) sin(b) + K cos(b)) f5 + t cos(a) sin(b) f6*

(2.8)

> part2 := SymmetrizeIndices(evalDG(g &t deltaW), [2, 3], "SkewSymmetric") :

> part3 := SymmetrizeIndices(RearrangeIndices(ContractIndices(J, ContractIndices(evalDG(g &t deltaW), J, [[3, 1]]), [[1, 2]]), [2, 1, 3]), [2, 3], "SkewSymmetric") :

> mu := evalDG( Nw + 1/2 · ( part2 - part3 ) ) :

0

```

[> cond0 := DGinfo(Nw, "CoefficientSet") :
[> sol0 := solve( {op(cond0), t ≠ 0} );
[> Neg0 := add( cond0[i]2, i = 1 ..nops(cond0) ) :

```

(2.1.1)

W1

```

[> SNw := SymmetrizeIndices(Nw, [1, 2, 3], "SkewSymmetric") :
[> condw1 := DGinfo(evalDG(Nw - SNw), "CoefficientSet") :
[> solve( {op(condw1), t ≠ 0, Neg0 ≠ 0} );
[> Negw1 := add( condw1[i]2, i = 1 ..nops(condw1) ) :

```

W3

```

[> condw3 := {op(DGinfo(deltaW, "CoefficientSet")), op(DGinfo(NJ,
"CoefficientSet"))} :
[> solve( {op(condw3), t ≠ 0, Neg0 ≠ 0} )
{K = 0, L = 1, M = 0, a = a, b = π, t = t}, {K = 0, L = -1, M = 0, a = a, b = 0, t = t}, {K
= sin(b), L = -cos(b), M = 0, a =  $\frac{1}{2}$  π, b = b, t = t}, {K = -sin(b), L = -cos(b), M
= 0, a = - $\frac{1}{2}$  π, b = b, t = t}
[> Negw3 := add( condw3[i]2, i = 1 ..nops(condw3) ) :

```

(2.3.1)

W4

```

[> condw4 := DGinfo(mu, "CoefficientSet") :
[> solve( {op(condw4), t ≠ 0, Neg0 ≠ 0} );
[> Negw4 := add( condw4[i]2, i = 1 ..nops(condw4) ) :

```

W1+W2

```

[> condw12 := DGinfo(DGsimply(simplify(evalDG(Nw
+ RearrangeIndices(ContractIndices(J, ContractIndices(J, Nw, [[1, 1]]), [[1,
3]]), [3, 1, 2]))), "CoefficientSet") :
[> use RealDomain in solve( {op(condw12), t ≠ 0, Neg0 ≠ 0, Negw1 ≠ 0} ) end use
{K = 0, L = 1, M = 0, a = a, b = 0, t = t}, {K = 0, L = -1, M = 0, a = a, b = π, t = t}, {K
= sin(b), L = cos(b), M = 0, a = - $\frac{1}{2}$  π, b = b, t = t}, {K = -sin(b), L = cos(b), M
= 0, a =  $\frac{1}{2}$  π, b = b, t = t}

```

(2.5.1)

```

> Negw12 := add(condw12[i]^2, i = 1..nops(condw12)) :
VC > simplify(subs({K=0, L=1, M=0, a=a, b=0, r=r, t=t}, Neg0), trig);
8 t^2 (2.5.2)

```

### W1+W3

```

> condw13 := {op(DGinfo(deltaW, "CoefficientSet")),
  op(DGinfo(SymmetrizeIndices(evalDG(Nw-ContractIndices(J,
  RearrangeIndices(ContractIndices(J, Nw, [[1, 3]]), [3, 1, 2]), [[1, 1]])), [1, 3],
  "Symmetric"), "CoefficientSet"))} :
> use RealDomain in solve({op(condw13), t ≠ 0}) end use;
{K=0, L=1, M=0, a=a, b=π, t=t}, {K=0, L=-1, M=0, a=a, b=0, t=t}, {K
(2.6.1)
  = sin(b), L = -cos(b), M=0, a = 1/2 π, b=b, t=t}, {K = -sin(b), L = -cos(b), M
  = 0, a = -1/2 π, b=b, t=t}
> Negw13 := add(condw13[i]^2, i = 1..nops(condw13)) :
> simplify(subs({K = -sin(b), L = -cos(b), M=0, a = -1/2 π, b=b, r=r, t=t}, Negw3),
  trig)
0 (2.6.2)

```

### W1+W4

```

> condw14 := DGinfo(SymmetrizeIndices(mu, [1, 2], "Symmetric"), "CoefficientSet") :
> solve({op(condw14), t ≠ 0, Neg0 ≠ 0, Negw1 ≠ 0, Negw4 ≠ 0});
> Negw14 := add(condw14[i]^2, i = 1..nops(condw14)) :

```

### W2+W3

```

> part1 := evalDG(Nw-ContractIndices(J, RearrangeIndices(ContractIndices(J, Nw, [[1,
  2]]), [2, 1, 3]), [[1, 1]])) :
> condw23 := {op(DGinfo(deltaW, "CoefficientSet")), op(DGinfo(evalDG(part1
  + RearrangeIndices(part1, [3, 1, 2]) + RearrangeIndices(part1, [2, 3, 1])),
  "CoefficientSet"))} :
> solve({op(condw23), t ≠ 0});
{K=0, L=1, M=0, a=a, b=π, t=t}, {K=0, L=-1, M=0, a=a, b=0, t=t}, {K
(2.8.1)
  = sin(b), L = -cos(b), M=0, a = 1/2 π, b=b, t=t}, {K = -sin(b), L = -cos(b), M
  = 0, a = -1/2 π, b=b, t=t}

```



**VC** >  $\text{simplify}\left(\text{subs}\left(\left\{K = -\sin(b), L = -\cos(b), M = 0, a = -\frac{1}{2}\pi, b = b, r = r, t = t\right\}, \text{Negw3}\right), \text{trig}\right);$

0

(2.8.2)

>  $\text{Negw23} := \text{add}(\text{condw23}[i]^2, i = 1 \dots \text{nops}(\text{condw23})) :$

## W2+W4

>  $\text{condw24} := \text{DGinfo}(\text{evalDG}(\text{ExteriorDerivative}(W) - W \&w Lee), \text{"CoefficientSet"}) :$

>  $\text{solve}(\{op(\text{condw24}), t \neq 0, \text{Neg0} \neq 0, \text{Negw2} \neq 0, \text{Negw4} \neq 0\});$

>  $\text{Negw24} := \text{add}(\text{condw24}[i]^2, i = 1 \dots \text{nops}(\text{condw24})) :$

## W3+W4

>  $\text{condw34} := \text{DGinfo}(\text{NJ}, \text{"CoefficientSet"}) :$

>  $\text{solve}(\{op(\text{condw34}), t \neq 0, \text{Neg0} \neq 0, \text{Negw3} \neq 0, \text{Negw4} \neq 0\})$

$\{K = K, L = 1, M = 0, a = a, b = \pi, t = t\}, \{K = K, L = -1, M = 0, a = a, b = 0, t = t\}, \{K$  (2.10.1)

$$\begin{aligned} &= 1, L = L, M = 0, a = \frac{1}{2}\pi, b = \frac{1}{2}\pi, t = t\}, \{K = 1, L = L, M = 0, a = -\frac{1}{2}\pi, b = \\ &-\frac{1}{2}\pi, t = t\}, \{K = -1, L = L, M = 0, a = \frac{1}{2}\pi, b = -\frac{1}{2}\pi, t = t\}, \{K = -1, L = L, M \\ &= 0, a = -\frac{1}{2}\pi, b = \frac{1}{2}\pi, t = t\}, \{K = \sin(a), L = \frac{M \sin(a)}{\cos(a)}, M = M, a = a, b \\ &= \frac{1}{2}\pi, t = t\}, \{K = -\sin(a), L = \frac{M \sin(a)}{\cos(a)}, M = M, a = a, b = -\frac{1}{2}\pi, t = t\}, \{K \\ &= K, L = -\frac{K \sin(b) + 1}{\cos(b)}, M = 0, a = -\frac{1}{2}\pi, b = b, t = t\}, \{K = K, L \\ &= \frac{K \sin(b) - 1}{\cos(b)}, M = 0, a = \frac{1}{2}\pi, b = b, t = t\}, \{K \\ &= \frac{-\sin(a)^3 \sin(b)^2 + M \cos(a) \cos(b) + \sin(b)^2 \sin(a)}{\sin(b) \cos(a)^2}, L \\ &= \frac{\sin(a) M \cos(a) + \cos(b) \sin(a)^2 - \cos(b)}{\cos(a)^2}, M = M, a = a, b = b, t = t\} \end{aligned}$$

**VC** >  $\text{simplify}\left(\text{subs}\left(\left\{K = \frac{-\sin(a)^3 \sin(b)^2 + M \cos(a) \cos(b) + \sin(b)^2 \sin(a)}{\sin(b) \cos(a)^2}, L\right.\right.\right.$

$$= \frac{\sin(a) M \cos(a) + \cos(b) \sin(a)^2 - \cos(b)}{\cos(a)^2}, M = M, a = a, b = b, r = r, t$$

$\left. = t\right\}, \text{Negw3}\right), \text{trig}\right)$

$$\frac{4t^2 (\cos(a)^4 \cos(b)^4 - 2 \cos(b)^2 \cos(a)^4 + \cos(a)^4 + M^2)}{\cos(a)^2 \sin(b)^2}$$

(2.10.2)

$$\lfloor \triangleright Negw34 := add(condw34[i]^2, i = 1 .. nops(condw34)) :$$

**W1+W2+W3**

$$\begin{aligned} &> \text{condw123} := \text{DGinfo}(\text{deltaW}, \text{"CoefficientSet"}) : \\ &> \text{solve}(\{op(\text{condw123}), t \neq 0, \text{Neg0} \neq 0, \text{Negw1} \neq 0, \text{Negw3} \neq 0, \text{Negw12} \neq 0, \text{Negw13} \\ &\quad \neq 0, \text{Negw23} \neq 0\}) \\ &\left\{K = -L \tan(b), L = L, M = M, a = \frac{1}{2} \pi, b = b, t = t\right\}, \left\{K = L \tan(b), L = L, M = M, a = \right. \quad (2.11.1) \\ &\quad \left. - \frac{1}{2} \pi, b = b, t = t\right\}, \{K = 0, L = L, M = M, a = a, b = 0, t = t\} \\ &> \text{simplify}\left(\text{subs}\left(\left\{K = -L \tan(b), L = L, M = M, a = \frac{1}{2} \pi, b = b, t = t\right\}, \text{Negw3}\right), \text{trig}\right) \\ &\quad \frac{64 (M^2 \cos(b)^2 + L^2 + 2 L \cos(b) + \cos(b)^2)}{\cos(b)^2} \quad (2.11.2) \end{aligned}$$

**W1+W2+W4**

```

> condw124 := DGinfo(evalDG(mu + ContractIndices(J,
  RearrangeIndices(ContractIndices(J, mu, [[1, 2]]), [2, 1, 3]), [[1, 1]])),
  "CoefficientSet") :
> solve({op(condw124), t ≠ 0, Neg0 ≠ 0, Negw1 ≠ 0, Negw4 ≠ 0, Negw12 ≠ 0, Negw14
  ≠ 0, Negw24 ≠ 0});

```

**W1+W3+W4**

```

> part1 := SymmetrizeIndices(Nw, [1, 2], "Symmetric") :
> condw134 := DGinfo(evalDG(part1 - ContractIndices(J,
  RearrangeIndices(ContractIndices(J, part1, [[1, 2]]), [2, 1, 3]), [[1, 1]])),
  "CoefficientSet") :
> use RealDomain in solve( {op(condw134), t ≠ 0} ) end use

```

$$\{K = K, L = 1, M = 0, a = a, b = \pi, t = t\}, \{K = K, L = -1, M = 0, a = a, b = 0, t = t\}, \left\{ K \right. \quad (2.13.1)$$

$$= 1, L = L, M = 0, a = \frac{1}{2} \pi, b = \frac{1}{2} \pi, t = t\}, \left\{ K = 1, L = L, M = 0, a = -\frac{1}{2} \pi, b = \right.$$

$$-\frac{1}{2} \pi, t = t\}, \left\{ K = -1, L = L, M = 0, a = \frac{1}{2} \pi, b = -\frac{1}{2} \pi, t = t\}, \left\{ K = -1, L = L, M \right.$$

$$= 0, a = -\frac{1}{2} \pi, b = \frac{1}{2} \pi, t = t\}, \left\{ K = \sin(a), L = \frac{M \sin(a)}{\cos(a)}, M = M, a = a, b \right.$$

$$= \frac{1}{2} \pi, t = t\}, \left\{ K = -\sin(a), L = \frac{M \sin(a)}{\cos(a)}, M = M, a = a, b = -\frac{1}{2} \pi, t = t\}, \left\{ K \right.$$

$$= K, L = \frac{K \sin(b) - 1}{\cos(b)}, M = 0, a = \frac{1}{2} \pi, b = b, t = t\}, \left\{ K = K, L = -\frac{K \sin(b) + 1}{\cos(b)}, \right.$$

$$M = 0, a = -\frac{1}{2} \pi, b = b, t = t\}, \left\{ K \right.$$

$$= \frac{-\sin(a) \cos(b)^2 \cos(a) + M \cos(b) + \sin(a) \cos(a)}{\cos(a) \sin(b)}, L$$

$$= \frac{M \sin(a) - \cos(b) \cos(a)}{\cos(a)}, M=M, a=a, b=b, t=t \}$$

$$\text{VC} > \text{simplify} \left( \text{subs} \left( \left\{ K = \frac{-\sin(a) \cos(b)^2 \cos(a) + M \cos(b) + \sin(a) \cos(a)}{\cos(a) \sin(b)}, L \right. \right. \right. \\ \left. \left. \left. = \frac{M \sin(a) - \cos(b) \cos(a)}{\cos(a)}, M=M, a=a, b=b, t=t \right\}, \text{Negw34} \right), \text{trig} \right) \\ 0 \quad (2.13.2)$$

## W2+W3+W4

$$\begin{aligned} &> \text{part1} := \text{evalDG}(\text{Nw} - \text{ContractIndices}(J, \text{RearrangeIndices}(\text{ContractIndices}(J, \text{Nw}, \\ &\quad [[1, 2]]), [2, 1, 3]), [[1, 1]])) : \\ &> \text{condw234} := \text{DGinfo}(\text{evalDG}(\text{part1} + \text{RearrangeIndices}(\text{part1}, [3, 1, 2]) \\ &\quad + \text{RearrangeIndices}(\text{part1}, [2, 3, 1])), \text{"CoefficientSet"}) : \\ &> \text{use RealDomain in solve}(\{op(\text{condw234}), t \neq 0, \text{Neg0} \neq 0, \text{Negw3} \neq 0, \text{Negw4} \neq 0, \\ &\quad \text{Negw23} \neq 0, \text{Negw24} \neq 0, \text{Negw34} \neq 0\}) \text{ end use} \\ &\left\{ K = \frac{-\cos(a) \cos(b)^2 \sin(a) + M \cos(b) + \sin(a) \cos(a)}{\cos(a) \sin(b)}, L \right. \end{aligned} \quad (2.14.1)$$

$$\begin{aligned} &= \frac{M \sin(a) - \cos(b) \cos(a)}{\cos(a)}, M=M, a=a, b=b, t=t \} \\ &> \text{simplify} \left( \text{subs} \left( \left\{ K = \frac{-\cos(b)^2 \sin(a) \cos(a) + M \cos(b) + \sin(a) \cos(a)}{\cos(a) \sin(b)}, L \right. \right. \right. \\ &\quad \left. \left. \left. = \frac{M \sin(a) - \cos(b) \cos(a)}{\cos(a)}, M=M, a=a, b=b, r=r, t=t \right\}, \text{Negw34} \right), \text{trig} \right) \\ &0 \quad (2.14.2) \end{aligned}$$

## A1.3

$$\begin{aligned} &> \text{restart} : \text{with}(\text{DifferentialGeometry}) : \text{with}(\text{LieAlgebras}) : \text{with}(\text{Tensor}) : \text{with}(\text{Tools}) : \\ &\quad \text{with}(\text{LinearAlgebra}) : \\ &> \text{StructureEquations} := [[\text{ee}, \text{e}] = \alpha * \text{ee}, [\text{ii}, \text{e}] = \alpha * \text{ii}, [\text{jj}, \text{e}] = \alpha * \text{jj}, [\text{kk}, \text{e}] = \alpha * \text{kk}, [\text{ee}, \text{ie}] \\ &\quad = \beta * \text{ee} + r * \text{ii}, [\text{ii}, \text{ie}] = \beta * \text{ii} - r * \text{ee}, [\text{jj}, \text{ie}] = \beta * \text{jj} - r * \text{kk}, [\text{kk}, \text{ie}] = \beta * \text{kk} + r * \text{jj}, [\text{e}, \\ &\quad \text{ie}] = \epsilon * \text{e}], [\text{ee}, \text{ii}, \text{jj}, \text{kk}, \text{e}, \text{ie}] : \\ &\quad L := \text{LieAlgebraData}(\text{StructureEquations}, \text{VC}); \\ &\quad L := [[\text{e1}, \text{e5}] = \alpha \text{e1}, [\text{e1}, \text{e6}] = \beta \text{e1} + \text{e2} \text{r}, [\text{e2}, \text{e5}] = \alpha \text{e2}, [\text{e2}, \text{e6}] = \beta \text{e2} - \text{e1} \text{r}, [\text{e3}, \text{e5}] \\ &\quad = \alpha \text{e3}, [\text{e3}, \text{e6}] = \beta \text{e3} - \text{e4} \text{r}, [\text{e4}, \text{e5}] = \alpha \text{e4}, [\text{e4}, \text{e6}] = \beta \text{e4} + \text{e3} \text{r}, [\text{e5}, \text{e6}] = \epsilon \text{e5}] \end{aligned} \quad (3.1)$$

$$\begin{aligned} &> \text{DGsetup}(L, [\text{e}], [\text{f}]) : \\ &> \text{Query}(\{\alpha, \beta, \epsilon\}, \text{"Jacobi"}); \\ &\text{true}, \{0, -\epsilon \alpha\}, [\{\alpha = \alpha, \beta = \beta, \epsilon = 0\}, \{\alpha = 0, \beta = \beta, \epsilon = \epsilon\}], [[[\text{e1}, \text{e5}] = \alpha \text{e1}, [\text{e1}, \text{e6}] \\ &\quad = \beta \text{e1} + \text{e2} \text{r}, [\text{e2}, \text{e5}] = \alpha \text{e2}, [\text{e2}, \text{e6}] = \beta \text{e2} - \text{e1} \text{r}, [\text{e3}, \text{e5}] = \alpha \text{e3}, [\text{e3}, \text{e6}] = \beta \text{e3} \\ &\quad - \text{e4} \text{r}, [\text{e4}, \text{e5}] = \alpha \text{e4}, [\text{e4}, \text{e6}] = \beta \text{e4} + \text{e3} \text{r}], [[\text{e1}, \text{e6}] = \beta \text{e1} + \text{e2} \text{r}, [\text{e2}, \text{e6}] = \beta \text{e2} \end{aligned} \quad (3.2)$$

$$-e_1 r, [e_3, e_6] = \beta e_3 - e_4 r, [e_4, e_6] = \beta e_4 + e_3 r, [e_5, e_6] = \varepsilon e_5]$$

$$\begin{aligned} &> g := \text{evalDG}((f_1 \wedge t f_1 + f_2 \wedge t f_2 + f_3 \wedge t f_3 + f_4 \wedge t f_4) + t \cdot (f_5 \wedge t f_5 + f_6 \wedge t f_6)); \\ &\quad g := f_1 f_1 + f_2 f_2 + f_3 f_3 + f_4 f_4 + t f_5 f_5 + t f_6 f_6 \end{aligned} \quad (3.3)$$

$$\begin{aligned} &> J0 := \text{Matrix}([ [0, -\cos(a) \sin(b), -\sin(a) \sin(b), -\cos(b), 0, 0], [\cos(a) \sin(b), 0, \\ &\quad \cos(b), -\sin(a) \sin(b), 0, 0], [\sin(a) \sin(b), -\cos(b), 0, \\ &\quad \cos(a) \sin(b), 0, 0], [\cos(b), \sin(a) \sin(b), -\cos(a) \sin(b), 0, 0, 0], [0, 0, 0, 0, 0, -1], \\ &\quad [0, 0, 0, 0, 1, 0]]); \end{aligned}$$

$$J0 := \begin{bmatrix} 0 & -\cos(a) \sin(b) & -\sin(a) \sin(b) & -\cos(b) & 0 & 0 \\ \cos(a) \sin(b) & 0 & \cos(b) & -\sin(a) \sin(b) & 0 & 0 \\ \sin(a) \sin(b) & -\cos(b) & 0 & \cos(a) \sin(b) & 0 & 0 \\ \cos(b) & \sin(a) \sin(b) & -\cos(a) \sin(b) & 0 & 0 & 0 \\ 0 & 0 & 0 & 0 & 0 & -1 \\ 0 & 0 & 0 & 0 & 1 & 0 \end{bmatrix} \quad (3.4)$$

$$\begin{aligned} &> J := \text{convert}(J0, \text{DGtensor}, [[\text{"con\_bas"}, \text{"cov\_bas"}], []]); \\ J &:= -\cos(a) \sin(b) e_1 f_2 - \sin(a) \sin(b) e_1 f_3 - \cos(b) e_1 f_4 + \cos(a) \sin(b) e_2 f_1 \\ &\quad + \cos(b) e_2 f_3 - \sin(a) \sin(b) e_2 f_4 + \sin(a) \sin(b) e_3 f_1 - \cos(b) e_3 f_2 \\ &\quad + \cos(a) \sin(b) e_3 f_4 + \cos(b) e_4 f_1 + \sin(a) \sin(b) e_4 f_2 - \cos(a) \sin(b) e_4 f_3 \\ &\quad - e_5 f_6 + e_6 f_5 \end{aligned} \quad (3.5)$$

$$\begin{aligned} &> w := \text{ContractIndices}(J, g, [[1, 1]]); \\ w &:= \cos(a) \sin(b) f_1 f_2 + \sin(a) \sin(b) f_1 f_3 + \cos(b) f_1 f_4 - \cos(a) \sin(b) f_2 f_1 \\ &\quad - \cos(b) f_2 f_3 + \sin(a) \sin(b) f_2 f_4 - \sin(a) \sin(b) f_3 f_1 + \cos(b) f_3 f_2 \\ &\quad - \cos(a) \sin(b) f_3 f_4 - \cos(b) f_4 f_1 - \sin(a) \sin(b) f_4 f_2 + \cos(a) \sin(b) f_4 f_3 \\ &\quad + t f_5 f_6 - t f_6 f_5 \end{aligned} \quad (3.6)$$

$$\begin{aligned} &> W := \text{convert}(w, \text{DGform}); \\ W &:= \cos(a) \sin(b) f_1 \wedge f_2 + \sin(a) \sin(b) f_1 \wedge f_3 + \cos(b) f_1 \wedge f_4 - \cos(b) f_2 \wedge f_3 \\ &\quad + \sin(a) \sin(b) f_2 \wedge f_4 - \cos(a) \sin(b) f_3 \wedge f_4 + t f_5 \wedge f_6 \end{aligned} \quad (3.7)$$

$$> \text{Nabla} := \text{Christoffel}(g);$$

$$> Nw := \text{RearrangeIndices}(\text{CovariantDerivative}(w, \text{Nabla}), [2, 3, 1]);$$

$$> NJ := \text{TensorBrackets}(J, J, \text{"Frolicher-Nijenhuis"});$$

$$> \text{delta}W := \text{HodgeStar}(g, \text{ExteriorDerivative}(\text{HodgeStar}(g, W)));$$

$$\begin{aligned} &> Lee := \text{convert}\left(\text{evalDG}\left(-\frac{1}{2} \cdot \text{ContractIndices}(J, \text{HodgeStar}(g, \right. \right. \\ &\quad \left. \left. \text{ExteriorDerivative}(\text{HodgeStar}(g, W))), [[1, 1]]\right), \text{DGform}\right); \\ &\quad Lee := -2 \alpha f_5 - 2 \beta f_6 \end{aligned} \quad (3.8)$$

$$> \text{part2} := \text{SymmetrizeIndices}(\text{evalDG}(g \wedge \text{delta}W), [2, 3], \text{"SkewSymmetric"});$$

$$\begin{aligned} &> \text{part3} := \text{SymmetrizeIndices}(\text{RearrangeIndices}(\text{ContractIndices}(J, \\ &\quad \text{ContractIndices}(\text{evalDG}(g \wedge \text{delta}W), J, [[3, 1]]), [[1, 2]]), [2, 1, 3]), [2, 3], \\ &\quad \text{"SkewSymmetric"}); \end{aligned}$$

$$> \mu := \text{evalDG}\left(Nw + \frac{1}{2} \cdot (\text{part2} - \text{part3})\right);$$

0

```

[> cond0 := DGinfo(Nw, "CoefficientSet") :
[> sol0 := solve( {op(cond0), t ≠ 0} );
    sol0 := {a = a, α = 0, b = b, β = 0, r = 0, t = t}, {a = 0, α = 0, b = 1/2 π, β = 0, r = r, t = t} (3.1.1)
[> Neg0 := add(cond0[i]2, i = 1 .. nops(cond0)) :

```

W1

```

[> SNw := SymmetrizeIndices(Nw, [1, 2, 3], "SkewSymmetric") :
[> condw1 := DGinfo(evalDG(Nw - SNw), "CoefficientSet") :
[> solve( {op(condw1), t ≠ 0, Neg0 ≠ 0} );
    {a = 0, α = 0, b = 1/2 π, β = 0, r = r, t = t}, {a = 0, α = 0, b = -1/2 π, β = 0, r = r, t = t} (3.2.1)
[> Negw1 := add(condw1[i]2, i = 1 .. nops(condw1)) :
[> simplify( subs( {a = 0, b = 1/2 π, r = r, t = t, α = 0, β = 0}, Neg0 ) );
    0 (3.2.2)

```

W3

```

[> condw3 := {op(DGinfo(deltaW, "CoefficientSet")), op(DGinfo(NJ,
    "CoefficientSet"))} :
[> solve( {op(condw3), t ≠ 0, Neg0 ≠ 0} )
[> Negw3 := add(condw3[i]2, i = 1 .. nops(condw3)) :

```

W4

```

[> condw4 := DGinfo(mu, "CoefficientSet") :
[> solve( {op(condw4), t ≠ 0, Neg0 ≠ 0} );
    {a = 0, α = 0, b = 1/2 π, β = 0, r = r, t = t}, {a = 0, α = 0, b = -1/2 π, β = 0, r = r, t = t} (3.4.1)
[vc > simplify( subs( {a = 0, b = -1/2 π, r = r, t = t, α = 0, β = 0}, Neg0 ), trig )
    0 (3.4.2)
[> Negw4 := add(condw4[i]2, i = 1 .. nops(condw4)) :

```

W1+W2

```

[> condw12 := DGinfo(DGsimpify(simplify(evalDG(Nw
    + RearrangeIndices(ContractIndices(J, ContractIndices(J, Nw, [[1, 1]]), [[1,
    3]]), [3, 1, 2]))), "CoefficientSet") :
[> use RealDomain in solve( {op(condw12), t ≠ 0, Neg0 ≠ 0, Negw1 ≠ 0, Negw2 ≠ 0} )
    end use
[> Negw12 := add(condw12[i]2, i = 1 .. nops(condw12)) :

```

### W1+W3

```

> condw13 := {op(DGinfo(deltaW, "CoefficientSet")),
  op(DGinfo(SymmetrizeIndices(evalDG(Nw-ContractIndices(J,
  RearrangeIndices(ContractIndices(J, Nw, [[1, 3]]), [3, 1, 2]), [[1, 1]])), [1, 3],
  "Symmetric"), "CoefficientSet"))}:
> use RealDomain in solve( {op(condw13), t ≠ 0, Neg0 ≠ 0, Negw1 ≠ 0, Negw3 ≠ 0} )
end use;
> Negw13 := add(condw13[i]^2, i = 1..nops(condw13)) :

```

### W1+W4

```

> condw14 := DGinfo(SymmetrizeIndices(mu, [1, 2], "Symmetric"), "CoefficientSet") :
> solve( {op(condw14), t ≠ 0, Neg0 ≠ 0, Negw1 ≠ 0, Negw4 ≠ 0} );
  {a=0, α=0, b= 1/2 π, β=0, r=r, t=t}, {a=0, α=0, b= -1/2 π, β=0, r=r, t=t} (3.7.1)
> Negw14 := add(condw14[i]^2, i = 1..nops(condw14)) :

```

### W2+W3

```

> part1 := evalDG(Nw-ContractIndices(J, RearrangeIndices(ContractIndices(J, Nw, [[1,
  2]]), [2, 1, 3]), [[1, 1]])) :
> condw23 := {op(DGinfo(deltaW, "CoefficientSet")), op(DGinfo(evalDG(part1
  + RearrangeIndices(part1, [3, 1, 2]) + RearrangeIndices(part1, [2, 3, 1])),
  "CoefficientSet"))}:
> solve( {op(condw23), t ≠ 0, Neg0 ≠ 0, Negw2 ≠ 0, Negw3 ≠ 0} );
> Negw23 := add(condw23[i]^2, i = 1..nops(condw23)) :

```

### W2+W4

```

> condw24 := DGinfo(evalDG(ExteriorDerivative(W) - W&w Lee), "CoefficientSet") :
> solve( {op(condw24), t ≠ 0, Neg0 ≠ 0, Negw4 ≠ 0} );
  {a=0, α=0, b= 1/2 π, β=0, r=r, t=t}, {a=0, α=0, b= -1/2 π, β=0, r=r, t=t} (3.9.1)
> Negw24 := add(condw24[i]^2, i = 1..nops(condw24)) :

```

### W3+W4

```

> condw34 := DGinfo(NJ, "CoefficientSet") :
> solve( {op(condw34), t ≠ 0, Neg0 ≠ 0, Negw3 ≠ 0, Negw4 ≠ 0} )
  {a=a, α=α, b=b, β=β, r=0, t=t}, {a=0, α=α, b= 1/2 π, β=β, r=r, t=t}, {a=0, (3.10.1)
  α=α, b= -1/2 π, β=β, r=r, t=t}
VC > simplify( subs( {a=a, b=b, r=0, t=t, α=α, β=β}, Negw4 ) );
  16 α^2 + 16 β^2 (3.10.2)

```

$$\mathbf{VC} > \text{simplify}\left(\text{subs}\left(\left\{a=0, b=\frac{1}{2}\pi, r=r, t=t, \alpha=\alpha, \beta=\beta\right\}, \text{Negw4}\right)\right);$$

$$16\alpha^2 + 16\beta^2 \quad (3.10.3)$$

$$\mathbf{VC} > \text{simplify}\left(\text{subs}\left(\left\{a=0, b=-\frac{1}{2}\pi, r=r, t=t, \alpha=\alpha, \beta=\beta\right\}, \text{Negw4}\right)\right);$$

$$16\alpha^2 + 16\beta^2 \quad (3.10.4)$$

$\mathbf{> Negw34 := add(condw34[i]^2, i = 1..nops(condw34)) :$

### ▼ W1+W2+W3

$\mathbf{> condw123 := DGinfo(deltaW, "CoefficientSet") :$   
 $\mathbf{> solve(\{op(condw123), t \neq 0, Neg0 \neq 0, Negw1 \neq 0, Negw3 \neq 0, Negw12 \neq 0, Negw13 \neq 0, Negw23 \neq 0\})}$   
 $\{a=a, \alpha=0, b=b, \beta=0, r=r, t=t\} \quad (3.11.1)$

### ▼ W1+W2+W4

$\mathbf{> condw124 := DGinfo(evalDG(mu + ContractIndices(J, RearrangeIndices(ContractIndices(J, mu, [[1, 2]]), [2, 1, 3]), [[1, 1]])), "CoefficientSet") :$   
 $\mathbf{> solve(\{op(condw124), t \neq 0, Neg0 \neq 0, Negw1 \neq 0, Negw4 \neq 0, Negw12 \neq 0, Negw14 \neq 0, Negw24 \neq 0\}) ;}$

### ▼ W1+W3+W4

$\mathbf{> part1 := SymmetrizeIndices(Nw, [1, 2], "Symmetric") :$   
 $\mathbf{> condw134 := DGinfo(evalDG(part1 - ContractIndices(J, RearrangeIndices(ContractIndices(J, part1, [[1, 2]]), [2, 1, 3]), [[1, 1]])), "CoefficientSet") :$   
 $\mathbf{> use RealDomain in solve(\{op(condw134), t \neq 0, Neg0 \neq 0, Negw1 \neq 0, Negw3 \neq 0, Negw4 \neq 0, Negw13 \neq 0, Negw14 \neq 0, Negw34 \neq 0\}) end use}$

### ▼ W2+W3+W4

$\mathbf{> part1 := evalDG(Nw - ContractIndices(J, RearrangeIndices(ContractIndices(J, Nw, [[1, 2]]), [2, 1, 3]), [[1, 1]])) :$   
 $\mathbf{> condw234 := DGinfo(evalDG(part1 + RearrangeIndices(part1, [3, 1, 2]) + RearrangeIndices(part1, [2, 3, 1])), "CoefficientSet") :$   
 $\mathbf{> use RealDomain in solve(\{op(condw234), t \neq 0, Neg0 \neq 0, Negw3 \neq 0, Negw4 \neq 0, Negw23 \neq 0, Negw24 \neq 0, Negw34 \neq 0\}) end use}$

## ▼ A1.4

$\mathbf{> restart : with(DifferentialGeometry) : with(LieAlgebras) : with(Tensor) : with(Tools) : with(LinearAlgebra) :$   
 $\mathbf{> StructureEquations := [[LAI, LAj] = 2 * LAK, [LAI, LAK] = -2 * LAj, [LAj, LAK] = 2 * LAI, [LAI, ee] = ii, [LAI, ii] = -ee, [LAI, jj] = kk, [LAI, kk] = -jj, [LAj, ee] = jj, [LAj, ii] =$

$-kk, [LAj, jj] = -ee, [LAj, kk] = ii, [LAK, ee] = kk, [LAK, ii] = jj, [LAK, jj] = -ii, [LAK, kk] = -ee, [ee, ii] = -e + \epsilon * LAi, [ee, jj] = \epsilon * LAj, [ee, kk] = \epsilon * LAK, [ii, jj] = \epsilon * LAK, [ii, kk] = -\epsilon * LAj, [jj, kk] = e + \epsilon * LAi, [ee, e] = 3 \epsilon * ii, [ii, e] = -3 \epsilon * ee, [jj, e] = -3 \epsilon * kk, [kk, e] = 3 \epsilon * jj, [LAI, LAj, LAK, ee, ii, jj, kk, e, ie] :$

$L := LieAlgebraData(StructureEquations, VC);$

$$\begin{aligned}
 L := & [ [e1, e2] = 2 e3, [e1, e3] = -2 e2, [e1, e4] = e5, [e1, e5] = -e4, [e1, e6] = e7, [e1, e7] \\
 & = -e6, [e2, e3] = 2 e1, [e2, e4] = e6, [e2, e5] = -e7, [e2, e6] = -e4, [e2, e7] = e5, [e3, \\
 & e4] = e7, [e3, e5] = e6, [e3, e6] = -e5, [e3, e7] = -e4, [e4, e5] = e1 \epsilon - e8, [e4, e6] \\
 & = \epsilon e2, [e4, e7] = \epsilon e3, [e4, e8] = 3 \epsilon e5, [e5, e6] = \epsilon e3, [e5, e7] = -\epsilon e2, [e5, e8] = \\
 & -3 \epsilon e4, [e6, e7] = e1 \epsilon + e8, [e6, e8] = -3 \epsilon e7, [e7, e8] = 3 \epsilon e6 ]
 \end{aligned} \quad (4.1)$$

$> DGsetup(L, [e], [f]) :$

$> Query("Jacobi");$

$true$

(4.2)

$> g := evalDG(temp \cdot (f1 \&t f1 + f2 \&t f2 + f3 \&t f3) + r \cdot (f4 \&t f4 + f5 \&t f5 + f6 \&t f6 + f7 \&t f7) + t \cdot (f8 \&t f8 + f9 \&t f9)) ;$

$$g := temp f1 f1 + temp f2 f2 + temp f3 f3 + r f4 f4 + r f5 f5 + r f6 f6 + r f7 f7 + t f8 f8 + t f9 f9 \quad (4.3)$$

$> J0 := Matrix([ [0, 0, 0, 0, 0, 0, 0, 0, 0], [0, 0, 0, 0, 0, 0, 0, 0, 0], [0, 0, 0, 0, 0, 0, 0, 0, 0], [0, 0, 0, -\cos(a) \sin(b), -\sin(a) \sin(b), -\cos(b), 0, 0], [0, 0, 0, \cos(a) \sin(b), 0, \cos(b), -\sin(a) \sin(b), 0, 0], [0, 0, 0, \sin(a) \sin(b), -\cos(b), 0, \cos(a) \sin(b), 0, 0], [0, 0, 0, \cos(b), \sin(a) \sin(b), -\cos(a) \sin(b), 0, 0, 0], [0, 0, 0, 0, 0, 0, 0, -1], [0, 0, 0, 0, 0, 0, 0, 1, 0]]);$

$$J0 := \begin{bmatrix} 0 & 0 & 0 & 0 & 0 & 0 & 0 & 0 & 0 \\ 0 & 0 & 0 & 0 & 0 & 0 & 0 & 0 & 0 \\ 0 & 0 & 0 & 0 & 0 & 0 & 0 & 0 & 0 \\ 0 & 0 & 0 & 0 & -\cos(a) \sin(b) & -\sin(a) \sin(b) & -\cos(b) & 0 & 0 \\ 0 & 0 & 0 & \cos(a) \sin(b) & 0 & \cos(b) & -\sin(a) \sin(b) & 0 & 0 \\ 0 & 0 & 0 & \sin(a) \sin(b) & -\cos(b) & 0 & \cos(a) \sin(b) & 0 & 0 \\ 0 & 0 & 0 & \cos(b) & \sin(a) \sin(b) & -\cos(a) \sin(b) & 0 & 0 & 0 \\ 0 & 0 & 0 & 0 & 0 & 0 & 0 & 0 & -1 \\ 0 & 0 & 0 & 0 & 0 & 0 & 0 & 1 & 0 \end{bmatrix} \quad (4.4)$$

$> J := convert(J0, DGtensor, [{"con_bas", "cov_bas"}, [ ]]);$

$$\begin{aligned}
 J := & -\cos(a) \sin(b) e4 f5 - \sin(a) \sin(b) e4 f6 - \cos(b) e4 f7 + \cos(a) \sin(b) e5 f4 \\
 & + \cos(b) e5 f6 - \sin(a) \sin(b) e5 f7 + \sin(a) \sin(b) e6 f4 - \cos(b) e6 f5 \\
 & + \cos(a) \sin(b) e6 f7 + \cos(b) e7 f4 + \sin(a) \sin(b) e7 f5 - \cos(a) \sin(b) e7 f6 \\
 & - e8 f9 + e9 f8
 \end{aligned} \quad (4.5)$$

$> w := ContractIndices(J, g, [[1, 1]]);$

$$\begin{aligned}
 w := & \cos(a) \sin(b) r f4 f5 + \sin(a) \sin(b) r f4 f6 + \cos(b) r f4 f7 - \cos(a) \sin(b) r f5 f4 \\
 & - \cos(b) r f5 f6 + \sin(a) \sin(b) r f5 f7 - \sin(a) \sin(b) r f6 f4 + \cos(b) r f6 f5 \\
 & - \cos(a) \sin(b) r f6 f7 - \cos(b) r f7 f4 - \sin(a) \sin(b) r f7 f5 + \cos(a) \sin(b) r f7 f6 \\
 & + t f8 f9 - t f9 f8
 \end{aligned} \quad (4.6)$$



$$\begin{aligned}
& \text{> } W := \text{convert}(w, \text{DGform}); \\
& W := \cos(a) \sin(b) r f4 \wedge f5 + \sin(a) \sin(b) r f4 \wedge f6 + \cos(b) r f4 \wedge f7 \\
& \quad - \cos(b) r f5 \wedge f6 + \sin(a) \sin(b) r f5 \wedge f7 - \cos(a) \sin(b) r f6 \wedge f7 + t f8 \wedge f9
\end{aligned} \tag{4.7}$$

$$\begin{aligned}
& \text{> } \text{Nabla} := \text{Christoffel}(g) : \\
& \text{> } Nw := \text{RearrangeIndices}(\text{subs}(\{temp = 0\}, \text{CovariantDerivative}(w, \text{Nabla})), [2, 3, 1]) : \\
& \text{> } NJ := \text{DGsimplify}(\text{subs}(\{e1 = 0, e2 = 0, e3 = 0, f1 = 0, f2 = 0, f3 = 0\}, \text{TensorBrackets}(J, J, \\
& \quad \text{"Frolicher-Nijenhuis"}))) : \\
& \text{> } \text{delta}W := \text{HodgeStar}(g, \text{ExteriorDerivative}(\text{HodgeStar}(g, W))) : \\
& \text{> } Lee := \text{convert}\left(\text{evalDG}\left(-\frac{1}{2} \cdot \text{ContractIndices}(J, \text{HodgeStar}(g, \right. \right. \\
& \quad \left. \left. \text{ExteriorDerivative}(\text{HodgeStar}(g, W)))\right), [[1, 1]]\right), \text{DGform}\right); \\
& \quad \quad \quad Lee := \frac{t \cos(a) \sin(b)}{r} f9
\end{aligned} \tag{4.8}$$

$$\begin{aligned}
& \text{> } \text{part2} := \text{SymmetrizeIndices}(\text{evalDG}(g \&t \text{delta}W), [2, 3], \text{"SkewSymmetric"}) : \\
& \text{> } \text{part3} := \text{SymmetrizeIndices}(\text{RearrangeIndices}(\text{ContractIndices}(J, \\
& \quad \text{ContractIndices}(\text{evalDG}(g \&t \text{delta}W), J, [[3, 1]]), [[1, 2]]), [2, 1, 3]), [2, 3], \\
& \quad \text{"SkewSymmetric"}) : \\
& \text{> } \mu := \text{subs}\left(\{temp = 0\}, \text{evalDG}\left(Nw + \frac{1}{2} \cdot (\text{part2} - \text{part3})\right)\right) :
\end{aligned}$$

$$\begin{aligned}
& \text{0} \\
& \left[ \begin{aligned}
& \text{> } \text{cond0} := \text{DGinfo}(Nw, \text{"CoefficientSet"}) : \\
& \text{> } \text{sol0} := \text{solve}(\{op(\text{cond0}), r \neq 0, t \neq 0\}); \\
& \quad \quad \quad \text{sol0} := \\
& \text{> } \text{Neg0} := \text{add}(\text{cond0}[i]^2, i = 1 \dots \text{nops}(\text{cond0})) :
\end{aligned} \right.
\end{aligned} \tag{4.1.1}$$

$$\begin{aligned}
& \text{W1} \\
& \left[ \begin{aligned}
& \text{> } SNw := \text{SymmetrizeIndices}(Nw, [1, 2, 3], \text{"SkewSymmetric"}) : \\
& \text{> } \text{condw1} := \text{DGinfo}(\text{evalDG}(Nw - SNw), \text{"CoefficientSet"}) : \\
& \text{> } \text{solve}(\{op(\text{condw1}), t \neq 0, r \neq 0, \text{Neg0} \neq 0\}); \\
& \text{> } \text{Negw1} := \text{add}(\text{condw1}[i]^2, i = 1 \dots \text{nops}(\text{condw1})) :
\end{aligned} \right.
\end{aligned}$$

$$\begin{aligned}
& \text{W3} \\
& \left[ \begin{aligned}
& \text{> } \text{condw3} := \{op(\text{DGinfo}(\text{delta}W, \text{"CoefficientSet"})), op(\text{DGinfo}(NJ, \\
& \quad \text{"CoefficientSet"}))\} : \\
& \text{> } \text{solve}(\{op(\text{condw3}), r \neq 0, t \neq 0, \text{Neg0} \neq 0\}) \\
& \text{> } \text{Negw3} := \text{add}(\text{condw3}[i]^2, i = 1 \dots \text{nops}(\text{condw3})) :
\end{aligned} \right.
\end{aligned}$$

$$\begin{aligned}
& \text{W4} \\
& \left[ \begin{aligned}
& \text{> } \text{condw4} := \text{DGinfo}(\mu, \text{"CoefficientSet"}) : \\
& \text{> } \text{solve}(\{op(\text{condw4}), t \neq 0, r \neq 0, \text{Neg0} \neq 0\});
\end{aligned} \right.
\end{aligned}$$

$$\left\{a=0, b=\frac{1}{2}\pi, \varepsilon=\varepsilon, r=r, t=t\right\}, \left\{a=0, b=-\frac{1}{2}\pi, \varepsilon=\varepsilon, r=r, t=t\right\} \quad (4.4.1)$$

>  $Negw4 := add(condw4[i]^2, i=1..nops(condw4)) :$

### W1+W2

>  $condw12 := DGinfo(DGsimply(simplify(evalDG(Nw + RearrangeIndices(ContractIndices(J, ContractIndices(J, Nw, [[1, 1]]), [[1, 3]]), [3, 1, 2]))), "CoefficientSet")) :$

> **use RealDomain in** solve( $\{op(condw12), t \neq 0, r \neq 0, Neg0 \neq 0, Negw1 \neq 0\}$ ) **end use**

$$\left\{a=\frac{1}{2}\pi, b=b, \varepsilon=\varepsilon, r=r, t=6\varepsilon r\right\}, \left\{a=-\frac{1}{2}\pi, b=b, \varepsilon=\varepsilon, r=r, t=6\varepsilon r\right\}, \left\{a=a, b=0, \varepsilon=\varepsilon, r=r, t=6\varepsilon r\right\}, \left\{a=a, b=\pi, \varepsilon=\varepsilon, r=r, t=6\varepsilon r\right\}, \left\{a=\frac{1}{2}\pi, b=\frac{1}{2}\pi, \varepsilon=\frac{1}{6}\frac{t}{r}, r=r, t=t\right\}, \left\{a=\frac{1}{2}\pi, b=-\frac{1}{2}\pi, \varepsilon=\frac{1}{6}\frac{t}{r}, r=r, t=t\right\}, \left\{a=-\frac{1}{2}\pi, b=\frac{1}{2}\pi, \varepsilon=\frac{1}{6}\frac{t}{r}, r=r, t=t\right\}, \left\{a=-\frac{1}{2}\pi, b=-\frac{1}{2}\pi, \varepsilon=\frac{1}{6}\frac{t}{r}, r=r, t=t\right\} \quad (4.5.1)$$

>  $Negw12 := add(condw12[i]^2, i=1..nops(condw12)) :$

### W1+W3

>  $condw13 := \{op(DGinfo(deltaW, "CoefficientSet")), op(DGinfo(SymmetrizeIndices(evalDG(Nw - ContractIndices(J, RearrangeIndices(ContractIndices(J, Nw, [[1, 3]]), [3, 1, 2]), [[1, 1]])), [1, 3], "Symmetric"), "CoefficientSet"))\} :$

> **use RealDomain in** solve( $\{op(condw13), r \neq 0, t \neq 0, Neg0 \neq 0, Negw1 \neq 0, Negw3 \neq 0\}$ ) **end use;**

$$\left\{a=\frac{1}{2}\pi, b=b, \varepsilon=\varepsilon, r=r, t=3\varepsilon r\right\}, \left\{a=-\frac{1}{2}\pi, b=b, \varepsilon=\varepsilon, r=r, t=3\varepsilon r\right\}, \left\{a=a, b=0, \varepsilon=\varepsilon, r=r, t=3\varepsilon r\right\}, \left\{a=\frac{1}{2}\pi, b=\frac{1}{2}\pi, \varepsilon=\frac{1}{3}\frac{t}{r}, r=r, t=t\right\}, \left\{a=\frac{1}{2}\pi, b=-\frac{1}{2}\pi, \varepsilon=\frac{1}{3}\frac{t}{r}, r=r, t=t\right\}, \left\{a=-\frac{1}{2}\pi, b=\frac{1}{2}\pi, \varepsilon=\frac{1}{3}\frac{t}{r}, r=r, t=t\right\}, \left\{a=-\frac{1}{2}\pi, b=-\frac{1}{2}\pi, \varepsilon=\frac{1}{3}\frac{t}{r}, r=r, t=t\right\} \quad (4.6.1)$$

>  $Negw13 := add(condw13[i]^2, i=1..nops(condw13)) :$

>  $simplify\left(subs\left(\left\{a=\frac{1}{2}\pi, b=b, e=e, r=r, t=3\varepsilon r\right\}, Negw1\right), trig\right);$

$$\frac{5}{2}r^2(10e^2 - 24e\varepsilon + 16\varepsilon^2) \quad (4.6.2)$$

### W1+W4

>  $condw14 := DGinfo(SymmetrizeIndices(mu, [1, 2], "Symmetric"), "CoefficientSet") :$

```

[> solve( {op(condw14), r ≠ 0, t ≠ 0, Neg0 ≠ 0, Negw1 ≠ 0, Negw4 ≠ 0});
[> Negw14 := add( condw14[i]2, i = 1 ..nops(condw14) ) :

```

## W2+W3

```

[> part1 := evalDG(Nw-ContractIndices(J, RearrangeIndices( ContractIndices(J, Nw, [[1,
2]]), [2, 1, 3]), [[1, 1]])) :
[> condw23 := {op(DGinfo(deltaW, "CoefficientSet")), op(DGinfo(evalDG(part1
+ RearrangeIndices(part1, [3, 1, 2]) + RearrangeIndices(part1, [2, 3, 1])),
"CoefficientSet"))} :
[> solve( {op(condw23), r ≠ 0, t ≠ 0, Neg0 ≠ 0, Negw3 ≠ 0});
{a =  $\frac{1}{2} \pi$ , b = b, ε = ε, r = r, t = -6 ε r}, {a = - $\frac{1}{2} \pi$ , b = b, ε = ε, r = r, t = -6 ε r}, {a = a, (4.8.1)
b = 0, ε = ε, r = r, t = -6 ε r}, {a =  $\frac{1}{2} \pi$ , b =  $\frac{1}{2} \pi$ , ε = - $\frac{1}{6} \frac{t}{r}$ , r = r, t = t}, {a =  $\frac{1}{2} \pi$ ,
b = - $\frac{1}{2} \pi$ , ε = - $\frac{1}{6} \frac{t}{r}$ , r = r, t = t}, {a = - $\frac{1}{2} \pi$ , b =  $\frac{1}{2} \pi$ , ε = - $\frac{1}{6} \frac{t}{r}$ , r = r, t = t}, {a
= - $\frac{1}{2} \pi$ , b = - $\frac{1}{2} \pi$ , ε = - $\frac{1}{6} \frac{t}{r}$ , r = r, t = t}
[> Negw23 := add( condw23[i]2, i = 1 ..nops(condw23) ) :

```

## W2+W4

```

[> condw24 := DGinfo(evalDG(ExteriorDerivative(W) - W&w Lee), "CoefficientSet") :
[> solve( {op(condw24), r ≠ 0, t ≠ 0, Neg0 ≠ 0, Negw2 ≠ 0, Negw4 ≠ 0});
[> Negw24 := add( condw24[i]2, i = 1 ..nops(condw24) ) :

```

## W3+W4

```

[> condw34 := DGinfo(NJ, "CoefficientSet") :
[> solve( {op(condw34), r ≠ 0, t ≠ 0, Neg0 ≠ 0, Negw3 ≠ 0, Negw4 ≠ 0})
[> Negw34 := add( condw34[i]2, i = 1 ..nops(condw34) ) :

```

## W1+W2+W3

```

[> condw123 := DGinfo(deltaW, "CoefficientSet") :
[> solve( {op(condw123), r ≠ 0, t ≠ 0, Neg0 ≠ 0, Negw1 ≠ 0, Negw3 ≠ 0, Negw12 ≠ 0,
Negw13 ≠ 0, Negw23 ≠ 0})
{a =  $\frac{1}{2} \pi$ , b = b, ε = ε, r = r, t = t}, {a = - $\frac{1}{2} \pi$ , b = b, ε = ε, r = r, t = t}, {a = a, b = 0, ε (4.11.1)
= ε, r = r, t = t}
VC > simplify( subs( {a =  $\frac{1}{2} \pi$ , b = b, r = r, t = t, ε = ε}, {Negw12, Negw13,
Negw23} ) )
{4 (3 ε r - t)2, 4 (6 ε r - t)2, 4 (6 ε r + t)2} (4.11.2)

```

## W1+W2+W4

```
> condw124 := DGinfo(evalDG(mu + ContractIndices(J,
  RearrangeIndices(ContractIndices(J, mu, [[1, 2]]), [2, 1, 3]), [[1, 1]])),
  "CoefficientSet") :
=
> solve({op(condw124), r ≠ 0, t ≠ 0, Neg0 ≠ 0, Negw1 ≠ 0, Negw4 ≠ 0, Negw12 ≠ 0,
  Negw14 ≠ 0, Negw24 ≠ 0});
      {a = a, b = b, ε = ε, r = r, t = 6 ε r} (4.12.1)
```

```
VC > simplify(subs({a = a, b = b, ε = ε, r = r, t = 6 ε r}, {Negw12, Negw14,
  Negw24}))
{9 ε2 r2 (cos(b)2 cos(a)2 - cos(a)2 + 1), 36 ε2 r2 (cos(b)4 cos(a)4 - cos(b)4 cos(a)2
- 2 cos(b)2 cos(a)4 + 6 cos(b)2 cos(a)2 + cos(a)4 - cos(b)2 - 5 cos(a)2 + 4),
- 144 cos(a)2 ε2 r2 (cos(b)2 - 1)}
```

## W1+W3+W4

```
> part1 := SymmetrizeIndices(Nw, [1, 2], "Symmetric") :
> condw134 := DGinfo(evalDG(part1 - ContractIndices(J,
  RearrangeIndices(ContractIndices(J, part1, [[1, 2]]), [2, 1, 3]), [[1, 1]])),
  "CoefficientSet") :
=
> use RealDomain in solve({op(condw134), r ≠ 0, t ≠ 0, Neg0 ≠ 0, Negw1 ≠ 0, Negw3
  ≠ 0, Negw4 ≠ 0, Negw13 ≠ 0, Negw14 ≠ 0, Negw34 ≠ 0}) end use
      {a = a, b = b, ε = ε, r = r, t = 3 ε r} (4.13.1)
```

```
> eqq := DGinfo(subs({temp = 0}, SymmetrizeIndices(ContractIndices(NJ, g, [[1, 1]]),
  [1, 3], "Symmetric")), "CoefficientSet");
eqq := {0, -2 (cos(a)2 cos(b)2 - cos(a)2 + 1) (3 ε r - t), 2 (cos(a)2 cos(b)2
- cos(a)2 + 1) (3 ε r - t), -2 cos(b) (3 ε r - t), 2 cos(b) (3 ε r - t),
-2 sin(a) sin(b) (3 ε r - t), 2 sin(a) sin(b) (3 ε r - t),
-2 cos(a) sin(b) cos(b) (3 ε r - t), 2 cos(a) sin(b) cos(b) (3 ε r - t),
-2 cos(a) sin(b)2 sin(a) (3 ε r - t), 2 cos(a) sin(b)2 sin(a) (3 ε r - t)}
```

```
> solve(eqq);
{a = a, b = b, ε = ε, r = r, t = 3 ε r}, {a = 0, b = 1/2 π, ε = ε, r = r, t = t}, {a = 0, b =
- 1/2 π, ε = ε, r = r, t = t}, {a = π, b = 1/2 π, ε = ε, r = r, t = t}, {a = π, b = - 1/2 π, ε
= ε, r = r, t = t} (4.13.3)
```

## W2+W3+W4

```
> part1 := evalDG(Nw - ContractIndices(J, RearrangeIndices(ContractIndices(J, Nw,
  [[1, 2]]), [2, 1, 3]), [[1, 1]])) :
=
> condw234 := DGinfo(evalDG(part1 + RearrangeIndices(part1, [3, 1, 2])
  + RearrangeIndices(part1, [2, 3, 1])), "CoefficientSet") :
```

```

> use RealDomain in solve( {op(condw234), r ≠ 0, t ≠ 0, Neg0 ≠ 0, Negw3 ≠ 0, Negw4
  ≠ 0, Negw23 ≠ 0, Negw24 ≠ 0, Negw34 ≠ 0} ) end use
{a=a, b=b, r=r, t=-6 r ε, ε=ε}, {a=0, b= 1/2 π, r=r, t=t, ε=ε}, {a=0, b=
- 1/2 π, r=r, t=t, ε=ε}, {a=π, b= 1/2 π, r=r, t=t, ε=ε}, {a=π, b=- 1/2 π, r=r,
t=t, ε=ε}
(4.14.1)

> simplify( subs( {a=a, b=b, r=r, t=-6 r ε, ε=ε}, {Negw23, Negw24, Negw34} ), trig);
{36 r^2 ε^2 (cos(b)^4 cos(a)^4 - cos(b)^4 cos(a)^2 - 2 cos(b)^2 cos(a)^4 + 6 cos(a)^2 cos(b)^2
+ cos(a)^4 - cos(b)^2 - 5 cos(a)^2 + 4), 144 ε^2 cos(a)^2 sin(b)^2,
576 cos(b)^2 cos(a)^2 ε^2 + 64 cos(a)^2 cos(b)^2 - 576 cos(a)^2 ε^2 - 64 cos(a)^2
+ 584 ε^2 + 64}
(4.14.2)

```

## A2.1

```

> restart : with(DifferentialGeometry) : with(LieAlgebras) : with(Tensor) : with(Tools) :
  with(LinearAlgebra) :
> StructureEquations := [[i1, j1] = k1, [i1, k1] = -j1, [j1, k1] = i1, [i2, j2] = k2, [i2, k2] = -j2,
  [j2, k2] = i2], [i1, j1, k1, i2, j2, k2] :
> L := LieAlgebraData(StructureEquations, A21) :
> DGsetup(L, [e], [f]) :
> W := evalDG(f1 &w f4 + f2 &w f5 + f3 &w f6)
  W := f1 ∧ f4 + f2 ∧ f5 + f3 ∧ f6
(5.1)

> J0 := Matrix( [[ [r, 0, 0, - (1+r^2)/t, 0, 0], [0, r, 0, 0, - (1+r^2)/t, 0], [0, 0, r, 0, 0,
  - (1+r^2)/t], [t, 0, 0, -r, 0, 0], [0, t, 0, 0, -r, 0], [0, 0, t, 0, 0, -r]] ] )

J0 :=
⎡  r  0  0  - (r^2+1)/t  0  0
⎢  0  r  0  0  - (r^2+1)/t  0
⎢  0  0  r  0  0  - (r^2+1)/t
⎢  t  0  0  -r  0  0
⎢  0  t  0  0  -r  0
⎢  0  0  t  0  0  -r
(5.2)

> J := convert(J0, DGtensor, [[ "con_bas", "cov_bas"], [ ]]);
J := r e1 f1 - (r^2+1)/t e1 f4 + r e2 f2 - (r^2+1)/t e2 f5 + r e3 f3 - (r^2+1)/t e3 f6 + t e4 f1
- r e4 f4 + t e5 f2 - r e5 f5 + t e6 f3 - r e6 f6
(5.3)

```

$$\begin{aligned} & \text{w} := \text{convert}(W, \text{DGtensor}); \\ & \text{w} := f1 f4 + f2 f5 + f3 f6 - f4 f1 - f5 f2 - f6 f3 \end{aligned} \quad (5.4)$$

$$\begin{aligned} & \text{g} := \text{ContractIndices}(J, \text{w}, [[1, 2]]); \\ & \text{g} := t f1 f1 - r f1 f4 + t f2 f2 - r f2 f5 + t f3 f3 - r f3 f6 - r f4 f1 + \frac{r^2 + 1}{t} f4 f4 - r f5 f2 \\ & \quad + \frac{r^2 + 1}{t} f5 f5 - r f6 f3 + \frac{r^2 + 1}{t} f6 f6 \end{aligned} \quad (5.5)$$

$$\begin{aligned} & \text{Nabla} := \text{Christoffel}(\text{g}) : \\ & \text{Nw} := \text{RearrangeIndices}(\text{CovariantDerivative}(\text{w}, \text{Nabla}), [2, 3, 1]) : \\ & \text{NJ} := \text{TensorBrackets}(J, J, \text{"Frolicher-Nijenhuis"}) : \\ & \text{deltaW} := \text{DGzero}(\text{"form"}, 1); \\ & \text{deltaW} := 0 f1 \end{aligned} \quad (5.6)$$

$$\begin{aligned} & \text{Lee} := \text{convert}\left(\text{evalDG}\left(-\frac{1}{2} \cdot \text{ContractIndices}(J, \text{deltaW}, [[1, 1]])\right), \text{DGform}\right); \\ & \text{Lee} := 0 f1 \end{aligned} \quad (5.7)$$

$$\begin{aligned} & \text{part2} := \text{SymmetrizeIndices}(\text{evalDG}(\text{g} \& \text{t deltaW}), [2, 3], \text{"SkewSymmetric"}) : \\ & \text{part3} := \text{SymmetrizeIndices}(\text{RearrangeIndices}(\text{ContractIndices}(J, \\ & \quad \text{ContractIndices}(\text{evalDG}(\text{g} \& \text{t deltaW}), J, [[3, 1]]), [[1, 2]]), [2, 1, 3]), [2, 3], \\ & \quad \text{"SkewSymmetric"}) : \\ & \text{mu} := \text{evalDG}\left(\text{Nw} + \frac{1}{2} \cdot (\text{part2} - \text{part3})\right) : \end{aligned}$$

$$\begin{aligned} & \text{cond0} := \text{DGinfo}(\text{Nw}, \text{"CoefficientSet"}) : \\ & \text{sol0} := \text{solve}(\{\text{op}(\text{cond0}), t \neq 0\}); \\ & \text{sol0} := \\ & \text{Neg0} := \text{add}(\text{cond0}[i]^2, i = 1 \dots \text{nops}(\text{cond0})) : \end{aligned} \quad (5.1.1)$$

$$\begin{aligned} & \text{SNw} := \text{SymmetrizeIndices}(\text{Nw}, [1, 2, 3], \text{"SkewSymmetric"}) : \\ & \text{condw1} := \text{DGinfo}(\text{evalDG}(\text{Nw} - \text{SNw}), \text{"CoefficientSet"}) : \\ & \text{solve}(\{\text{op}(\text{condw1}), t \neq 0, \text{Neg0} \neq 0\}); \\ & \quad \{r = \text{RootOf}(3 \_Z^2 - 1), t = 2 \text{RootOf}(3 \_Z^2 - 1)\} \\ & \text{Negw1} := \text{add}(\text{condw1}[i]^2, i = 1 \dots \text{nops}(\text{condw1})) : \end{aligned} \quad (5.2.1)$$

$$\begin{aligned} & \text{condw3} := \{\text{op}(\text{DGinfo}(\text{deltaW}, \text{"CoefficientSet"})), \text{op}(\text{DGinfo}(\text{NJ}, \\ & \quad \text{"CoefficientSet"}))\} : \\ & \text{solve}(\{\text{op}(\text{condw3}), t \neq 0, \text{Neg0} \neq 0\}) \\ & \quad \{r = \text{RootOf}(\_Z^2 + 1), t = 2 \text{RootOf}(\_Z^2 + 1)\} \\ & \text{Negw3} := \text{add}(\text{condw3}[i]^2, i = 1 \dots \text{nops}(\text{condw3})) : \end{aligned} \quad (5.3.1)$$

#### W4

```
[> condw4 := DGinfo(mu, "CoefficientSet") :  
[> solve( {op(condw4), t ≠ 0, Neg0 ≠ 0});  
[> Negw4 := add( condw4[i]2, i = 1 ..nops(condw4) ) :
```

#### W1+W2

```
[> condw12 := DGinfo( DGsimplify( simplify( evalDG( Nw  
+ RearrangeIndices( ContractIndices(J, ContractIndices(J, Nw, [[1, 1]]), [[1,  
3]]), [3, 1, 2]) ) ) ), "CoefficientSet") :  
[> use RealDomain in solve( {op(condw12), t ≠ 0, Neg0 ≠ 0, Negw1 ≠ 0, Negw2 ≠ 0})  
end use  
[> Negw12 := add( condw12[i]2, i = 1 ..nops(condw12) ) :
```

#### W1+W3

```
[> condw13 := { op( DGinfo( deltaW, "CoefficientSet" ) ),  
op( DGinfo( SymmetrizeIndices( evalDG( Nw - ContractIndices(J,  
RearrangeIndices( ContractIndices(J, Nw, [[1, 3]]), [3, 1, 2]) ), [[1, 1]] ) ), [1, 3],  
"Symmetric"), "CoefficientSet" ) } :  
[> use RealDomain in solve( {op(condw13), t ≠ 0, Neg0 ≠ 0, Negw1 ≠ 0, Negw3 ≠ 0})  
end use;  
{ r=r, t ≠ 0, t ≠ RootOf( 5 r2 _Z4 + ( -10 r3 - 2 r ) _Z3 + ( 10 r4 + 4 r2 + 2 ) _Z2 + ( (5.6.1)  
- 10 r5 - 12 r3 - 2 r ) _Z + 5 r6 + 10 r4 + 5 r2 ), t ≠ RootOf( 9 r2 _Z4 + ( -18 r3  
- 6 r ) _Z3 + ( 18 r4 + 12 r2 + 2 ) _Z2 + ( -18 r5 - 24 r3 - 6 r ) _Z + 9 r6 + 18 r4  
+ 9 r2 ), t ≠ RootOf( _Z8 - 4 r _Z7 + 4 r2 _Z6 + ( r4 + 2 r2 + 1 ) _Z4 + ( 4 r6 + 8 r4  
+ 4 r2 ) _Z2 + ( -4 r7 - 12 r5 - 12 r3 - 4 r ) _Z + r8 + 4 r6 + 6 r4 + 4 r2 + 1 ) }  
[> Negw13 := add( condw13[i]2, i = 1 ..nops(condw13) ) :
```

#### W1+W4

```
[> condw14 := DGinfo( SymmetrizeIndices(mu, [1, 2], "Symmetric"), "CoefficientSet") :  
[> solve( {op(condw14), t ≠ 0, Neg0 ≠ 0, Negw1 ≠ 0, Negw4 ≠ 0});  
[> Negw14 := add( condw14[i]2, i = 1 ..nops(condw14) ) :
```

#### W2+W3

```
[> part1 := evalDG( Nw - ContractIndices(J, RearrangeIndices( ContractIndices(J, Nw, [[1,  
2]]), [2, 1, 3]), [[1, 1]] ) ) :  
[> condw23 := { op( DGinfo( deltaW, "CoefficientSet" ) ), op( DGinfo( evalDG( part1  
+ RearrangeIndices( part1, [3, 1, 2] ) + RearrangeIndices( part1, [2, 3, 1] ) ),  
"CoefficientSet" ) } :  
[> solve( {op(condw23), t ≠ 0, Neg0 ≠ 0, Negw2 ≠ 0, Negw3 ≠ 0});  
[> Negw23 := add( condw23[i]2, i = 1 ..nops(condw23) ) :
```

## W2+W4

```
[> condw24 := DGinfo(evalDG(ExteriorDerivative(W) - W &w Lee), "CoefficientSet") :  
[> solve( {op(condw24), t ≠ 0, Neg0 ≠ 0, Negw2 ≠ 0, Negw4 ≠ 0});  
[> Negw24 := add( condw24[i]^2, i = 1 ..nops(condw24)) :
```

## W3+W4

```
[> condw34 := DGinfo(NJ, "CoefficientSet") :  
[> solve( {op(condw34), t ≠ 0, Neg0 ≠ 0, Negw3 ≠ 0, Negw4 ≠ 0})  
[> Negw34 := add( condw34[i]^2, i = 1 ..nops(condw34)) :
```

## W1+W2+W3

```
[> condw123 := DGinfo(deltaW, "CoefficientSet");  
                                condw123 := {0} (5.11.1)  
[> solve( {op(condw123), t ≠ 0, Neg0 ≠ 0, Negw1 ≠ 0, Negw3 ≠ 0, Negw12 ≠ 0, Negw13  
          ≠ 0, Negw23 ≠ 0})
```

## W1+W2+W4

```
[> condw124 := DGinfo(evalDG(mu + ContractIndices(J,  
    RearrangeIndices(ContractIndices(J, mu, [[1, 2]]), [2, 1, 3]), [[1, 1]])),  
    "CoefficientSet") :  
[> solve( {op(condw124), t ≠ 0, Neg0 ≠ 0, Negw1 ≠ 0, Negw4 ≠ 0, Negw12 ≠ 0, Negw14  
          ≠ 0, Negw24 ≠ 0});
```

## W1+W3+W4

```
[> part1 := SymmetrizeIndices(Nw, [1, 2], "Symmetric") :  
[> condw134 := DGinfo(evalDG(part1 - ContractIndices(J,  
    RearrangeIndices(ContractIndices(J, part1, [[1, 2]]), [2, 1, 3]), [[1, 1]])),  
    "CoefficientSet") :  
[> use RealDomain in solve( {op(condw134), t ≠ 0, Neg0 ≠ 0, Negw1 ≠ 0, Negw3 ≠ 0,  
    Negw4 ≠ 0, Negw13 ≠ 0, Negw14 ≠ 0, Negw34 ≠ 0}) end use
```

## W2+W3+W4

```
[> part1 := evalDG(Nw - ContractIndices(J, RearrangeIndices(ContractIndices(J, Nw,  
    [[1, 2]]), [2, 1, 3]), [[1, 1]])) :  
[> condw234 := DGinfo(evalDG(part1 + RearrangeIndices(part1, [3, 1, 2])  
    + RearrangeIndices(part1, [2, 3, 1])), "CoefficientSet") :  
[> use RealDomain in solve( {op(condw234), t ≠ 0, Neg0 ≠ 0, Negw3 ≠ 0, Negw4 ≠ 0,  
    Negw23 ≠ 0, Negw24 ≠ 0, Negw34 ≠ 0}) end use
```

## A2.2

```
[> restart : with(DifferentialGeometry) : with(LieAlgebras) : with(Tensor) : with(Tools) :  
    with(LinearAlgebra) :  
[> StructureEquations := [[i1, j1] = k1, [i1, k1] = -j1, [j1, k1] = i1, [i1, j2] = k2, [i1, k2] = -j2,
```



$[j1, k2] = i2, [i2, j1] = k2, [i2, k1] = -j2, [j2, k1] = i2, [i2, j2] = -k1, [i2, k2] = j1, [j2, k2] = -i1, [i1, j1, k1, i2, j2, k2] :$

>  $L := \text{LieAlgebraData}(\text{StructureEquations}, A22) :$

>  $\text{DGsetup}(L, [e], [f]) :$

>  $W := \text{evalDG}(f1 \&w f4 + f2 \&w f5 + f3 \&w f6)$

$$W := f1 \wedge f4 + f2 \wedge f5 + f3 \wedge f6$$

(6.1)

>  $J0 := \text{Matrix}\left(\left[\left[\begin{matrix} r & 0 & 0 & -\frac{(1+r^2)}{t} & 0 & 0 \end{matrix}\right], \left[\begin{matrix} 0 & r & 0 & 0 & -\frac{(1+r^2)}{t} & 0 \end{matrix}\right], \left[\begin{matrix} 0 & 0 & r & 0 & 0 & 0 \end{matrix}\right], \right.\right.$

$\left.\left[-\frac{(1+r^2)}{t}\right], \left[\begin{matrix} t & 0 & 0 & -r & 0 & 0 \end{matrix}\right], \left[\begin{matrix} 0 & t & 0 & 0 & -r & 0 \end{matrix}\right], \left[\begin{matrix} 0 & 0 & t & 0 & 0 & -r \end{matrix}\right]\right]$

$$J0 := \begin{bmatrix} r & 0 & 0 & -\frac{r^2+1}{t} & 0 & 0 \\ 0 & r & 0 & 0 & -\frac{r^2+1}{t} & 0 \\ 0 & 0 & r & 0 & 0 & -\frac{r^2+1}{t} \\ t & 0 & 0 & -r & 0 & 0 \\ 0 & t & 0 & 0 & -r & 0 \\ 0 & 0 & t & 0 & 0 & -r \end{bmatrix}$$

(6.2)

>  $J := \text{convert}(J0, \text{DGtensor}, [[\text{"con\_bas"}, \text{"cov\_bas"}], [ ]]);$

$$J := r e1 f1 - \frac{r^2+1}{t} e1 f4 + r e2 f2 - \frac{r^2+1}{t} e2 f5 + r e3 f3 - \frac{r^2+1}{t} e3 f6 + t e4 f1 - r e4 f4 + t e5 f2 - r e5 f5 + t e6 f3 - r e6 f6$$

(6.3)

>  $w := \text{convert}(W, \text{DGtensor});$

$$w := f1 f4 + f2 f5 + f3 f6 - f4 f1 - f5 f2 - f6 f3$$

(6.4)

>  $g := \text{ContractIndices}(J, w, [[1, 2]]);$

$$g := t f1 f1 - r f1 f4 + t f2 f2 - r f2 f5 + t f3 f3 - r f3 f6 - r f4 f1 + \frac{r^2+1}{t} f4 f4 - r f5 f2 + \frac{r^2+1}{t} f5 f5 - r f6 f3 + \frac{r^2+1}{t} f6 f6$$

(6.5)

>  $\text{Nabla} := \text{Christoffel}(g) :$

>  $Nw := \text{RearrangeIndices}(\text{CovariantDerivative}(w, \text{Nabla}), [2, 3, 1]) :$

>  $NJ := \text{TensorBrackets}(J, J, \text{"Frolicher-Nijenhuis"}) :$

>  $\text{delta}W := \text{DGzero}(\text{"form"}, 1);$

$$\text{delta}W := 0 f1$$

(6.6)

>  $\text{Lee} := \text{convert}\left(\text{evalDG}\left(-\frac{1}{2} \cdot \text{ContractIndices}(J, \text{delta}W, [[1, 1]])\right), \text{DGform}\right);$

$$\text{Lee} := 0 f1$$

(6.7)

>  $\text{part2} := \text{SymmetrizeIndices}(\text{evalDG}(g \&t \text{delta}W), [2, 3], \text{"SkewSymmetric"}) :$

>  $\text{part3} := \text{SymmetrizeIndices}(\text{RearrangeIndices}(\text{ContractIndices}(J, \text{ContractIndices}(\text{evalDG}(g \&t \text{delta}W), J, [[3, 1]]), [[1, 2]]), [2, 1, 3]), [2, 3],$

$$\begin{aligned}
& \text{"SkewSymmetric") :} \\
& \text{> mu := evalDG}\left(Nw + \frac{1}{2} \cdot (part2 - part3)\right) : \\
& \text{> DGinfo(NJ, "CoefficientSet")} \\
& \left\{ -4 \, t \, r, 4 \, t \, r, -\frac{2 \left( r^4 + 3 \, r^2 \, t^2 + 2 \, r^2 - t^2 + 1 \right)}{t^2}, \frac{2 \left( r^4 + 3 \, r^2 \, t^2 + 2 \, r^2 - t^2 + 1 \right)}{t^2}, -2 \, r^2 \right. \\
& \quad \left. + 2 \, t^2 - 2, 2 \, r^2 - 2 \, t^2 + 2 \right\}
\end{aligned} \tag{6.8}$$

**0**

$$\begin{aligned}
& \text{> cond0 := DGinfo(Nw, "CoefficientSet") :} \\
& \text{> sol0 := solve( \{op(cond0), t \neq 0\} );} \\
& \quad \text{sol0 :=} \\
& \text{> Neg0 := add( cond0[i]^2, i = 1 ..nops( cond0) ) :}
\end{aligned} \tag{6.1.1}$$

**W1**

$$\begin{aligned}
& \text{> SNw := SymmetrizeIndices(Nw, [1, 2, 3], "SkewSymmetric") :} \\
& \text{> condw1 := DGinfo(evalDG(Nw - SNw), "CoefficientSet") :} \\
& \text{> solve( \{op(condw1), t \neq 0, Neg0 \neq 0\} );} \\
& \quad \{r=0, t=RootOf(3 \_Z^2 + 1)\} \\
& \text{> Negw1 := add( condw1[i]^2, i = 1 ..nops( condw1) ) :}
\end{aligned} \tag{6.2.1}$$

**W3**

$$\begin{aligned}
& \text{> condw3 := \{op(DGinfo(deltaW, "CoefficientSet")), op(DGinfo(NJ,} \\
& \quad \text{"CoefficientSet"))\} :} \\
& \text{> solve( \{op(condw3), t \neq 0, Neg0 \neq 0\} )} \\
& \quad \{r=0, t=1\}, \{r=0, t=-1\} \\
& \text{> Negw3 := add( condw3[i]^2, i = 1 ..nops( condw3) ) :}
\end{aligned} \tag{6.3.1}$$

**W4**

$$\begin{aligned}
& \text{> condw4 := DGinfo(mu, "CoefficientSet") :} \\
& \text{> solve( \{op(condw4), t \neq 0, Neg0 \neq 0\} );} \\
& \text{> Negw4 := add( condw4[i]^2, i = 1 ..nops( condw4) ) :}
\end{aligned}$$

**W1+W2**

$$\begin{aligned}
& \text{> condw12 := DGinfo(DGsimplify(simplify(evalDG(Nw} \\
& \quad \text{+ RearrangeIndices(ContractIndices(J, ContractIndices(J, Nw, [[1, 1]]), [[1,} \\
& \quad \text{3]]), [3, 1, 2]))), "CoefficientSet") :} \\
& \text{> use RealDomain in solve( \{op(condw12), t \neq 0, Neg0 \neq 0, Negw1 \neq 0, Negw2 \neq 0\} )} \\
& \quad \text{end use}
\end{aligned}$$

```

[> Negw12 := add(condw12[i]2, i = 1 ..nops(condw12)) :

```

### ▼ W1+W3

```

[> condw13 := {op(DGinfo(deltaW, "CoefficientSet")),
  op(DGinfo(SymmetrizeIndices(evalDG(Nw-ContractIndices(J,
  RearrangeIndices(ContractIndices(J, Nw, [[1, 3]]), [3, 1, 2]), [[1, 1]])), [1, 3],
  "Symmetric"), "CoefficientSet"))} :
[> use RealDomain in solve({op(condw13), t ≠ 0, Neg0 ≠ 0, Negw1 ≠ 0, Negw3 ≠ 0})
  end use;
[> Negw13 := add(condw13[i]2, i = 1 ..nops(condw13)) :

```

### ▼ W1+W4

```

[> condw14 := DGinfo(SymmetrizeIndices(mu, [1, 2], "Symmetric"), "CoefficientSet") :
[> solve({op(condw14), t ≠ 0, Neg0 ≠ 0, Negw1 ≠ 0, Negw4 ≠ 0});
[> Negw14 := add(condw14[i]2, i = 1 ..nops(condw14)) :

```

### ▼ W2+W3

```

[> part1 := evalDG(Nw-ContractIndices(J, RearrangeIndices(ContractIndices(J, Nw, [[1,
  2]]), [2, 1, 3]), [[1, 1]])) :
[> condw23 := {op(DGinfo(deltaW, "CoefficientSet")), op(DGinfo(evalDG(part1
  + RearrangeIndices(part1, [3, 1, 2]) + RearrangeIndices(part1, [2, 3, 1])),
  "CoefficientSet"))} :
[> solve({op(condw23), t ≠ 0, Neg0 ≠ 0, Negw2 ≠ 0, Negw3 ≠ 0});
[> Negw23 := add(condw23[i]2, i = 1 ..nops(condw23)) :

```

### ▼ W2+W4

```

[> condw24 := DGinfo(evalDG(ExteriorDerivative(W) - W&w Lee), "CoefficientSet") :
[> solve({op(condw24), t ≠ 0, Neg0 ≠ 0, Negw2 ≠ 0, Negw4 ≠ 0});
[> Negw24 := add(condw24[i]2, i = 1 ..nops(condw24)) :

```

### ▼ W3+W4

```

[> condw34 := DGinfo(NJ, "CoefficientSet") :
[> solve({op(condw34), t ≠ 0});
  {r=0, t=1}, {r=0, t=-1} (6.10.1)
[> Negw34 := add(condw34[i]2, i = 1 ..nops(condw34)) :

```

### ▼ W1+W2+W3

```

[> condw123 := DGinfo(deltaW, "CoefficientSet") :
[> solve({op(condw123), t ≠ 0, Neg0 ≠ 0, Negw1 ≠ 0, Negw3 ≠ 0, Negw12 ≠ 0, Negw13
  ≠ 0, Negw23 ≠ 0})

```

### ▼ W1+W2+W4

```

> condw124 := DGinfo(evalDG(mu + ContractIndices(J,
  RearrangeIndices(ContractIndices(J, mu, [[1, 2]]), [2, 1, 3]), [[1, 1]])),
  "CoefficientSet") :
> solve({op(condw124), t ≠ 0, Neg0 ≠ 0, Negw1 ≠ 0, Negw4 ≠ 0, Negw12 ≠ 0, Negw14
  ≠ 0, Negw24 ≠ 0});

```

### W1+W3+W4

```

> part1 := SymmetrizeIndices(Nw, [1, 2], "Symmetric") :
> condw134 := DGinfo(evalDG(part1 - ContractIndices(J,
  RearrangeIndices(ContractIndices(J, part1, [[1, 2]]), [2, 1, 3]), [[1, 1]])),
  "CoefficientSet") :
> use RealDomain in solve({op(condw134), t ≠ 0, Neg0 ≠ 0, Negw1 ≠ 0, Negw3 ≠ 0,
  Negw4 ≠ 0, Negw13 ≠ 0, Negw14 ≠ 0, Negw34 ≠ 0}) end use

```

### W2+W3+W4

```

> part1 := evalDG(Nw - ContractIndices(J, RearrangeIndices(ContractIndices(J, Nw,
  [[1, 2]]), [2, 1, 3]), [[1, 1]])) :
> condw234 := DGinfo(evalDG(part1 + RearrangeIndices(part1, [3, 1, 2])
  + RearrangeIndices(part1, [2, 3, 1])), "CoefficientSet") :
> use RealDomain in solve({op(condw234), t ≠ 0, Neg0 ≠ 0, Negw3 ≠ 0, Negw4 ≠ 0,
  Negw23 ≠ 0, Negw24 ≠ 0, Negw34 ≠ 0}) end use

```

## A2.3

```

> restart : with(DifferentialGeometry) : with(LieAlgebras) : with(Tensor) : with(Tools) :
  with(LinearAlgebra) :
> StructureEquations := [[i1, j1] = k1, [i1, k1] = -j1, [j1, k1] = i1, [i1, j2] = k2, [i1, k2] = -j2,
  [j1, k2] = i2, [i2, j1] = k2, [i2, k1] = -j2, [j2, k1] = i2], [i1, j1, k1, i2, j2, k2] :
> L := LieAlgebraData(StructureEquations, A23) :
> DGsetup(L, [e], [f]) :
> W := evalDG(f1 &w f4 + f2 &w f5 + f3 &w f6)
      W:=f1 ∧ f4 + f2 ∧ f5 + f3 ∧ f6

```

(7.1)

```

> J0 := Matrix([[r, 0, 0, - (1 + r^2)/t, 0, 0], [0, r, 0, 0, - (1 + r^2)/t, 0], [0, 0, r, 0, 0, 0,
  - (1 + r^2)/t], [t, 0, 0, -r, 0, 0], [0, t, 0, 0, -r, 0], [0, 0, t, 0, 0, -r]])

```

(7.2)

$$J0 := \begin{bmatrix} r & 0 & 0 & -\frac{r^2+1}{t} & 0 & 0 \\ 0 & r & 0 & 0 & -\frac{r^2+1}{t} & 0 \\ 0 & 0 & r & 0 & 0 & -\frac{r^2+1}{t} \\ t & 0 & 0 & -r & 0 & 0 \\ 0 & t & 0 & 0 & -r & 0 \\ 0 & 0 & t & 0 & 0 & -r \end{bmatrix} \quad (7.2)$$

```
> J := convert(J0, DGtensor, [[ "con_bas", "cov_bas"], [ ]]);
J := r e1 f1 - \frac{r^2+1}{t} e1 f4 + r e2 f2 - \frac{r^2+1}{t} e2 f5 + r e3 f3 - \frac{r^2+1}{t} e3 f6 + t e4 f1
      - r e4 f4 + t e5 f2 - r e5 f5 + t e6 f3 - r e6 f6 \quad (7.3)
```

```
> w := convert(W, DGtensor);
      w := f1 f4 + f2 f5 + f3 f6 - f4 f1 - f5 f2 - f6 f3 \quad (7.4)
```

```
> g := ContractIndices(J, w, [[1, 2]]);
g := t f1 f1 - r f1 f4 + t f2 f2 - r f2 f5 + t f3 f3 - r f3 f6 - r f4 f1 + \frac{r^2+1}{t} f4 f4 - r f5 f2
      + \frac{r^2+1}{t} f5 f5 - r f6 f3 + \frac{r^2+1}{t} f6 f6 \quad (7.5)
```

```
> Nabla := Christoffel(g) :
> Nw := RearrangeIndices(CovariantDerivative(w, Nabla), [2, 3, 1]) :
> NJ := TensorBrackets(J, J, "Frolicher-Nijenhuis") :
> deltaW := DGzero("form", 1);
      deltaW := 0 f1 \quad (7.6)
```

```
> Lee := convert\left( evalDG\left( -\frac{1}{2} \cdot ContractIndices(J, deltaW, [[1, 1]]) \right), DGform \right);
      Lee := 0 f1 \quad (7.7)
```

```
> part2 := SymmetrizeIndices(evalDG(g &t deltaW), [2, 3], "SkewSymmetric") :
> part3 := SymmetrizeIndices(RearrangeIndices(ContractIndices(J,
      ContractIndices(evalDG(g &t deltaW), J, [[3, 1]]), [[1, 2]]), [2, 1, 3]), [2, 3],
      "SkewSymmetric") :
```

```
> mu := evalDG\left( Nw + \frac{1}{2} \cdot ( part2 - part3 ) \right) :
```

▼ 0

```
> cond0 := DGinfo(Nw, "CoefficientSet") :
> sol0 := solve( {op(cond0), t \neq 0} );
      sol0 := \quad (7.1.1)
> Neg0 := add( cond0[i]^2, i = 1 .. nops(cond0) ) :
```

## W1

```
[> SNw := SymmetrizeIndices(Nw, [1, 2, 3], "SkewSymmetric") :  
[> condw1 := DGinfo(evalDG(Nw - SNw), "CoefficientSet") :  
[> solve( {op(condw1), t ≠ 0, Neg0 ≠ 0} );  
[> Negw1 := add( condw1[i]2, i = 1 .. nops(condw1) ) :
```

## W3

```
[> condw3 := {op(DGinfo(deltaW, "CoefficientSet")), op(DGinfo(NJ,  
"CoefficientSet"))} :  
[> solve( {op(condw3), t ≠ 0, Neg0 ≠ 0} )  
[> Negw3 := add( condw3[i]2, i = 1 .. nops(condw3) ) :
```

## W4

```
[> condw4 := DGinfo(mu, "CoefficientSet") :  
[> solve( {op(condw4), t ≠ 0, Neg0 ≠ 0} );  
[> Negw4 := add( condw4[i]2, i = 1 .. nops(condw4) ) :
```

## W1+W2

```
[> condw12 := DGinfo(DGsimply(simplify(evalDG(Nw  
+ RearrangeIndices(ContractIndices(J, ContractIndices(J, Nw, [[1, 1]]), [[1,  
3]]), [3, 1, 2]))), "CoefficientSet") :  
[> use RealDomain in solve( {op(condw12), t ≠ 0, Neg0 ≠ 0, Negw1 ≠ 0, Negw2 ≠ 0} )  
end use  
[> Negw12 := add( condw12[i]2, i = 1 .. nops(condw12) ) :
```

## W1+W3

```
[> condw13 := {op(DGinfo(deltaW, "CoefficientSet")),  
op(DGinfo(SymmetrizeIndices(evalDG(Nw - ContractIndices(J,  
RearrangeIndices(ContractIndices(J, Nw, [[1, 3]]), [3, 1, 2]), [[1, 1]]), [1, 3],  
"Symmetric"), "CoefficientSet"))};  
[> condw13 := {0} (7.6.1)  
[> use RealDomain in s := solve( {op(condw13), t ≠ 0, Neg0 ≠ 0, Negw1 ≠ 0, Negw3  
≠ 0} ) end use;  
[> s := (7.6.2)  
[> Negw13 := add( condw13[i]2, i = 1 .. nops(condw13) ) :
```

## W1+W4

```
[> condw14 := DGinfo(SymmetrizeIndices(mu, [1, 2], "Symmetric"), "CoefficientSet") :  
[> solve( {op(condw14), t ≠ 0, Neg0 ≠ 0, Negw1 ≠ 0, Negw4 ≠ 0} );  
[> Negw14 := add( condw14[i]2, i = 1 .. nops(condw14) ) :
```

## W2+W3

```
[> part1 := evalDG(Nw - ContractIndices(J, RearrangeIndices(ContractIndices(J, Nw, [[1,
  2]]), [2, 1, 3]), [[1, 1]])) :
[> condw23 := {op(DGinfo(deltaW, "CoefficientSet")), op(DGinfo(evalDG(part1
  + RearrangeIndices(part1, [3, 1, 2]) + RearrangeIndices(part1, [2, 3, 1])),
  "CoefficientSet"))} :
[> solve({op(condw23), t ≠ 0, Neg0 ≠ 0, Negw2 ≠ 0, Negw3 ≠ 0});
[> Negw23 := add(condw23[i]2, i = 1 .. nops(condw23)) :
```

## W2+W4

```
[> condw24 := DGinfo(evalDG(ExteriorDerivative(W) - W&w Lee), "CoefficientSet") :
[> solve({op(condw24), t ≠ 0, Neg0 ≠ 0, Negw2 ≠ 0, Negw4 ≠ 0});
[> Negw24 := add(condw24[i]2, i = 1 .. nops(condw24)) :
```

## W3+W4

```
[> condw34 := DGinfo(NJ, "CoefficientSet") :
[> solve({op(condw34), t ≠ 0, Neg0 ≠ 0, Negw3 ≠ 0, Negw4 ≠ 0})
[> Negw34 := add(condw34[i]2, i = 1 .. nops(condw34)) :
```

## W1+W2+W3

```
[> condw123 := DGinfo(deltaW, "CoefficientSet");
[> condw123 := {0} (7.11.1)
[> solve({op(condw123), t ≠ 0, Neg0 ≠ 0, Negw1 ≠ 0, Negw3 ≠ 0, Negw12 ≠ 0, Negw13
  ≠ 0, Negw23 ≠ 0})
```

## W1+W2+W4

```
[> condw124 := DGinfo(evalDG(mu + ContractIndices(J,
  RearrangeIndices(ContractIndices(J, mu, [[1, 2]]), [2, 1, 3]), [[1, 1]])),
  "CoefficientSet") :
[> solve({op(condw124), t ≠ 0, Neg0 ≠ 0, Negw1 ≠ 0, Negw4 ≠ 0, Negw12 ≠ 0, Negw14
  ≠ 0, Negw24 ≠ 0});
```

## W1+W3+W4

```
[> part1 := SymmetrizeIndices(Nw, [1, 2], "Symmetric") :
[> condw134 := DGinfo(evalDG(part1 - ContractIndices(J,
  RearrangeIndices(ContractIndices(J, part1, [[1, 2]]), [2, 1, 3]), [[1, 1]])),
  "CoefficientSet") :
[> use RealDomain in solve({op(condw134), t ≠ 0, Neg0 ≠ 0, Negw1 ≠ 0, Negw3 ≠ 0,
  Negw4 ≠ 0, Negw13 ≠ 0, Negw14 ≠ 0, Negw34 ≠ 0}) end use
```

## W2+W3+W4

```
[> part1 := evalDG(Nw - ContractIndices(J, RearrangeIndices(ContractIndices(J, Nw,
  [[1, 2]]), [2, 1, 3]), [[1, 1]])) :
```

```

> condw234 := DGinfo(evalDG(part1 + RearrangeIndices(part1, [3, 1, 2])
+ RearrangeIndices(part1, [2, 3, 1])), "CoefficientSet") :
> use RealDomain in solve( {op(condw234), t ≠ 0, Neg0 ≠ 0, Negw3 ≠ 0, Negw4 ≠ 0,
Negw23 ≠ 0, Negw24 ≠ 0, Negw34 ≠ 0} ) end use

```

## A2.4

```

> restart : with(DifferentialGeometry) : with(LieAlgebras) : with(Tensor) : with(Tools) :
with(LinearAlgebra) :
> StructureEquations := [[i1, j1] = k2, [i1, k1] = -j2, [j1, k1] = i2], [i1, j1, k1, i2, j2, k2] :
> L := LieAlgebraData(StructureEquations, A24) :
> DGsetup(L, [e], [f]) :
> W := evalDG(f1 &w f4 + f2 &w f5 + f3 &w f6)
W := f1 ∧ f4 + f2 ∧ f5 + f3 ∧ f6 (8.1)

```

```

> J0 := Matrix( [[ [r, 0, 0, - (1 + r^2)/t, 0, 0], [0, r, 0, 0, - (1 + r^2)/t, 0], [0, 0, r, 0, 0, - (1 + r^2)/t],
- (1 + r^2)/t ], [t, 0, 0, -r, 0, 0], [0, t, 0, 0, -r, 0], [0, 0, t, 0, 0, -r] ] )
J0 :=
⎡  r  0  0  - (r^2 + 1)/t  0  0 ⎤
⎢  0  r  0  0  - (r^2 + 1)/t  0 ⎥
⎢  0  0  r  0  0  - (r^2 + 1)/t ⎥
⎢  t  0  0  -r  0  0 ⎥
⎢  0  t  0  0  -r  0 ⎥
⎢  0  0  t  0  0  -r ⎥
(8.2)

```

```

> J := convert(J0, DGtensor, [[ "con_bas", "cov_bas"], [ ]]);
J := r e1 f1 - (r^2 + 1)/t e1 f4 + r e2 f2 - (r^2 + 1)/t e2 f5 + r e3 f3 - (r^2 + 1)/t e3 f6 + t e4 f1
- r e4 f4 + t e5 f2 - r e5 f5 + t e6 f3 - r e6 f6 (8.3)

```

```

> w := convert(W, DGtensor);
w := f1 f4 + f2 f5 + f3 f6 - f4 f1 - f5 f2 - f6 f3 (8.4)

```

```

> g := ContractIndices(J, w, [[1, 2]]);
g := t f1 f1 - r f1 f4 + t f2 f2 - r f2 f5 + t f3 f3 - r f3 f6 - r f4 f1 + (r^2 + 1)/t f4 f4 - r f5 f2
+ (r^2 + 1)/t f5 f5 - r f6 f3 + (r^2 + 1)/t f6 f6 (8.5)

```

```

> Nabla := Christoffel(g) :
> Nw := RearrangeIndices(CovariantDerivative(w, Nabla), [2, 3, 1]) :
> NJ := TensorBrackets(J, J, "Frolicher-Nijenhuis") :
> deltaW := DGzero("form", 1);

```



*deltaW := 0 fl* (8.6)

> *Lee := convert*(*evalDG*( $-\frac{1}{2} \cdot \text{ContractIndices}(J, \text{deltaW}, [[1, 1]])$ ), *DGform*);

*Lee := 0 fl* (8.7)

> *part2 := SymmetrizeIndices*(*evalDG*(*g &t deltaW*), [2, 3], "SkewSymmetric") :

> *part3 := SymmetrizeIndices*(*RearrangeIndices*(*ContractIndices*(*J*,  
*ContractIndices*(*evalDG*(*g &t deltaW*), *J*, [[3, 1]]), [[1, 2]]), [2, 1, 3]), [2, 3],  
"SkewSymmetric") :

> *mu := evalDG*(*Nw* +  $\frac{1}{2} \cdot (\text{part2} - \text{part3})$ ) :

▼ 0

> *cond0 := DGinfo*(*Nw*, "CoefficientSet") :

> *sol0 := solve*(*op*(*cond0*), *t* ≠ 0);

*sol0 :=*

(8.1.1)

> *Neg0 := add*(*cond0*[*i*]<sup>2</sup>, *i* = 1..*nops*(*cond0*)) :

▼ W1

> *SNw := SymmetrizeIndices*(*Nw*, [1, 2, 3], "SkewSymmetric") :

> *condw1 := DGinfo*(*evalDG*(*Nw* - *SNw*), "CoefficientSet") :

> *solve*(*op*(*condw1*), *t* ≠ 0, *Neg0* ≠ 0);

$\{r = \text{RootOf}(\_Z^2 + 1), t = t\}$

(8.2.1)

> *Negw1 := add*(*condw1*[*i*]<sup>2</sup>, *i* = 1..*nops*(*condw1*)) :

▼ W3

> *condw3 := {op*(*DGinfo*(*deltaW*, "CoefficientSet")), *op*(*DGinfo*(*NJ*,  
"CoefficientSet"))} :

> *solve*(*op*(*condw3*), *t* ≠ 0, *Neg0* ≠ 0)

> *Negw3 := add*(*condw3*[*i*]<sup>2</sup>, *i* = 1..*nops*(*condw3*)) :

▼ W4

> *condw4 := DGinfo*(*mu*, "CoefficientSet") :

> *solve*(*op*(*condw4*), *t* ≠ 0, *Neg0* ≠ 0);

> *Negw4 := add*(*condw4*[*i*]<sup>2</sup>, *i* = 1..*nops*(*condw4*)) :

▼ W1+W2

> *condw12 := DGinfo*(*DGimplify*(*simplify*(*evalDG*(*Nw*  
+ *RearrangeIndices*(*ContractIndices*(*J*, *ContractIndices*(*J*, *Nw*, [[1, 1]]), [[1,  
3]]), [3, 1, 2])))), "CoefficientSet") :

> **use** *RealDomain* **in** *solve*(*op*(*condw12*), *t* ≠ 0, *Neg0* ≠ 0, *Negw1* ≠ 0, *Negw2* ≠ 0)  
**end use**

```
[> Negw12 := add(condw12[i]2, i = 1 ..nops(condw12)) :
```

### ▼ W1+W3

```
[> condw13 := {op(DGinfo(deltaW, "CoefficientSet")),
  op(DGinfo(SymmetrizeIndices(evalDG(Nw-ContractIndices(J,
    RearrangeIndices(ContractIndices(J, Nw, [[1, 3]]), [3, 1, 2]), [[1, 1]])), [1, 3],
    "Symmetric"), "CoefficientSet"))};
                                condw13 := {0} (8.6.1)
[> use RealDomain in solve({op(condw13), t ≠ 0, Neg0 ≠ 0, Negw1 ≠ 0, Negw3 ≠ 0});
  end use;
[> Negw13 := add(condw13[i]2, i = 1 ..nops(condw13)) :
```

### ▼ W1+W4

```
[> condw14 := DGinfo(SymmetrizeIndices(mu, [1, 2], "Symmetric"), "CoefficientSet") :
[> solve({op(condw14), t ≠ 0, Neg0 ≠ 0, Negw1 ≠ 0, Negw4 ≠ 0});
[> Negw14 := add(condw14[i]2, i = 1 ..nops(condw14)) :
```

### ▼ W2+W3

```
[> part1 := evalDG(Nw-ContractIndices(J, RearrangeIndices(ContractIndices(J, Nw, [[1,
  2]]), [2, 1, 3]), [[1, 1]])) :
[> condw23 := {op(DGinfo(deltaW, "CoefficientSet")), op(DGinfo(evalDG(part1
  + RearrangeIndices(part1, [3, 1, 2]) + RearrangeIndices(part1, [2, 3, 1])),
  "CoefficientSet"))} :
[> solve({op(condw23), t ≠ 0, Neg0 ≠ 0, Negw2 ≠ 0, Negw3 ≠ 0});
[> Negw23 := add(condw23[i]2, i = 1 ..nops(condw23)) :
```

### ▼ W2+W4

```
[> condw24 := DGinfo(evalDG(ExteriorDerivative(W) - W&w Lee), "CoefficientSet") :
[> solve({op(condw24), t ≠ 0, Neg0 ≠ 0, Negw2 ≠ 0, Negw4 ≠ 0});
[> Negw24 := add(condw24[i]2, i = 1 ..nops(condw24)) :
```

### ▼ W3+W4

```
[> condw34 := DGinfo(NJ, "CoefficientSet") :
[> solve({op(condw34), t ≠ 0, Neg0 ≠ 0, Negw3 ≠ 0, Negw4 ≠ 0});
[> Negw34 := add(condw34[i]2, i = 1 ..nops(condw34)) :
```

### ▼ W1+W2+W3

```
[> condw123 := DGinfo(deltaW, "CoefficientSet") :
[> solve({op(condw123), t ≠ 0, Neg0 ≠ 0, Negw1 ≠ 0, Negw3 ≠ 0, Negw12 ≠ 0, Negw13
  ≠ 0, Negw23 ≠ 0})
```

### ▼ W1+W2+W4

```

> condw124 := DGinfo(evalDG(mu + ContractIndices(J,
  RearrangeIndices(ContractIndices(J, mu, [[1, 2]]), [2, 1, 3]), [[1, 1]])),
  "CoefficientSet") :
> solve({op(condw124), t ≠ 0, Neg0 ≠ 0, Negw1 ≠ 0, Negw4 ≠ 0, Negw12 ≠ 0, Negw14
  ≠ 0, Negw24 ≠ 0});

```

### ▼ W1+W3+W4

```

> part1 := SymmetrizeIndices(Nw, [1, 2], "Symmetric") :
> condw134 := DGinfo(evalDG(part1 - ContractIndices(J,
  RearrangeIndices(ContractIndices(J, part1, [[1, 2]]), [2, 1, 3]), [[1, 1]])),
  "CoefficientSet") :
> use RealDomain in solve({op(condw134), t ≠ 0, Neg0 ≠ 0, Negw1 ≠ 0, Negw3 ≠ 0,
  Negw4 ≠ 0, Negw13 ≠ 0, Negw14 ≠ 0, Negw34 ≠ 0}) end use

```

### ▼ W2+W3+W4

```

> part1 := evalDG(Nw - ContractIndices(J, RearrangeIndices(ContractIndices(J, Nw,
  [[1, 2]]), [2, 1, 3]), [[1, 1]])) :
> condw234 := DGinfo(evalDG(part1 + RearrangeIndices(part1, [3, 1, 2])
  + RearrangeIndices(part1, [2, 3, 1])), "CoefficientSet") :
> use RealDomain in solve({op(condw234), t ≠ 0, Neg0 ≠ 0, Negw3 ≠ 0, Negw4 ≠ 0,
  Negw23 ≠ 0, Negw24 ≠ 0, Negw34 ≠ 0}) end use

```
