# Supplementary material for: Homogeneous almost complex structures in dimension 6 with semi-simple isotropy
Source: arXiv:1401.8187 ancillary file (2014-02-12)
Supplement: Supplementary file 3 [file SKT.pdf]

We test our homogeneous (pseudo) Hermitian structures for the Strong Kähler with Torsion (SKT) property:  $\text{NJ}=0$  &  $(d \circ J)^2 \omega = 0$ .

We also test for a generalization of the condition:  $(d \circ J)^k \omega = 0$

$k=1$  is Kähler,  $k=2$  is SKT and others are apparently new.

## A1.1

```
> restart : with(DifferentialGeometry) : with(LieAlgebras) : with(Tensor) : with(Tools) :
with(LinearAlgebra) :
```

```
> StructureEquations := [ [ee, ii] = α * e, [jj, kk] = -α * e, [ee, ie] =  $\frac{\epsilon}{2}$  * ee + r * ii, [ii, ie] =  $\frac{\epsilon}{2}$ 
* ii - r * ee, [jj, ie] =  $\frac{\epsilon}{2}$  * jj - r * kk, [kk, ie] =  $\frac{\epsilon}{2}$  * kk + r * jj, [e, ie] = ε * e ], [ee, ii, jj,
kk, e, ie] :
```

```
L := LieAlgebraData(StructureEquations, VC);
```

$$L := \left[ [e1, e2] = \alpha e5, [e1, e6] = r e2 + \frac{1}{2} \epsilon e1, [e2, e6] = \frac{1}{2} \epsilon e2 - r e1, [e3, e4] = -\alpha e5, \right. \quad (1.1)$$

$$\left. [e3, e6] = -r e4 + \frac{1}{2} \epsilon e3, [e4, e6] = \frac{1}{2} \epsilon e4 + r e3, [e5, e6] = \epsilon e5 \right]$$

```
> DGsetup(L, [e], [f]) :
```

```
> Query("Jacobi");
```

true

(1.2)

```
> g := evalDG(t * (f1 &t f1 + f2 &t f2 + f3 &t f3 + f4 &t f4) + (f5 &t f5 + f6 &t f6));
```

$$g := t f1 f1 + t f2 f2 + t f3 f3 + t f4 f4 + f5 f5 + f6 f6$$

(1.3)

```
> J0 := Matrix([ [0, -cos(a) sin(b), -sin(a) sin(b), -cos(b), 0, 0], [cos(a) sin(b), 0,
cos(b), -sin(a) sin(b), 0, 0], [sin(a) sin(b), -cos(b), 0,
cos(a) sin(b), 0, 0], [cos(b), sin(a) sin(b), -cos(a) sin(b), 0, 0, 0], [0, 0, 0, 0, 0, -1],
[0, 0, 0, 0, 1, 0]]);
```

$$J0 := \begin{bmatrix} 0 & -\cos(a) \sin(b) & -\sin(a) \sin(b) & -\cos(b) & 0 & 0 \\ \cos(a) \sin(b) & 0 & \cos(b) & -\sin(a) \sin(b) & 0 & 0 \\ \sin(a) \sin(b) & -\cos(b) & 0 & \cos(a) \sin(b) & 0 & 0 \\ \cos(b) & \sin(a) \sin(b) & -\cos(a) \sin(b) & 0 & 0 & 0 \\ 0 & 0 & 0 & 0 & 0 & -1 \\ 0 & 0 & 0 & 0 & 1 & 0 \end{bmatrix} \quad (1.4)$$

```
> J := convert(J0, DGtensor, [[ "con_bas", "cov_bas"], [ ]]);
```

$$J := -\cos(a) \sin(b) e1 f2 - \sin(a) \sin(b) e1 f3 - \cos(b) e1 f4 + \cos(a) \sin(b) e2 f1 \quad (1.5)$$

$$+ \cos(b) e2 f3 - \sin(a) \sin(b) e2 f4 + \sin(a) \sin(b) e3 f1 - \cos(b) e3 f2$$

$$+ \cos(a) \sin(b) e3 f4 + \cos(b) e4 f1 + \sin(a) \sin(b) e4 f2 - \cos(a) \sin(b) e4 f3$$

$$- e5 f6 + e6 f5$$

```
> w := convert(ContractIndices(J, g, [[1, 1]]), DGform);
```

$$w := \cos(a) \sin(b) t f1 \wedge f2 + \sin(a) \sin(b) t f1 \wedge f3 + \cos(b) t f1 \wedge f4 - \cos(b) t f2 \wedge f3 \quad (1.6)$$

$$+ \sin(a) \sin(b) t f2 \wedge f4 - \cos(a) \sin(b) t f3 \wedge f4 + f5 \wedge f6$$

>  $Jt := Transformation(VC, VC, J0) :$

>  $w1 := Pullback(Jt, ExteriorDerivative(w))$

$$\begin{aligned} w1 := & (2 \cos(b)^2 \cos(a)^2 \alpha + \epsilon \cos(a) \sin(b) t - 2 \cos(a)^2 \alpha + \alpha) f1 \wedge f2 \wedge f5 \\ & + (2 \cos(b)^2 \sin(a) \cos(a) \alpha + \epsilon \sin(a) \sin(b) t + 2 r \cos(b) t \\ & - 2 \sin(a) \cos(a) \alpha) f1 \wedge f3 \wedge f5 - (2 \cos(b) \cos(a) \sin(b) \alpha + 2 r \sin(a) \sin(b) t \\ & - \epsilon \cos(b) t) f1 \wedge f4 \wedge f5 + (2 \cos(b) \cos(a) \sin(b) \alpha + 2 r \sin(a) \sin(b) t \\ & - \epsilon \cos(b) t) f2 \wedge f3 \wedge f5 + (2 \cos(b)^2 \sin(a) \cos(a) \alpha + \epsilon \sin(a) \sin(b) t \\ & + 2 r \cos(b) t - 2 \sin(a) \cos(a) \alpha) f2 \wedge f4 \wedge f5 - (2 \cos(b)^2 \cos(a)^2 \alpha \\ & + \epsilon \cos(a) \sin(b) t - 2 \cos(a)^2 \alpha + \alpha) f3 \wedge f4 \wedge f5 \end{aligned} \quad (1.7)$$

>  $w2 := Pullback(Jt, ExteriorDerivative(w1))$

$$\begin{aligned} w2 := & 2 \alpha (2 \cos(b)^2 \cos(a)^2 \alpha + \epsilon \cos(a) \sin(b) t - 2 \cos(a)^2 \alpha + \alpha) f1 \wedge f2 \wedge f3 \wedge f4 \\ & - (8 \cos(b)^2 \cos(a)^3 \sin(b) r^2 t - 8 \cos(a)^3 \sin(b) r^2 t + 8 \cos(a) \sin(b) r^2 t \\ & + 2 \cos(a) \sin(b) t \epsilon^2 - 2 \alpha \epsilon) f1 \wedge f2 \wedge f5 \wedge f6 - (4 \sin(b) \sin(a) r^2 t \\ & - 2 \cos(b) r t \epsilon + 2 \sin(b) \sin(a) t \epsilon^2 - 4 \cos(b) \cos(a) \sin(b) r \alpha \\ & - 8 \sin(b) \sin(a) r^2 \cos(a)^2 t + 8 \cos(b)^2 \cos(a)^2 \sin(b) \sin(a) r^2 t) \\ & f1 \wedge f3 \wedge f5 \wedge f6 - (-4 \cos(b)^2 \cos(a) \sin(a) r \alpha + 8 \cos(b)^3 \cos(a)^2 r^2 t \\ & - 8 \cos(b) r^2 t \cos(a)^2 + 4 \cos(b) r^2 t + 2 \cos(b) t \epsilon^2 + 4 \cos(a) \sin(a) r \alpha \\ & + 2 \sin(b) \sin(a) r t \epsilon) f1 \wedge f4 \wedge f5 \wedge f6 + (-4 \cos(b)^2 \cos(a) \sin(a) r \alpha \\ & + 8 \cos(b)^3 \cos(a)^2 r^2 t - 8 \cos(b) r^2 t \cos(a)^2 + 4 \cos(b) r^2 t + 2 \cos(b) t \epsilon^2 \\ & + 4 \cos(a) \sin(a) r \alpha + 2 \sin(b) \sin(a) r t \epsilon) f2 \wedge f3 \wedge f5 \wedge f6 \\ & - (4 \sin(b) \sin(a) r^2 t - 2 \cos(b) r t \epsilon + 2 \sin(b) \sin(a) t \epsilon^2 \\ & - 4 \cos(b) \cos(a) \sin(b) r \alpha - 8 \sin(b) \sin(a) r^2 \cos(a)^2 t \\ & + 8 \cos(b)^2 \cos(a)^2 \sin(b) \sin(a) r^2 t) f2 \wedge f4 \wedge f5 \wedge f6 \\ & + (8 \cos(b)^2 \cos(a)^3 \sin(b) r^2 t - 8 \cos(a)^3 \sin(b) r^2 t + 8 \cos(a) \sin(b) r^2 t \\ & + 2 \cos(a) \sin(b) t \epsilon^2 - 2 \alpha \epsilon) f3 \wedge f4 \wedge f5 \wedge f6 \end{aligned} \quad (1.8)$$

>  $w3 := Pullback(Jt, ExteriorDerivative(w2))$

$$\begin{aligned} w3 := & -8 \alpha (2 \cos(b)^2 \cos(a)^3 \sin(b) r^2 t - 2 \cos(a)^3 \sin(b) r^2 t - \cos(a)^2 \cos(b)^2 \alpha \epsilon \\ & + 2 \cos(a) \sin(b) r^2 t + \cos(a)^2 \alpha \epsilon - \alpha \epsilon) f1 \wedge f2 \wedge f3 \wedge f4 \wedge f5 \end{aligned} \quad (1.9)$$

>  $w4 := Pullback(Jt, ExteriorDerivative(w3))$

$$\begin{aligned} w4 := & 24 \epsilon \alpha (2 \cos(b)^2 \cos(a)^3 \sin(b) r^2 t - 2 \cos(a)^3 \sin(b) r^2 t - \cos(a)^2 \cos(b)^2 \alpha \epsilon \\ & + 2 \cos(a) \sin(b) r^2 t + \cos(a)^2 \alpha \epsilon - \alpha \epsilon) f1 \wedge f2 \wedge f3 \wedge f4 \wedge f5 \wedge f6 \end{aligned} \quad (1.10)$$

>  $NJ := TensorBrackets(J, J, "Frolicher-Nijenhuis") :$

> **use** *RealDomain* **in**  $Slv := solve(\{op(DGinfo(w2, "CoefficientSet")), op(DGinfo(NJ, "CoefficientSet"))\}, t \neq 0, \alpha \neq 0)$  **end use**

$$Slv := \left\{ a=0, b=\frac{1}{2}\pi, r=r, t=t, \alpha=\varepsilon t, \varepsilon=\varepsilon \right\}, \left\{ a=\pi, b=-\frac{1}{2}\pi, r=r, t=t, \alpha=\varepsilon t, \varepsilon=\varepsilon \right\}, \quad (1.11)$$

$$\left\{ a=0, b=-\frac{1}{2}\pi, r=r, t=t, \alpha=-\varepsilon t, \varepsilon=\varepsilon \right\}, \left\{ a=\pi, b=\frac{1}{2}\pi, r=r, t=t, \alpha=-\varepsilon t, \varepsilon=\varepsilon \right\}$$

If  $\varepsilon=0$ , then the structure is flat, so we let  $\varepsilon=1$

> use RealDomain in  $Slv := solve(\{op(DGinfo(w2, "CoefficientSet")), op(DGinfo(NJ, "CoefficientSet")), t \neq 0, \alpha \neq 0, \varepsilon = 1\})$  end use

$$Slv := \left\{ a=0, b=\frac{1}{2}\pi, r=r, t=t, \alpha=t, \varepsilon=1 \right\}, \left\{ a=0, b=-\frac{1}{2}\pi, r=r, t=t, \alpha=-t, \varepsilon=1 \right\}, \quad (1.12)$$

$$\left\{ a=\pi, b=\frac{1}{2}\pi, r=r, t=t, \alpha=-t, \varepsilon=1 \right\}, \left\{ a=\pi, b=-\frac{1}{2}\pi, r=r, t=t, \alpha=t, \varepsilon=1 \right\}$$

The first and the last cases correspond to  $q=+i$ , the other two to  $q=-i$  (this can be changed to  $+$  by the price of changing the parameters)

> evalDG(subs(Slv[1], EinsteinTensor(g) +  $\Lambda \cdot InverseMetric(g)$ )); evalDG(subs(Slv[2], EinsteinTensor(g) +  $\Lambda \cdot InverseMetric(g)$ ));

evalDG(subs(Slv[3], EinsteinTensor(g) +  $\Lambda \cdot InverseMetric(g)$ )); evalDG(subs(Slv[4], EinsteinTensor(g) +  $\Lambda \cdot InverseMetric(g)$ ))

$$\frac{\Lambda+4}{t} e1 e1 + \frac{\Lambda+4}{t} e2 e2 + \frac{\Lambda+4}{t} e3 e3 + \frac{\Lambda+4}{t} e4 e4 + (\Lambda+4) e5 e5 + (\Lambda+4) e6 e6$$

$$\frac{\Lambda+4}{t} e1 e1 + \frac{\Lambda+4}{t} e2 e2 + \frac{\Lambda+4}{t} e3 e3 + \frac{\Lambda+4}{t} e4 e4 + (\Lambda+4) e5 e5 + (\Lambda+4) e6 e6$$

$$\frac{\Lambda+4}{t} e1 e1 + \frac{\Lambda+4}{t} e2 e2 + \frac{\Lambda+4}{t} e3 e3 + \frac{\Lambda+4}{t} e4 e4 + (\Lambda+4) e5 e5 + (\Lambda+4) e6 e6$$

$$\frac{\Lambda+4}{t} e1 e1 + \frac{\Lambda+4}{t} e2 e2 + \frac{\Lambda+4}{t} e3 e3 + \frac{\Lambda+4}{t} e4 e4 + (\Lambda+4) e5 e5 + (\Lambda+4) e6 e6 \quad (1.13)$$

This was a check of the Einstein condition

> simplify(subs(Slv[1], w1)); DGsimplify(simplify(subs(Slv[1], NJ))); simplify(subs(Slv[1], J0))

$$0 f1 \wedge f2 \wedge f5 + 0 f1 \wedge f3 \wedge f5 + 0 f1 \wedge f4 \wedge f5 + 0 f2 \wedge f3 \wedge f5 + 0 f2 \wedge f4 \wedge f5$$

$$+ 0 f3 \wedge f4 \wedge f5$$

$$0 e1 f1 f1$$

(1.14)

$$\begin{bmatrix} 0 & -1 & 0 & 0 & 0 & 0 \\ 1 & 0 & 0 & 0 & 0 & 0 \\ 0 & 0 & 0 & 1 & 0 & 0 \\ 0 & 0 & -1 & 0 & 0 & 0 \\ 0 & 0 & 0 & 0 & 0 & -1 \\ 0 & 0 & 0 & 0 & 1 & 0 \end{bmatrix} \quad (1.14)$$

> *simplify(subs(Slv[2], w1)); DGsimplify(simplify(subs(Slv[2], NJ)); simplify(subs(Slv[2], J0))*

$$0 f1 \wedge f2 \wedge f5 + 0 f1 \wedge f3 \wedge f5 + 0 f1 \wedge f4 \wedge f5 + 0 f2 \wedge f3 \wedge f5 + 0 f2 \wedge f4 \wedge f5 + 0 f3 \wedge f4 \wedge f5$$

$$0 e1 f1 f1 \begin{bmatrix} 0 & -1 & 0 & 0 & 0 & 0 \\ 1 & 0 & 0 & 0 & 0 & 0 \\ 0 & 0 & 0 & 1 & 0 & 0 \\ 0 & 0 & -1 & 0 & 0 & 0 \\ 0 & 0 & 0 & 0 & 0 & -1 \\ 0 & 0 & 0 & 0 & 1 & 0 \end{bmatrix} \quad (1.15)$$

> *simplify(subs(Slv[3], w1)); DGsimplify(simplify(subs(Slv[3], NJ)); simplify(subs(Slv[3], J0))*

$$0 f1 \wedge f2 \wedge f5 + 0 f1 \wedge f3 \wedge f5 + 0 f1 \wedge f4 \wedge f5 + 0 f2 \wedge f3 \wedge f5 + 0 f2 \wedge f4 \wedge f5 + 0 f3 \wedge f4 \wedge f5$$

$$0 e1 f1 f1 \begin{bmatrix} 0 & 1 & 0 & 0 & 0 & 0 \\ -1 & 0 & 0 & 0 & 0 & 0 \\ 0 & 0 & 0 & -1 & 0 & 0 \\ 0 & 0 & 1 & 0 & 0 & 0 \\ 0 & 0 & 0 & 0 & 0 & -1 \\ 0 & 0 & 0 & 0 & 1 & 0 \end{bmatrix} \quad (1.16)$$

> *simplify(subs(Slv[4], w1)); DGsimplify(simplify(subs(Slv[4], NJ)); simplify(subs(Slv[4], J0))*

$$0 f1 \wedge f2 \wedge f5 + 0 f1 \wedge f3 \wedge f5 + 0 f1 \wedge f4 \wedge f5 + 0 f2 \wedge f3 \wedge f5 + 0 f2 \wedge f4 \wedge f5 + 0 f3 \wedge f4 \wedge f5$$

$$0 e1 f1 f1$$

(1.17)

$$\begin{bmatrix} 0 & 1 & 0 & 0 & 0 & 0 \\ -1 & 0 & 0 & 0 & 0 & 0 \\ 0 & 0 & 0 & -1 & 0 & 0 \\ 0 & 0 & 1 & 0 & 0 & 0 \\ 0 & 0 & 0 & 0 & 0 & -1 \\ 0 & 0 & 0 & 0 & 1 & 0 \end{bmatrix} \quad (1.17)$$

Thus these SKT are the Kahler structures

## A1.2

```
> restart : with(DifferentialGeometry) : with(LieAlgebras) : with(Tensor) : with(Tools) :
with(LinearAlgebra) :
```

Here the element  $i$  of  $V=H$  is fixed by the structure equations, so the endomorphism ring is smaller. Namely we can allow rotation  $\exp(c*i)$  around the  $i$  axis in  $\text{Im}(H)$ . This allows us to make the  $k$ -coefficient of  $q$  vanish:  $q \in \langle i, j \rangle$ . This reduces the computations. The  $p = M*i + L*j + K*k$  is general imaginary quaternion.

```
> StructureEquations := [[ee, ii] = e + M*ie, [ee, jj] = L*ie, [ee, kk] = K*ie, [ii, jj] = -K*ie,
[ii, kk] = L*ie, [jj, kk] = -e - M*ie], [ee, ii, jj, kk, e, ie] :
```

```
> LL := LieAlgebraData(StructureEquations, VC)
LL := [[e1, e2] = Me6 + e5, [e1, e3] = Le6, [e1, e4] = Ke6, [e2, e3] = -Ke6, [e2, e4]
= Le6, [e3, e4] = -Me6 - e5] (2.1)
```

```
> DGsetup(LL, [e], [f]) : Query("Jacobi")
true (2.2)
```

```
> g := evalDG((f1 &t f1 + f2 &t f2 + f3 &t f3 + f4 &t f4) + t*(f5 &t f5 + f6 &t f6));
g := f1 f1 + f2 f2 + f3 f3 + f4 f4 + t f5 f5 + t f6 f6 (2.3)
```

```
> J0 := eval(subs(b = pi/2, Matrix([ [0, -cos(a) sin(b), -sin(a) sin(b), -cos(b), 0, 0],
[cos(a) sin(b), 0,
cos(b), -sin(a) sin(b), 0, 0], [sin(a) sin(b), -cos(b), 0,
cos(a) sin(b), 0, 0], [cos(b), sin(a) sin(b), -cos(a) sin(b), 0, 0, 0], [0, 0, 0, 0, 0, -1],
[0, 0, 0, 0, 1, 0]])))
```

$$J0 := \begin{bmatrix} 0 & -\cos(a) & -\sin(a) & 0 & 0 & 0 \\ \cos(a) & 0 & 0 & -\sin(a) & 0 & 0 \\ \sin(a) & 0 & 0 & \cos(a) & 0 & 0 \\ 0 & \sin(a) & -\cos(a) & 0 & 0 & 0 \\ 0 & 0 & 0 & 0 & 0 & -1 \\ 0 & 0 & 0 & 0 & 1 & 0 \end{bmatrix} \quad (2.4)$$

```
> J := convert(J0, DGtensor, [["con_bas", "cov_bas"], [ ]]) : Jt := Transformation(VC, VC,
J0) :
```

```
> w := convert(ContractIndices(J, g, [[1, 1]]), DGform);
```

$$w := \cos(a) f1 \wedge f2 + \sin(a) f1 \wedge f3 + \sin(a) f2 \wedge f4 - \cos(a) f3 \wedge f4 + t f5 \wedge f6 \quad (2.5)$$

$$\begin{aligned} &> w1 := \text{Pullback}(Jt, \text{ExteriorDerivative}(w)) \\ w1 &:= -t (2 \cos(a)^2 - 1) f1 \wedge f2 \wedge f5 - t (2 L \sin(a) \cos(a) + 2 M \cos(a)^2 \\ &\quad - M) f1 \wedge f2 \wedge f6 - 2 t \cos(a) \sin(a) f1 \wedge f3 \wedge f5 + t (2 L \cos(a)^2 \\ &\quad - 2 M \sin(a) \cos(a) - L) f1 \wedge f3 \wedge f6 + K t f1 \wedge f4 \wedge f6 - K t f2 \wedge f3 \wedge f6 \\ &\quad - 2 t \cos(a) \sin(a) f2 \wedge f4 \wedge f5 + t (2 L \cos(a)^2 - 2 M \sin(a) \cos(a) \\ &\quad - L) f2 \wedge f4 \wedge f6 + t (2 \cos(a)^2 - 1) f3 \wedge f4 \wedge f5 + t (2 L \sin(a) \cos(a) \\ &\quad + 2 M \cos(a)^2 - M) f3 \wedge f4 \wedge f6 \end{aligned} \quad (2.6)$$

$$\begin{aligned} &> w2 := \text{Pullback}(Jt, \text{ExteriorDerivative}(w1)) \\ w2 &:= 2 t (2 L^2 \cos(a)^2 - 4 L M \sin(a) \cos(a) - 2 M^2 \cos(a)^2 + K^2 - L^2 + M^2 - 2 \cos(a)^2 \\ &\quad + 1) f1 \wedge f2 \wedge f3 \wedge f4 \end{aligned} \quad (2.7)$$

$$\begin{aligned} &> w3 := \text{Pullback}(Jt, \text{ExteriorDerivative}(w2)) \\ w3 &:= 0 f1 \wedge f2 \wedge f3 \wedge f4 \wedge f5 \end{aligned} \quad (2.8)$$

$$\begin{aligned} &> NJ := \text{TensorBrackets}(J, J, \text{"Frolicher-Nijenhuis"}) : \\ &> \text{KaehlerEq} := \text{DGinfo}(\text{ExteriorDerivative}(w), \text{"CoefficientSet"}); \\ &\quad \text{KaehlerEq} := \{t, K t, L t, M t, -t, -K t, -M t\} \end{aligned} \quad (2.9)$$

$$\begin{aligned} &> \text{SumKaehlerEq} := \text{factor}(\text{add}(\text{KaehlerEq}[i]^2, i = 1 \dots \text{nops}(\text{KaehlerEq}))); \\ &\quad \text{SumKaehlerEq} := t^2 (2 K^2 + L^2 + 2 M^2 + 2) \end{aligned} \quad (2.10)$$

$$\begin{aligned} &> \text{sols} := \text{solve}(\{ \text{op}(\text{DGinfo}(w2, \text{"CoefficientSet"})), \text{op}(\text{DGinfo}(NJ, \text{"CoefficientSet"})), t \\ &\quad \neq 0 \}) \\ \text{sols} &:= \left\{ K = -1, L = \text{RootOf}(\_Z^2 - 2), M = 0, a = -\frac{1}{2} \pi, t = t \right\}, \{ K = \sin(a), L \\ &\quad = \text{RootOf}(\_Z^2 - 3 \sin(a)^2 + 1) \sin(a), M = \text{RootOf}(\_Z^2 - 3 \sin(a)^2 + 1) \cos(a), a \\ &\quad = a, t = t \}, \{ K = 0, L = 0, M = \text{RootOf}(\_Z^2 + 1), a = \pi, t = t \} \end{aligned} \quad (2.11)$$

$$\begin{aligned} &> \text{nops}(\{\text{sols}\}); \\ &\quad 3 \end{aligned} \quad (2.12)$$

The first of these solutions is a part of the second, the third is not real. So we consider only the second one, giving the general SKT case for A1.2.

This solution is  $q = \cos(a) \cdot i + \sin(a) \cdot j$ ,  $p = \pm \sqrt{3 \sin^2(a) - 1} \cdot q + \sin(a) \cdot k$

An alternative computation (similar to A3.3 below) consists in letting  $i$  in the structure equation to be changed to an arbitrary imaginary quaternion  $u$ , and fixing  $q = i$  (by an endomorphism). We can also rotate (by an endomorphism  $\langle j, k \rangle$  plane to make  $u \in \langle i, j \rangle$  (in other words, make  $k$ -component vanish).

$$\begin{aligned} &> \text{restart} : \text{with}(\text{DifferentialGeometry}) : \text{with}(\text{LieAlgebras}) : \text{with}(\text{Tensor}) : \text{with}(\text{Tools}) : \\ &\quad \text{with}(\text{LinearAlgebra}) : \\ &> \text{StructureEquations} := [[ee, ii] = \alpha 1 \cdot e + M \cdot ie, [ee, jj] = \alpha 2 \cdot e + L \cdot ie, [ee, kk] = K \cdot ie, [ii, jj] = \\ &\quad -K \cdot ie, [ii, kk] = \alpha 2 \cdot e + L \cdot ie, [jj, kk] = -\alpha 1 \cdot e - M \cdot ie], [ee, ii, jj, kk, e, ie] : \\ &> LL := \text{LieAlgebraData}(\text{StructureEquations}, \text{VC}) : \text{DGsetup}(LL, [e], [f]) : \text{Query}(\text{"Jacobi"}) \end{aligned} \quad (2.13)$$

*true* (2.13)

```

> g := evalDG((f1 &t f1 + f2 &t f2 + f3 &t f3 + f4 &t f4) + t*(f5 &t f5 + f6 &t f6)) :
> J0 := eval(subs({a=0, b=π/2}, Matrix([ [0, -cos(a) sin(b), -sin(a) sin(b), -cos(b), 0,
0], [cos(a) sin(b), 0,
cos(b), -sin(a) sin(b), 0, 0], [sin(a) sin(b), -cos(b), 0, cos(a) sin(b), 0, 0], [cos(b),
sin(a) sin(b), -cos(a) sin(b), 0, 0, 0], [0, 0, 0, 0, 0, -1], [0, 0, 0, 0, 1, 0]])))

```

$$J0 := \begin{bmatrix} 0 & -1 & 0 & 0 & 0 & 0 \\ 1 & 0 & 0 & 0 & 0 & 0 \\ 0 & 0 & 0 & 1 & 0 & 0 \\ 0 & 0 & -1 & 0 & 0 & 0 \\ 0 & 0 & 0 & 0 & 0 & -1 \\ 0 & 0 & 0 & 0 & 1 & 0 \end{bmatrix} \quad (2.14)$$

```

> J := convert(J0, DGtensor, [{"con_bas", "cov_bas"}, [ ]]) : Jt := Transformation(VC, VC,
J0) :
> w := convert(ContractIndices(J, g, [[1, 1]]), DGform) :
> w1 := Pullback(Jt, ExteriorDerivative(w)) :
> w2 := Pullback(Jt, ExteriorDerivative(w1)) :
> w3 := Pullback(Jt, ExteriorDerivative(w2))

```

$$w3 := 0 f1 \wedge f2 \wedge f3 \wedge f4 \wedge f5 \quad (2.15)$$

```

> NJ := TensorBrackets(J, J, "Frolicher-Nijenhuis") :
> KaehlerEq := DGinfo(ExteriorDerivative(w), "CoefficientSet");

```

$$KaehlerEq := \{K t, L t, M t, \alpha t, -K t, -M t, -\alpha t, -\alpha^2 t\} \quad (2.16)$$

```

> SumKaehlerEq := factor(add(KaehlerEq[i]^2, i=1..nops(KaehlerEq)));

```

$$SumKaehlerEq := t^2 (2 K^2 + L^2 + 2 M^2 + 2 \alpha^2 + \alpha^2) \quad (2.17)$$

```

> sols := convert(solve({op(DGinfo(NJ, "CoefficientSet")), op(DGinfo(w2,
"CoefficientSet")), t ≠ 0, SumKaehlerEq ≠ 0}), radical)

```

$$sols := \{K = -\alpha^2, L = 0, M = \sqrt{-\alpha^2 + 2 \alpha^2}, t = t, \alpha = \alpha, \alpha^2 = \alpha^2\} \quad (2.18)$$

### A1.3

```

> restart : with(DifferentialGeometry) : with(LieAlgebras) : with(Tensor) : with(Tools) :
> StructureEquations := [[ee, e] = α·ee, [ii, e] = α·ii, [jj, e] = α·jj, [kk, e] = α·kk, [ee, ie] = β
·ee + r·ii, [ii, ie] = β·ii - r·ee, [jj, ie] = β·jj - r·kk, [kk, ie] = β·kk + r·jj, [e, ie] = ε·e] :
> L := LieAlgebraData(StructureEquations, [ee, ii, jj, kk, e, ie], VC) :
> DGsetup(L, [e], [f]) :
> Query({a, ε}, "Jacobi")

```

$$true, \{0, -\epsilon \alpha\}, [\{a = a, \epsilon = 0\}], [[e1, e5] = \alpha e1, [e1, e6] = e1 \beta + e2 r, [e2, e5] = \alpha e2, \quad (3.1)$$

$$[e2, e6] = -e1 r + e2 \beta, [e3, e5] = \alpha e3, [e3, e6] = e3 \beta - e4 r, [e4, e5] = \alpha e4, [e4, e6]$$

$$= e3 r + e4 \beta]$$

$$\begin{aligned} &> g := \text{evalDG}((f1 \&t f1 + f2 \&t f2 + f3 \&t f3 + f4 \&t f4) + t \cdot (f5 \&t f5 + f6 \&t f6)); \\ &\quad g := f1 f1 + f2 f2 + f3 f3 + f4 f4 + t f5 f5 + t f6 f6 \end{aligned} \quad (3.2)$$

$$\begin{aligned} &> J0 := \text{Matrix}([ [0, -\cos(a) \sin(b), -\sin(a) \sin(b), -\cos(b), 0, 0], [\cos(a) \sin(b), 0, \cos(b), -\sin(a) \sin(b), 0, 0], [\sin(a) \sin(b), -\cos(b), 0, \cos(a) \sin(b), 0, 0], [\cos(b), \sin(a) \sin(b), -\cos(a) \sin(b), 0, 0, 0], [0, 0, 0, 0, 0, -1], [0, 0, 0, 0, 1, 0]]); \\ &\quad J0 := \begin{bmatrix} 0 & -\cos(a) \sin(b) & -\sin(a) \sin(b) & -\cos(b) & 0 & 0 \\ \cos(a) \sin(b) & 0 & \cos(b) & -\sin(a) \sin(b) & 0 & 0 \\ \sin(a) \sin(b) & -\cos(b) & 0 & \cos(a) \sin(b) & 0 & 0 \\ \cos(b) & \sin(a) \sin(b) & -\cos(a) \sin(b) & 0 & 0 & 0 \\ 0 & 0 & 0 & 0 & 0 & -1 \\ 0 & 0 & 0 & 0 & 1 & 0 \end{bmatrix} \end{aligned} \quad (3.3)$$

$$\begin{aligned} &> J := \text{convert}(J0, \text{DGtensor}, [ ["con_bas", "cov_bas"], [ ]]); \\ J &:= -\cos(a) \sin(b) e1 f2 - \sin(a) \sin(b) e1 f3 - \cos(b) e1 f4 + \cos(a) \sin(b) e2 f1 \\ &\quad + \cos(b) e2 f3 - \sin(a) \sin(b) e2 f4 + \sin(a) \sin(b) e3 f1 - \cos(b) e3 f2 \\ &\quad + \cos(a) \sin(b) e3 f4 + \cos(b) e4 f1 + \sin(a) \sin(b) e4 f2 - \cos(a) \sin(b) e4 f3 \\ &\quad - e5 f6 + e6 f5 \end{aligned} \quad (3.4)$$

$$\begin{aligned} &> w := \text{convert}(\text{ContractIndices}(J, g, [[1, 1]]), \text{DGform}); \\ w &:= \cos(a) \sin(b) f1 \wedge f2 + \sin(a) \sin(b) f1 \wedge f3 + \cos(b) f1 \wedge f4 - \cos(b) f2 \wedge f3 \\ &\quad + \sin(a) \sin(b) f2 \wedge f4 - \cos(a) \sin(b) f3 \wedge f4 + t f5 \wedge f6 \end{aligned} \quad (3.5)$$

$$\begin{aligned} &> Jt := \text{Transformation}(\text{VC}, \text{VC}, J0); \\ &> w1 := \text{Pullback}(Jt, \text{ExteriorDerivative}(w)); \\ w1 &:= 2 \beta \cos(a) \sin(b) f1 \wedge f2 \wedge f5 - 2 \alpha \cos(a) \sin(b) f1 \wedge f2 \wedge f6 \end{aligned} \quad (3.6)$$

$$\begin{aligned} &\quad + (2 \beta \sin(a) \sin(b) + 2 r \cos(b)) f1 \wedge f3 \wedge f5 - 2 \alpha \sin(a) \sin(b) f1 \wedge f3 \wedge f6 \\ &\quad - (2 r \sin(a) \sin(b) - 2 \beta \cos(b)) f1 \wedge f4 \wedge f5 - 2 \alpha \cos(b) f1 \wedge f4 \wedge f6 \\ &\quad + (2 r \sin(a) \sin(b) - 2 \beta \cos(b)) f2 \wedge f3 \wedge f5 + 2 \alpha \cos(b) f2 \wedge f3 \wedge f6 \\ &\quad + (2 \beta \sin(a) \sin(b) + 2 r \cos(b)) f2 \wedge f4 \wedge f5 - 2 \alpha \sin(a) \sin(b) f2 \wedge f4 \wedge f6 \\ &\quad - 2 \beta \cos(a) \sin(b) f3 \wedge f4 \wedge f5 + 2 \alpha \cos(a) \sin(b) f3 \wedge f4 \wedge f6 \\ &> w2 := \text{factor}(\text{Pullback}(Jt, \text{ExteriorDerivative}(w1))); \\ w2 &:= -2 \cos(a) \sin(b) (4 \cos(a)^2 \cos(b)^2 r^2 - 4 \cos(a)^2 r^2 + 4 r^2 + 2 \alpha^2 + 2 \beta^2 \\ &\quad + \epsilon \beta) f1 \wedge f2 \wedge f5 \wedge f6 - (4 \sin(a) \sin(b) r^2 + 4 \alpha^2 \sin(a) \sin(b) \\ &\quad + 4 \sin(a) \sin(b) \beta^2 - 8 \sin(a) \sin(b) r^2 \cos(a)^2 + 8 \cos(a)^2 \sin(a) \sin(b) \cos(b)^2 r^2 \\ &\quad - 2 \cos(b) r \epsilon + 2 \sin(a) \sin(b) \beta \epsilon) f1 \wedge f3 \wedge f5 \wedge f6 - (8 \cos(a)^2 \cos(b)^3 r^2 \\ &\quad - 8 \cos(a)^2 \cos(b) r^2 + 2 \sin(a) \sin(b) r \epsilon + 4 \cos(b) r^2 + 4 \alpha^2 \cos(b) + 4 \cos(b) \beta^2 \\ &\quad + 2 \cos(b) \beta \epsilon) f1 \wedge f4 \wedge f5 \wedge f6 + (8 \cos(a)^2 \cos(b)^3 r^2 - 8 \cos(a)^2 \cos(b) r^2 \\ &\quad + 2 \sin(a) \sin(b) r \epsilon + 4 \cos(b) r^2 + 4 \alpha^2 \cos(b) + 4 \cos(b) \beta^2 + 2 \cos(b) \beta \epsilon) \end{aligned} \quad (3.7)$$



$$\begin{aligned}
& f2 \wedge f3 \wedge f5 \wedge f6 - \left( 4 \sin(a) \sin(b) r^2 + 4 \alpha^2 \sin(a) \sin(b) + 4 \sin(a) \sin(b) \beta^2 \right. \\
& - 8 \sin(a) \sin(b) r^2 \cos(a)^2 + 8 \cos(a)^2 \sin(a) \sin(b) \cos(b)^2 r^2 - 2 \cos(b) r \epsilon \\
& \left. + 2 \sin(a) \sin(b) \beta \epsilon \right) f2 \wedge f4 \wedge f5 \wedge f6 + 2 \cos(a) \sin(b) \left( 4 \cos(a)^2 \cos(b)^2 r^2 \right. \\
& \left. - 4 \cos(a)^2 r^2 + 4 r^2 + 2 \alpha^2 + 2 \beta^2 + \epsilon \beta \right) f3 \wedge f4 \wedge f5 \wedge f6
\end{aligned}$$

We have to explore the possibility  $q=\pm i$  (another possibility for  $N_J=0$  is  $r=0$ ,  $q\neq\pm i$ , but then we have endomorphism freedom to change  $q$  back to  $i$  because  $\text{ad}(e), \text{ad}(ie)$  act by  $\mathbb{R}$ -scalings, and so the structure eqns will not change)

$$\begin{aligned}
& > \text{factor} \left( \text{evalDG} \left( \text{subs} \left( \left\{ a=0, b=\frac{\pi}{2} \right\}, w2 \right) \right) \right) \\
& - \left( 4 \alpha^2 + 4 \beta^2 + 2 \epsilon \beta \right) f1 \wedge f2 \wedge f5 \wedge f6 + 0 f1 \wedge f3 \wedge f5 \wedge f6 + 0 f1 \wedge f4 \wedge f5 \wedge f6 \\
& + 0 f2 \wedge f3 \wedge f5 \wedge f6 + 0 f2 \wedge f4 \wedge f5 \wedge f6 + \left( 4 \alpha^2 + 4 \beta^2 \right. \\
& \left. + 2 \epsilon \beta \right) f3 \wedge f4 \wedge f5 \wedge f6
\end{aligned} \tag{3.8}$$

> SKT when  $\alpha^2 + \beta^2 + \frac{1}{2} \epsilon \beta = 0$ . To be non-Kahler we have to take  $\epsilon = 1$ ,  $\alpha = 0$ ,  $\beta = -\frac{1}{2}$ ,  $r$  any,  $q = i$  (because  $r$  is any)

Let us re-check the Kahler condition for A1.3

$$\begin{aligned}
& > \text{Sol} := \text{solve}(\text{DGinfo}(w1, \text{"CoefficientSet"})); \\
& \quad \text{Sol} := \{a=a, b=b, r=0, \alpha=0, \beta=0\}, \left\{ a=0, b=\frac{1}{2} \pi, r=r, \alpha=0, \beta=0 \right\}
\end{aligned} \tag{3.9}$$

$$> \text{simplify}(\text{subs}(\text{Sol}[1], [\text{StructureEquations}, J0]))$$

$$[[ee, e]=0, [ii, e]=0, [jj, e]=0, [kk, e]=0, [ee, ie]=0, [ii, ie]=0, [jj, ie]=0, [kk, ie] \tag{3.10}$$

$$=0, [e, ie]=\epsilon e],$$

$$\begin{bmatrix} 0 & -\cos(a) \sin(b) & -\sin(a) \sin(b) & -\cos(b) & 0 & 0 \\ \cos(a) \sin(b) & 0 & \cos(b) & -\sin(a) \sin(b) & 0 & 0 \\ \sin(a) \sin(b) & -\cos(b) & 0 & \cos(a) \sin(b) & 0 & 0 \\ \cos(b) & \sin(a) \sin(b) & -\cos(a) \sin(b) & 0 & 0 & 0 \\ 0 & 0 & 0 & 0 & 0 & -1 \\ 0 & 0 & 0 & 0 & 1 & 0 \end{bmatrix}$$

This is the case of  $H \oplus C$ , with  $H$  flat and  $C$  2D solvable (non-abelian), and  $J$  can be taken to  $i$  by an endomorphism,  $g$  is standard

> *simplify(subs(Sol[2], [StructureEquations, J0]))*

$$[[ee, e]=0, [ii, e]=0, [jj, e]=0, [kk, e]=0, [ee, ie]=ii r, [ii, ie]=-ee r, [jj, ie]=-kk r, \quad (3.11)$$

$$[kk, ie]=jj r, [e, ie]=\epsilon e], \quad \begin{bmatrix} 0 & -1 & 0 & 0 & 0 & 0 \\ 1 & 0 & 0 & 0 & 0 & 0 \\ 0 & 0 & 0 & 1 & 0 & 0 \\ 0 & 0 & -1 & 0 & 0 & 0 \\ 0 & 0 & 0 & 0 & 0 & -1 \\ 0 & 0 & 0 & 0 & 1 & 0 \end{bmatrix}$$

This case  $\alpha = \beta = 0$ ,  $J=i$  contains the previous, so this is the Kahler structure for A1.3

>

## A1.4

> *restart : with(DifferentialGeometry) : with(LieAlgebras) : with(Tensor) : with(Tools) : with(LinearAlgebra) :*

> *StructureEquations := [[LAI, LAj]=2 \* LAK, [LAI, LAK]=-2 \* LAj, [LAj, LAK]=2 \* LAi, [LAI, ee]=ii, [LAI, ii]=-ee, [LAI, jj]=kk, [LAI, kk]=-jj, [LAj, ee]=jj, [LAj, ii]=-kk, [LAj, jj]=-ee, [LAj, kk]=ii, [LAK, ee]=kk, [LAK, ii]=jj, [LAK, jj]=-ii, [LAK, kk]=-ee, [ee, ii]=-e + \epsilon \* LAi, [ee, jj]=\epsilon \* LAj, [ee, kk]=\epsilon \* LAK, [ii, jj]=\epsilon \* LAK, [ii, kk]=- \epsilon \* LAj, [jj, kk]=e + \epsilon \* LAi, [ee, e]=3 \epsilon \* ii, [ii, e]=-3 \epsilon \* ee, [jj, e]=-3 \epsilon \* kk, [kk, e]=3 \epsilon \* jj], [LAI, LAj, LAK, ee, ii, jj, kk, e, ie] :*

*L := LieAlgebraData(StructureEquations, VC);*

$$L := [[e1, e2]=2 e3, [e1, e3]=-2 e2, [e1, e4]=e5, [e1, e5]=-e4, [e1, e6]=e7, [e1, e7]=-e6, [e2, e3]=2 e1, [e2, e4]=e6, [e2, e5]=-e7, [e2, e6]=-e4, [e2, e7]=e5, [e3, e4]=e7, [e3, e5]=e6, [e3, e6]=-e5, [e3, e7]=-e4, [e4, e5]=e1 \epsilon - e8, [e4, e6]$$

$$= \varepsilon e_2, [e_4, e_7] = \varepsilon e_3, [e_4, e_8] = 3 \varepsilon e_5, [e_5, e_6] = \varepsilon e_3, [e_5, e_7] = -\varepsilon e_2, [e_5, e_8] = -3 \varepsilon e_4, [e_6, e_7] = e_1 \varepsilon + e_8, [e_6, e_8] = -3 \varepsilon e_7, [e_7, e_8] = 3 \varepsilon e_6]$$

> DGsetup(L, [e], [f]) :

> Query("Jacobi");

true

(4.2)

> g := evalDG(temp·(f1 &t f1 + f2 &t f2 + f3 &t f3) + (f4 &t f4 + f5 &t f5 + f6 &t f6 + f7 &t f7) + t·(f8 &t f8 + f9 &t f9));

$$g := temp f1 f1 + temp f2 f2 + temp f3 f3 + f4 f4 + f5 f5 + f6 f6 + f7 f7 + t f8 f8 + t f9 f9 \quad (4.3)$$

> J0 := Matrix([ [0, 0, 0, 0, 0, 0, 0, 0, 0], [0, 0, 0, 0, 0, 0, 0, 0, 0], [0, 0, 0, 0, 0, 0, 0, 0, 0], [0, 0, 0, 0, -cos(a) sin(b), -sin(a) sin(b), -cos(b), 0, 0], [0, 0, 0, cos(a) sin(b), 0, cos(b), -sin(a) sin(b), 0, 0], [0, 0, 0, sin(a) sin(b), -cos(b), 0, cos(a) sin(b), 0, 0], [0, 0, 0, cos(b), sin(a) sin(b), -cos(a) sin(b), 0, 0, 0], [0, 0, 0, 0, 0, 0, 0, 0, 0], [0, 0, 0, 0, 0, 0, 0, 0, 1], [0, 0, 0, 0, 0, 0, 0, 1, 0]]);

$$J0 := \begin{bmatrix} 0 & 0 & 0 & 0 & 0 & 0 & 0 & 0 & 0 \\ 0 & 0 & 0 & 0 & 0 & 0 & 0 & 0 & 0 \\ 0 & 0 & 0 & 0 & 0 & 0 & 0 & 0 & 0 \\ 0 & 0 & 0 & 0 & -\cos(a) \sin(b) & -\sin(a) \sin(b) & -\cos(b) & 0 & 0 \\ 0 & 0 & 0 & \cos(a) \sin(b) & 0 & \cos(b) & -\sin(a) \sin(b) & 0 & 0 \\ 0 & 0 & 0 & \sin(a) \sin(b) & -\cos(b) & 0 & \cos(a) \sin(b) & 0 & 0 \\ 0 & 0 & 0 & \cos(b) & \sin(a) \sin(b) & -\cos(a) \sin(b) & 0 & 0 & 0 \\ 0 & 0 & 0 & 0 & 0 & 0 & 0 & 0 & -1 \\ 0 & 0 & 0 & 0 & 0 & 0 & 0 & 1 & 0 \end{bmatrix} \quad (4.4)$$

> J := convert(J0, DGtensor, [[ "con\_bas", "cov\_bas"], [ ]]);

$$J := -\cos(a) \sin(b) e_4 f_5 - \sin(a) \sin(b) e_4 f_6 - \cos(b) e_4 f_7 + \cos(a) \sin(b) e_5 f_4 + \cos(b) e_5 f_6 - \sin(a) \sin(b) e_5 f_7 + \sin(a) \sin(b) e_6 f_4 - \cos(b) e_6 f_5 + \cos(a) \sin(b) e_6 f_7 + \cos(b) e_7 f_4 + \sin(a) \sin(b) e_7 f_5 - \cos(a) \sin(b) e_7 f_6 - e_8 f_9 + e_9 f_8 \quad (4.5)$$

> w := convert(ContractIndices(J, g, [[1, 1]]), DGform);

$$w := \cos(a) \sin(b) f_4 \wedge f_5 + \sin(a) \sin(b) f_4 \wedge f_6 + \cos(b) f_4 \wedge f_7 - \cos(b) f_5 \wedge f_6 + \sin(a) \sin(b) f_5 \wedge f_7 - \cos(a) \sin(b) f_6 \wedge f_7 + t f_8 \wedge f_9 \quad (4.6)$$

> Jt := Transformation(VC, VC, J0) :

> w1 := Pullback(Jt, ExteriorDerivative(w))

$$w1 := -t (2 \cos(a)^2 \cos(b)^2 - 2 \cos(a)^2 + 1) f_4 \wedge f_5 \wedge f_8 + 2 t \cos(a) \sin(b)^2 \sin(a) f_4 \wedge f_6 \wedge f_8 - 6 \varepsilon \cos(b) f_4 \wedge f_6 \wedge f_9 + 2 t \cos(a) \sin(b) \cos(b) f_4 \wedge f_7 \wedge f_8 + 6 \varepsilon \sin(a) \sin(b) f_4 \wedge f_7 \wedge f_9 - 2 t \cos(a) \sin(b) \cos(b) f_5 \wedge f_6 \wedge f_8 - 6 \varepsilon \sin(a) \sin(b) f_5 \wedge f_6 \wedge f_9 + 2 t \cos(a) \sin(b)^2 \sin(a) f_5 \wedge f_7 \wedge f_8 - 6 \varepsilon \cos(b) f_5 \wedge f_7 \wedge f_9 + t (2 \cos(a)^2 \cos(b)^2 - 2 \cos(a)^2 + 1) f_6 \wedge f_7 \wedge f_8 \quad (4.7)$$

> w2 := factor(Pullback(Jt, ExteriorDerivative(w1)))

$$w2 := 2 t (2 \cos(a)^2 \cos(b)^2 - 2 \cos(a)^2 + 1) f4 \wedge f5 \wedge f6 \wedge f7 \quad (4.8)$$

$$\begin{aligned} & - 72 \cos(a) \sin(b) \varepsilon^2 (\cos(a)^2 \cos(b)^2 - \cos(a)^2 + 1) f4 \wedge f5 \wedge f8 \wedge f9 \\ & - 36 \sin(b) \sin(a) \varepsilon^2 (2 \cos(a)^2 \cos(b)^2 - 2 \cos(a)^2 + 1) f4 \wedge f6 \wedge f8 \wedge f9 \\ & - 36 \cos(b) \varepsilon^2 (2 \cos(a)^2 \cos(b)^2 - 2 \cos(a)^2 + 1) f4 \wedge f7 \wedge f8 \wedge f9 \\ & + 36 \cos(b) \varepsilon^2 (2 \cos(a)^2 \cos(b)^2 - 2 \cos(a)^2 + 1) f5 \wedge f6 \wedge f8 \wedge f9 \\ & - 36 \sin(b) \sin(a) \varepsilon^2 (2 \cos(a)^2 \cos(b)^2 - 2 \cos(a)^2 + 1) f5 \wedge f7 \wedge f8 \wedge f9 \\ & + 72 \cos(a) \sin(b) \varepsilon^2 (\cos(a)^2 \cos(b)^2 - \cos(a)^2 + 1) f6 \wedge f7 \wedge f8 \wedge f9 \end{aligned}$$

>

$$\begin{aligned} & > w3 := \text{Pullback}(Jt, \text{ExteriorDerivative}(w2)) \\ & w3 := 144 \varepsilon^2 \cos(a) \sin(b) (1 - \cos(a)^2 + \cos(a)^2 \cos(b)^2) f4 \wedge f5 \wedge f6 \wedge f7 \wedge f8 \quad (4.9) \end{aligned}$$

$$\begin{aligned} & > w4 := \text{Pullback}(Jt, \text{ExteriorDerivative}(w3)) \\ & w4 := 0 f1 \wedge f2 \wedge f3 \wedge f4 \wedge f5 \wedge f6 \quad (4.10) \end{aligned}$$

$$\begin{aligned} & > Slv := \text{solve}(\{op(DGinfo(w2, "CoefficientSet")), t \neq 0, \varepsilon \neq 0\}) \\ & Slv := \quad (4.11) \end{aligned}$$

$$\begin{aligned} & > \text{use RealDomain in } Slv := \text{solve}(\{op(DGinfo(w3, "CoefficientSet")), t \neq 0, \varepsilon \neq 0\}) \text{ end} \\ & \text{use} \end{aligned}$$

$$Slv := \left\{ a = \frac{1}{2} \pi, b = b, \varepsilon = \varepsilon, t = t \right\}, \left\{ a = a, b = 0, \varepsilon = \varepsilon, t = t \right\} \quad (4.12)$$

One important root is lost by solve:  $\cos(a)^2=1, \cos(b)=0$ . It corresponds to the structure  $q = \pm i$

$$> \text{simplify}(\text{subs}(Slv[1], J0))$$

$$\begin{bmatrix} 0 & 0 & 0 & 0 & 0 & 0 & 0 & 0 & 0 \\ 0 & 0 & 0 & 0 & 0 & 0 & 0 & 0 & 0 \\ 0 & 0 & 0 & 0 & 0 & 0 & 0 & 0 & 0 \\ 0 & 0 & 0 & 0 & 0 & -\sin(b) & -\cos(b) & 0 & 0 \\ 0 & 0 & 0 & 0 & 0 & \cos(b) & -\sin(b) & 0 & 0 \\ 0 & 0 & 0 & \sin(b) & -\cos(b) & 0 & 0 & 0 & 0 \\ 0 & 0 & 0 & \cos(b) & \sin(b) & 0 & 0 & 0 & 0 \\ 0 & 0 & 0 & 0 & 0 & 0 & 0 & 0 & -1 \\ 0 & 0 & 0 & 0 & 0 & 0 & 0 & 1 & 0 \end{bmatrix} \quad (4.13)$$

$$> \text{simplify}(\text{subs}(Slv[2], J0))$$

$$(4.14)$$

$$\begin{bmatrix} 0 & 0 & 0 & 0 & 0 & 0 & 0 & 0 & 0 \\ 0 & 0 & 0 & 0 & 0 & 0 & 0 & 0 & 0 \\ 0 & 0 & 0 & 0 & 0 & 0 & 0 & 0 & 0 \\ 0 & 0 & 0 & 0 & 0 & 0 & -1 & 0 & 0 \\ 0 & 0 & 0 & 0 & 0 & 1 & 0 & 0 & 0 \\ 0 & 0 & 0 & 0 & -1 & 0 & 0 & 0 & 0 \\ 0 & 0 & 0 & 1 & 0 & 0 & 0 & 0 & 0 \\ 0 & 0 & 0 & 0 & 0 & 0 & 0 & 0 & -1 \\ 0 & 0 & 0 & 0 & 0 & 0 & 0 & 1 & 0 \end{bmatrix}$$

(4.14)

This is the 3-SKT property

## A2.2

```
> restart : with(DifferentialGeometry) : with(LieAlgebras) : with(Tensor) : with(Tools) :
with(LinearAlgebra) :
> StructureEquations := [[i, j] = k, [i, k] = -j, [j, k] = i, [i, j2] = k2, [i, k2] = -j2, [j, k2] = i2,
[i2, j] = k2, [i2, k] = -j2, [j2, k] = i2, [i2, j2] = -k, [i2, k2] = j, [j2, k2] = -i], [i, j, k, i2,
j2, k2] :
```

```
> L := LieAlgebraData(StructureEquations, Dsu) :
```

```
> DGsetup(L, [e], [f]) :
```

```
> w := evalDG(f1 &w f4 + f2 &w f5 + f3 &w f6) :
```

```
> J0 := Matrix([[r, 0, 0, - (1 + r^2)/t, 0, 0], [0, r, 0, 0, - (1 + r^2)/t, 0], [0, 0, r, 0, 0, 0,
- (1 + r^2)/t], [t, 0, 0, -r, 0, 0], [0, t, 0, 0, -r, 0], [0, 0, t, 0, 0, -r]]) :
```

```
> J := convert(J0, DGtensor, [[ "con_bas", "cov_bas"], [ ]]) :
```

$$J := r e1 f1 - \frac{r^2 + 1}{t} e1 f4 + r e2 f2 - \frac{r^2 + 1}{t} e2 f5 + r e3 f3 - \frac{r^2 + 1}{t} e3 f6 + t e4 f1 - r e4 f4 + t e5 f2 - r e5 f5 + t e6 f3 - r e6 f6 \quad (5.1)$$

```
> Jt := Transformation(Dsu, Dsu, J0) :
```

$$Jt := \left[ [e1, r e1 + t e4], [e2, r e2 + t e5], [e3, r e3 + t e6], \left[ e4, -\frac{r^2 + 1}{t} e1 - r e4 \right], \left[ e5, -\frac{r^2 + 1}{t} e2 - r e5 \right], \left[ e6, -\frac{r^2 + 1}{t} e3 - r e6 \right] \right] \quad (5.2)$$

```
> w1 := Pullback(Jt, ExteriorDerivative(w)) :
```

$$w1 := (3 r^2 t + 3 t^3) f1 \wedge f2 \wedge f3 - (3 r^3 + 3 t^2 r + 2 r) f1 \wedge f2 \wedge f6 + (3 r^3 + 3 t^2 r + 2 r) f1 \wedge f3 \wedge f5 + \frac{3 r^4 + 3 r^2 t^2 + 4 r^2 + 1}{t} f1 \wedge f5 \wedge f6 - (3 r^3 + 3 t^2 r + 2 r) f2 \wedge f3 \wedge f4 - \frac{3 r^4 + 3 r^2 t^2 + 4 r^2 + 1}{t} f2 \wedge f4 \wedge f6 \quad (5.3)$$

$$+ \frac{3r^4 + 3r^2t^2 + 4r^2 + 1}{t} f_3 \wedge f_4 \wedge f_5 - \frac{3r(r^4 + r^2t^2 + 2r^2 + 1)}{t^2} f_4 \wedge f_5 \wedge f_6$$

> w2 := Pullback(Jt, ExteriorDerivative(w1))

$$w2 := \frac{3r^4 + 6r^2t^2 + 3t^4 + 4r^2 + 1}{t} f_1 \wedge f_2 \wedge f_4 \wedge f_5 \quad (5.4)$$

$$+ \frac{3r^4 + 6r^2t^2 + 3t^4 + 4r^2 + 1}{t} f_1 \wedge f_3 \wedge f_4 \wedge f_6$$

$$+ \frac{3r^4 + 6r^2t^2 + 3t^4 + 4r^2 + 1}{t} f_2 \wedge f_3 \wedge f_5 \wedge f_6$$

> w3 := Pullback(Jt, ExteriorDerivative(w2))

$$w3 := -\frac{1}{p_1^2 t^3 p_2^2} (2(-p_1^2 t^2 p_2 - 2t^3 p_2^3 \varepsilon p_1^3 b + p_1^3 - t^4 p_2^2 p_1 + t^6 p_2^3 + 3r^4 p_1^3) \quad (5.5)$$

$$+ 3r^2 p_1^3 + r^6 p_1^3 + 3t^2 p_2 r^4 p_1^2 + 2t^2 p_2 r^2 p_1^2 + 3t^4 p_2^2 p_1 r^2 + \varepsilon p_1^2 t^5 p_2^4 b$$

$$+ 2\varepsilon p_1^3 t^3 p_2^3 r^2 b + \varepsilon p_1^4 t p_2^2 r^4 b + 2\varepsilon p_1^4 t p_2^2 b r^2 + \varepsilon p_1^4 t p_2^2 b)$$

$$f_1 \wedge f_2 \wedge f_3 \wedge f_4 \wedge f_5)$$

> w4 := Pullback(Jt, ExteriorDerivative(w3))

> DGinfo(w2, "CoefficientSet");

$$\left\{ \frac{3r^4 + 6r^2t^2 + 3t^4 + 4r^2 + 1}{t} \right\} \quad (5.6)$$

This is never zero, so no SKT cases here

### A3.1

> restart : with(DifferentialGeometry) : with(LieAlgebras) : with(Tensor) : with(Tools) :  
with(LinearAlgebra) :

We take  $p=p_1*i+p_2*j$  (always possible by an endomorphism)

> StructureEquations :=  $\left[ [ee, ii] = p_1 \cdot e, [ee, jj] = -p_2 \cdot e, [ii, kk] = -p_2 \cdot e, [jj, kk] = p_1 \cdot e, \right.$

$$[ee, ie] = \frac{\varepsilon}{2} \cdot ee + R \cdot p_1 \cdot ii + R \cdot p_2 \cdot jj, [ii, ie] = \frac{\varepsilon}{2} \cdot ii - R \cdot p_1 \cdot ee + R \cdot p_2 \cdot kk, [jj, ie]$$

$$= \frac{\varepsilon}{2} \cdot jj - R \cdot p_1 \cdot kk + R \cdot p_2 \cdot ee, [kk, ie] = \frac{\varepsilon}{2} \cdot kk + R \cdot p_1 \cdot jj + R \cdot p_2 \cdot ii, [e, ie] = \varepsilon \cdot e \left. \right]$$

$[ee, ii, jj, kk, e, ie] :$

$L := \text{LieAlgebraData}(\text{StructureEquations}, \text{VC});$

$$L := \left[ [e_1, e_2] = p_1 e_5, [e_1, e_3] = -p_2 e_5, [e_1, e_6] = R p_2 e_3 + R p_1 e_2 + \frac{1}{2} \varepsilon e_1, [e_2, e_4] = \quad (6.1)$$

$$-p_2 e_5, [e_2, e_6] = R p_2 e_4 + \frac{1}{2} \varepsilon e_2 - R p_1 e_1, [e_3, e_4] = p_1 e_5, [e_3, e_6] = -R p_1 e_4$$

$$+ \frac{1}{2} \varepsilon e_3 + R p_2 e_1, [e_4, e_6] = \frac{1}{2} \varepsilon e_4 + R p_2 e_2 + R p_1 e_3, [e_5, e_6] = \varepsilon e_5 \right]$$

> DGsetup(L, [e], [f]) : Query("Jacobi");

true

(6.2)

$$\begin{aligned} &> g := \text{evalDG}(b \cdot (f1 \&t f1 + f2 \&t f2 - f3 \&t f3 - f4 \&t f4) + (f5 \&t f5 + f6 \&t f6)); \\ &g := b f1 f1 + b f2 f2 - b f3 f3 - b f4 f4 + f5 f5 + f6 f6 \end{aligned} \quad (6.3)$$

We can always normalize by an endomorphism  $q=i$  on  $V$ . This is equivalent to  $\{r=0, t=1\}$  in the general parametrization of  $J$  below

$$\begin{aligned} &> J0 := \text{subs}(\{r=0, t=1\}, \text{Matrix}([ [0, -((1+r^2+t^2)/(2t)), -((1+r^2-t^2)/(2t)), -r, 0, 0], [ (1+r^2+t^2)/(2t), 0, r, -((1+r^2-t^2)/(2t)), 0, 0], [ -((1+r^2-t^2)/(2t)), r, 0, (1+r^2+t^2)/(2t), 0, 0], [ -r, -((1+r^2-t^2)/(2t)), -((1+r^2+t^2)/(2t)), 0, 0, 0], [0, 0, 0, 0, 0, -1], [0, 0, 0, 0, 1, 0]])); \\ &J0 := \begin{bmatrix} 0 & -1 & 0 & 0 & 0 & 0 \\ 1 & 0 & 0 & 0 & 0 & 0 \\ 0 & 0 & 0 & 1 & 0 & 0 \\ 0 & 0 & -1 & 0 & 0 & 0 \\ 0 & 0 & 0 & 0 & 0 & -1 \\ 0 & 0 & 0 & 0 & 1 & 0 \end{bmatrix} \end{aligned} \quad (6.4)$$

$$\begin{aligned} &> J := \text{convert}(J0, \text{DGtensor}, [[\text{"con\_bas"}, \text{"cov\_bas"}], [ ]]); \\ &> w := \text{convert}(\text{ContractIndices}(J, g, [[1, 1]]), \text{DGform}); \\ &w := b f1 \wedge f2 + b f3 \wedge f4 + f5 \wedge f6 \end{aligned} \quad (6.5)$$

$$\begin{aligned} &> Jt := \text{Transformation}(\text{VC}, \text{VC}, J0); \\ &> w1 := \text{Pullback}(Jt, \text{ExteriorDerivative}(w)); \\ &w1 := (\varepsilon b - p1) f1 \wedge f2 \wedge f5 - p2 f1 \wedge f3 \wedge f5 - 2 R p2 b f1 \wedge f4 \wedge f5 \\ &\quad + 2 R p2 b f2 \wedge f3 \wedge f5 - p2 f2 \wedge f4 \wedge f5 + (\varepsilon b - p1) f3 \wedge f4 \wedge f5 \end{aligned} \quad (6.6)$$

First let's check the Kahler condition

$$\begin{aligned} &> NJ := \text{TensorBrackets}(J, J, \text{"Frolicher-Nijenhuis"}); \\ \text{VC} &> \text{use RealDomain in } Slv := \text{solve}(\{op(\text{DGinfo}(w1, \text{"CoefficientSet"})), \\ &\quad op(\text{DGinfo}(NJ, \text{"CoefficientSet"})), b \neq 0, \varepsilon = 0, p1^2 + p2^2 \neq 0\}) \text{ end use} \\ &Slv := \end{aligned} \quad (6.7)$$

$$\begin{aligned} \text{VC} &> \text{use RealDomain in } Slv := \text{convert}(\text{solve}(\{op(\text{DGinfo}(w1, \text{"CoefficientSet"})), \\ &\quad op(\text{DGinfo}(NJ, \text{"CoefficientSet"})), b \neq 0, \varepsilon = 1\}), \text{radical}) \text{ end use} \\ &Slv := \{R=R, b=p1, p1=p1, p2=0, \varepsilon=1\} \end{aligned} \quad (6.8)$$

Now we are going to check SKT

$$\begin{aligned} &> w2 := \text{Pullback}(Jt, \text{ExteriorDerivative}(w1)); \\ &> w3 := \text{Pullback}(Jt, \text{ExteriorDerivative}(w2)); \\ &> w4 := \text{Pullback}(Jt, \text{ExteriorDerivative}(w3)); \\ &> \text{use RealDomain in } Slv := \text{solve}(\{op(\text{DGinfo}(w2, \text{"CoefficientSet"})), op(\text{DGinfo}(NJ, \\ &\quad \text{"CoefficientSet"})), b \neq 0, \varepsilon = 0\}) \text{ end use} \\ &Slv := \{R=R, b=b, p1=0, p2=0, \varepsilon=0\} \end{aligned} \quad (6.9)$$

$$\begin{aligned} &> \text{use RealDomain in } Slv := \text{solve}(\{op(\text{DGinfo}(w2, \text{"CoefficientSet"})), op(\text{DGinfo}(NJ, \\ &\quad \text{"CoefficientSet"})), b \neq 0, \varepsilon = 1\}) \text{ end use} \\ &Slv := \{R=R, b=p1, p1=p1, p2=0, \varepsilon=1\} \end{aligned} \quad (6.10)$$

The first case is flat, the second is Kahler, so there's no proper SKT for A3.1

## A3.2

[We will suppose  $p \neq 0$  (A3.2 for  $p=0$  is a subset of A3.4)]

$r \neq 0$

> restart : with(DifferentialGeometry) : with(LieAlgebras) : with(Tensor) : with(Tools) :

We normalize  $p=p*(ii+jj)$ ,  $r=r/p$

> StructureEquations :=  $\left[ [ee, ii] = p \cdot e, [ee, jj] = -p \cdot e, [ii, kk] = -p \cdot e, [jj, kk] = p \cdot e, [ee, e] \right.$   
 $= r \cdot (ii + jj), [ii, e] = -r \cdot (ee - kk), [jj, e] = r \cdot (ee - kk), [kk, e] = r \cdot (ii + jj), [ee, ie]$   
 $= \varepsilon \cdot ee + \lambda \cdot (ii + jj) - \frac{\varepsilon}{2} \cdot kk, [ii, ie] = \varepsilon \cdot ii - \lambda \cdot (ee - kk) + \frac{\varepsilon}{2} \cdot jj, [jj, ie] = \varepsilon \cdot jj + \lambda$   
 $\cdot (ee - kk) + \frac{\varepsilon}{2} \cdot ii, [kk, ie] = \varepsilon \cdot kk + \lambda \cdot (ii + jj) - \frac{\varepsilon}{2} \cdot ee, [e, ie] = \varepsilon \cdot e \left. \right], [ee, ii, jj, kk,$   
 $e, ie] :$

$L := \text{LieAlgebraData}(\text{StructureEquations}, \text{VC});$

$L := \left[ [e1, e2] = p \cdot e5, [e1, e3] = -p \cdot e5, [e1, e5] = e2 \cdot r + e3 \cdot r, [e1, e6] = -\frac{1}{2} \varepsilon \cdot e4 + \varepsilon \cdot e1 \right. \quad (7.1.1)$   
 $+ \lambda \cdot e2 + \lambda \cdot e3, [e2, e4] = -p \cdot e5, [e2, e5] = -e1 \cdot r + e4 \cdot r, [e2, e6] = \lambda \cdot e4 + \frac{1}{2} \varepsilon \cdot e3$   
 $- \lambda \cdot e1 + \varepsilon \cdot e2, [e3, e4] = p \cdot e5, [e3, e5] = e1 \cdot r - e4 \cdot r, [e3, e6] = -\lambda \cdot e4 + \varepsilon \cdot e3$   
 $+ \frac{1}{2} \varepsilon \cdot e2 + \lambda \cdot e1, [e4, e5] = e2 \cdot r + e3 \cdot r, [e4, e6] = \varepsilon \cdot e4 + \lambda \cdot e3 + \lambda \cdot e2 - \frac{1}{2} \varepsilon \cdot e1,$   
 $[e5, e6] = \varepsilon \cdot e5 \left. \right]$

> DGsetup(L, [e], [f]) : Query("Jacobi");  
 $\text{true} \quad (7.1.2)$

> g := evalDG((f1 &t f1 + f2 &t f2 - f3 &t f3 - f4 &t f4) + b \cdot (f5 &t f5 + f6 &t f6));  
 $g := f1 \cdot f1 + f2 \cdot f2 - f3 \cdot f3 - f4 \cdot f4 + b \cdot f5 \cdot f5 + b \cdot f6 \cdot f6 \quad (7.1.3)$

> J0 := Matrix([ [0, -(R^2 + t^2 + 1)/(2 \cdot t), -(R^2 - t^2 + 1)/(2 \cdot t), -R, 0, 0], [(R^2 + t^2 + 1)/(2 \cdot t), 0, R, -(R^2 - t^2 + 1)/(2 \cdot t), 0, 0], [-(R^2 - t^2 + 1)/(2 \cdot t), R, 0, (R^2 + t^2 + 1)/(2 \cdot t), 0, 0], [-R, -(R^2 - t^2 + 1)/(2 \cdot t), -(R^2 + t^2 + 1)/(2 \cdot t), 0, 0, 0], [0, 0, 0, 0, 0, -1], [0, 0, 0, 0, 1, 0]]);  
 $J0 := \quad (7.1.4)$

$$\begin{bmatrix} 0, -\frac{1}{2} \frac{R^2 + t^2 + 1}{t}, -\frac{1}{2} \frac{R^2 - t^2 + 1}{t}, -R, 0, 0, \\ \frac{1}{2} \frac{R^2 + t^2 + 1}{t}, 0, R, -\frac{1}{2} \frac{R^2 - t^2 + 1}{t}, 0, 0, \\ -\frac{1}{2} \frac{R^2 - t^2 + 1}{t}, R, 0, \frac{1}{2} \frac{R^2 + t^2 + 1}{t}, 0, 0 \end{bmatrix}$$



$$\begin{bmatrix} -R, -\frac{1}{2} \frac{R^2 - t^2 + 1}{t}, -\frac{1}{2} \frac{R^2 + t^2 + 1}{t}, 0, 0, 0 \end{bmatrix},$$

$$\begin{bmatrix} 0, 0, 0, 0, 0, -1 \end{bmatrix},$$

$$\begin{bmatrix} 0, 0, 0, 0, 1, 0 \end{bmatrix}]$$

>  $J := \text{Transformation}(\text{VC}, \text{VC}, J0) : \text{Jtensor} := \text{convert}(J0, \text{DGtensor}, [["\text{con\_bas}",$   
 $\text{"cov\_bas"}], [ ])$  :

>  $\omega := \text{convert}(\text{ContractIndices}(\text{Jtensor}, g, [[1, 1]]), \text{DGform})$ ;

$$\omega := \frac{R^2 + t^2 + 1}{2t} f1 \wedge f2 + \frac{R^2 - t^2 + 1}{2t} f1 \wedge f3 + R f1 \wedge f4 - R f2 \wedge f3$$

$$+ \frac{R^2 - t^2 + 1}{2t} f2 \wedge f4 + \frac{R^2 + t^2 + 1}{2t} f3 \wedge f4 + b f5 \wedge f6 \quad (7.1.5)$$

>  $\omega1 := \text{Pullback}(J, \text{ExteriorDerivative}(\omega))$  :

> **use RealDomain in**  $\text{solve}(\{op(\text{DGinfo}(\omega1, \text{"CoefficientSet"})), b \neq 0\})$  **end use**  
 $\{R=R, b=b, p=0, r=0, t=t, \varepsilon=0, \lambda=0\}$  (7.1.6)

This corresponds to the flat case, so no Kahler structures here

>  $\omega2 := \text{Pullback}(J, \text{ExteriorDerivative}(\omega1))$  :

> **use RealDomain in**  $\text{solve}(\{op(\text{DGinfo}(\omega2, \text{"CoefficientSet"})), b \neq 0\})$  **end use**  
 $\left\{ R = \frac{\lambda}{b p}, b=b, p=p, r=\text{RootOf}(\_Z^2 - 3, \text{label}=\_L61) p b, t=t, \varepsilon = \frac{2(b^2 p^2 + \lambda^2)}{b p t}, \right.$  (7.1.7)  
 $\left. \lambda = \lambda \right\}$

>  $\text{solve}(\{op(\text{DGinfo}(\omega2, \text{"CoefficientSet"})), b \neq 0\})$   
 $\{R=R, b=b, p=0, r=r, t=t, \varepsilon=0, \lambda=\text{RootOf}(\_Z^2 + 1) r\}, \{R=\text{RootOf}(\_Z^2 + 1), b$  (7.1.8)  
 $=b, p=p, r=r, t=t, \varepsilon=0, \lambda=\lambda\}$

No real solutions, so no SKT

▼ **r=0**

>  $\text{restart} : \text{with}(\text{DifferentialGeometry}) : \text{with}(\text{LieAlgebras}) : \text{with}(\text{Tensor}) : \text{with}(\text{Tools}) :$   
 $\text{with}(\text{LinearAlgebra}) :$

>  $\text{StructureEquations} := \left[ [ee, ii] = p \cdot e, [ee, jj] = -p \cdot e, [ii, kk] = -p \cdot e, [jj, kk] = p \cdot e, [ee, ie] \right.$   
 $= (\varepsilon + s) \cdot ee + \lambda \cdot (ii + jj) - \frac{\varepsilon + 2s}{2} \cdot kk, [ii, ie] = (\varepsilon + s) \cdot ii - \lambda \cdot (ee - kk)$   
 $+ \frac{\varepsilon + 2s}{2} \cdot jj, [jj, ie] = (\varepsilon + s) \cdot jj + \lambda \cdot (ee - kk) + \frac{\varepsilon + 2s}{2} \cdot ii, [kk, ie] = (\varepsilon + s) \cdot kk$   
 $\left. + \lambda \cdot (ii + jj) - \frac{\varepsilon + 2s}{2} \cdot ee, [e, ie] = \varepsilon \cdot e \right], [ee, ii, jj, kk, e, ie] :$

$L := \text{LieAlgebraData}(\text{StructureEquations}, \text{VC});$

$$L := \left[ [e1, e2] = p e5, [e1, e3] = -p e5, [e1, e6] = \left( -\frac{1}{2} \varepsilon - s \right) e4 + \lambda e3 + \lambda e2 + (\varepsilon + s) e1, [e2, e4] = -p e5, [e2, e6] = \lambda e4 + \left( \frac{1}{2} \varepsilon + s \right) e3 + (\varepsilon + s) e2 - \lambda e1, [e3, e4] = p e5, [e3, e6] = -\lambda e4 + (\varepsilon + s) e3 + \left( \frac{1}{2} \varepsilon + s \right) e2 + \lambda e1, [e4, e6] = (\varepsilon + s) e4 + \lambda e3 + \lambda e2 + \left( -\frac{1}{2} \varepsilon - s \right) e1, [e5, e6] = \varepsilon e5 \right] \quad (7.2.1)$$

$$> \text{DGsetup}(L, [e], [f]) : \text{Query}(\text{"Jacobi"}); \quad \text{true} \quad (7.2.2)$$

$$> g := \text{evalDG}((f1 \&t f1 + f2 \&t f2 - f3 \&t f3 - f4 \&t f4) + b \cdot (f5 \&t f5 + f6 \&t f6)); \\ g := f1 f1 + f2 f2 - f3 f3 - f4 f4 + b f5 f5 + b f6 f6 \quad (7.2.3)$$

$$> J0 := \text{Matrix}([ [0, -((1 + r^2 + t^2)/(2t)), -((1 + r^2 - t^2)/(2t)), -r, 0, 0], [ (1 + r^2 + t^2)/(2t), 0, r, -((1 + r^2 - t^2)/(2t)), 0, 0], [ -((1 + r^2 - t^2)/(2t)), r, 0, (1 + r^2 + t^2)/(2t), 0, 0], [ -r, -((1 + r^2 - t^2)/(2t)), -((1 + r^2 + t^2)/(2t)), 0, 0, 0], [0, 0, 0, 0, 0, -1], [0, 0, 0, 0, 1, 0]]); \\ J0 := \quad (7.2.4)$$

$$\begin{bmatrix} 0, -\frac{1}{2} \frac{r^2 + t^2 + 1}{t}, -\frac{1}{2} \frac{r^2 - t^2 + 1}{t}, -r, 0, 0, \\ \frac{1}{2} \frac{r^2 + t^2 + 1}{t}, 0, r, -\frac{1}{2} \frac{r^2 - t^2 + 1}{t}, 0, 0, \\ -\frac{1}{2} \frac{r^2 - t^2 + 1}{t}, r, 0, \frac{1}{2} \frac{r^2 + t^2 + 1}{t}, 0, 0, \\ -r, -\frac{1}{2} \frac{r^2 - t^2 + 1}{t}, -\frac{1}{2} \frac{r^2 + t^2 + 1}{t}, 0, 0, 0, \\ 0, 0, 0, 0, 0, -1, \\ 0, 0, 0, 0, 1, 0 \end{bmatrix}$$

$$> J := \text{Transformation}(\text{VC}, \text{VC}, J0) : \text{Jtensor} := \text{convert}(J0, \text{DGtensor}, [ ["con\_bas", "cov\_bas"], [ ]]);$$

$$> \omega := \text{convert}(\text{ContractIndices}(\text{Jtensor}, g, [[1, 1]]), \text{DGform});$$

$$\omega := \frac{r^2 + t^2 + 1}{2t} f1 \wedge f2 + \frac{r^2 - t^2 + 1}{2t} f1 \wedge f3 + r f1 \wedge f4 - r f2 \wedge f3 \\ + \frac{r^2 - t^2 + 1}{2t} f2 \wedge f4 + \frac{r^2 + t^2 + 1}{2t} f3 \wedge f4 + b f5 \wedge f6 \quad (7.2.5)$$

$$> \text{NJ} := \text{TensorBrackets}(\text{Jtensor}, \text{Jtensor}, \text{"Frolicher-Nijenhuis"});$$

$$> \omega1 := \text{Pullback}(J, \text{ExteriorDerivative}(\omega));$$

$$> \text{use RealDomain in solve}(\{ \text{op}(\text{DGinfo}(\omega1, \text{"CoefficientSet"})), \text{op}(\text{DGinfo}(\text{NJ}, \text{"CoefficientSet"})), b \neq 0 \}); \text{end use} \\ \{b = b, p = 0, r = r, s = 0, t = t, \varepsilon = 0, \lambda = 0\} \quad (7.2.6)$$

No solutions because p is nonzero

```
>  $\omega_2 := \text{Pullback}(J, \text{ExteriorDerivative}(\omega_1)) :$ 
> use RealDomain in solve( {op(DGinfo( $\omega_2$ , "CoefficientSet")), op(DGinfo( $\omega_1$ ,
"CoefficientSet"))}, b  $\neq$  0,  $\epsilon=0$ ); end use
{b = b, p = 0, r = r, s = 0, t = t,  $\epsilon=0$ ,  $\lambda=0$ }
```

(7.2.7)

```
> use RealDomain in Slv := solve( {op(DGinfo( $\omega_2$ , "CoefficientSet")), op(DGinfo(NJ,
"CoefficientSet"))}, b  $\neq$  0,  $\epsilon=1$ ); end use
Slv :=
```

(7.2.8)

### A3.3

Free imaginary split quaternion  $s$  are parameterised as  $p = M \cdot i + L \cdot j + K \cdot k$ ,  $u = \alpha_1 \cdot i + \alpha_2 \cdot j + \alpha_3 \cdot k$

```
> restart : with(DifferentialGeometry) : with(LieAlgebras) : with(Tensor) : with(Tools) :
with(LinearAlgebra) :
```

```
> StructureEquations := [[ee, ii] =  $\alpha_1 \cdot e + M \cdot ie$ , [ee, jj] =  $-\alpha_2 \cdot e - L \cdot ie$ , [ee, kk] =  $-\alpha_3 \cdot e - K$ 
 $\cdot ie$ , [ii, jj] =  $\alpha_3 \cdot e + K \cdot ie$ , [ii, kk] =  $-\alpha_2 \cdot e - L \cdot ie$ , [jj, kk] =  $\alpha_1 \cdot e + M \cdot ie$ ], [ee, ii, jj, kk, e,
ie] :
```

```
> LL := LieAlgebraData(StructureEquations, VC) : DGsetup(LL, [e], [f]) ;
```

Lie algebra: VC

(8.1)

```
> g := evalDG((f1 &t f1 + f2 &t f2 - f3 &t f3 - f4 &t f4) + b · (f5 &t f5 + f6 &t f6)) ;
```

$g := f_1 f_1 + f_2 f_2 - f_3 f_3 - f_4 f_4 + b f_5 f_5 + b f_6 f_6$

(8.2)

To avoid complicated expressions we can use the endomorphism freedom to fix  $q=i$ , i.e.  $t=1, r=0$

```
> J0 := subs({t = 1, r = 0}, Matrix([ [0, -((1 + r^2 + t^2)/(2 t)), -((1 + r^2 - t^2)/(2 t)), -r, 0, 0], [ (
1 + r^2 + t^2)/(2 t), 0, r, -((1 + r^2 - t^2)/(2 t)), 0, 0], [ -((1 + r^2 - t^2)/(2 t)), r, 0, (1 + r^2 + t^2)/(2 t), 0, 0], [ -r, -((1 + r^2 - t^2)/(2 t)), -((1 + r^2 + t
^2)/(2 t)), 0, 0, 0], [0, 0, 0, 0, 0, -1], [0, 0, 0, 0, 1, 0]])) ;
```

$$J_0 := \begin{bmatrix} 0 & -1 & 0 & 0 & 0 & 0 \\ 1 & 0 & 0 & 0 & 0 & 0 \\ 0 & 0 & 0 & 1 & 0 & 0 \\ 0 & 0 & -1 & 0 & 0 & 0 \\ 0 & 0 & 0 & 0 & 0 & -1 \\ 0 & 0 & 0 & 0 & 1 & 0 \end{bmatrix}$$

(8.3)

```
> J := Transformation(VC, VC, J0) : Jtensor := convert(J0, DGtensor, [{"con_bas",
"cov_bas"}, [ ]]) :
```

```
>  $\omega := \text{convert}(\text{ContractIndices}(Jtensor, g, [[1, 1]]), \text{DGform}) ;$ 
```

$\omega := f_1 \wedge f_2 + f_3 \wedge f_4 + b f_5 \wedge f_6$

(8.4)

```
>  $\omega_1 := \text{Pullback}(J, \text{ExteriorDerivative}(\omega)) ;$ 
```

$\omega_1 := -\alpha_1 b f_1 \wedge f_2 \wedge f_5 - M b f_1 \wedge f_2 \wedge f_6 - \alpha_2 b f_1 \wedge f_3 \wedge f_5 - L b f_1 \wedge f_3 \wedge f_6$   
 $- \alpha_3 b f_1 \wedge f_4 \wedge f_5 - K b f_1 \wedge f_4 \wedge f_6 + \alpha_3 b f_2 \wedge f_3 \wedge f_5 + K b f_2 \wedge f_3 \wedge f_6$

(8.5)

```

--  $\omega_2 := \text{Pullback}(J, \text{ExteriorDerivative}(\omega_1));$ 
 $\omega_2 := (2 M^2 b + 2 L^2 b + 2 K^2 b + 2 \alpha^2 b + 2 \alpha^2 b + 2 \alpha^3 b) f_1 \wedge f_2 \wedge f_3 \wedge f_4$  (8.6)
--  $\omega_3 := \text{Pullback}(J, \text{ExteriorDerivative}(\omega_2));$ 
 $\omega_3 := 0 f_1 \wedge f_2 \wedge f_3 \wedge f_4 \wedge f_5$  (8.7)
--  $NJ := \text{TensorBrackets}(J\text{tensor}, J\text{tensor}, \text{"Frolicher-Nijenhuis"}) :$ 
--  $KaehlerEq := DGinfo(\text{ExteriorDerivative}(\omega), \text{"CoefficientSet"}) ;$ 
 $KaehlerEq := \{K b, M b, \alpha_2 b, \alpha_3 b, -K b, -L b, -\alpha b, -\alpha_3 b\}$  (8.8)
--  $SumKaehlerEq := \text{add}(KaehlerEq[i]^2, i = 1 .. \text{nops}(KaehlerEq)) ;$ 
 $SumKaehlerEq := 2 K^2 b^2 + M^2 b^2 + \alpha^2 b^2 + 2 \alpha^3 b^2 + L^2 b^2 + \alpha^2 b^2$  (8.9)
-- use RealDomain in sols := solve( { op(DGinfo(  $\omega_2$ , "CoefficientSet" ) ), op(DGinfo(NJ, "CoefficientSet" ) ),  $b \neq 0$  } ) end use
sols := {  $K = -\alpha^2, L = \alpha^3, M = \text{RootOf}(\_Z^2 + 2 \alpha^3^2 + 2 \alpha^2^2 + \alpha^2^2), \alpha = \alpha, \alpha_2 = \alpha_2, \alpha_3 = \alpha_3, b = b$  } (8.10)

```

This corresponds (in the real case) to  $\alpha = \alpha_2 = K = L = M = 0$ , so the case is flat (non-interesting).  
Conclusion: no SKT for this case.

Let us make a comment on why A1.2 has SKT structures, while A2.3 (which is similar in formulae to A1.2) has none. The space of complex structures on V in the first case is the sphere  $S^2$  and the space of SKT is a circle  $S^1$  in it (if we fix  $u=i$ ). In the second case the space of complex structures is a pseudosphere (two-sheet hyperboloid diffeomorphic to the disjoint union of two balls  $\mathbb{R}^2 \times B^2$ ). In this case the circle  $S^1$  is imaginary, meaning it meets the real pseudosphere by the empty set. A similar situation happens with A3.5 (vs. A1.4) structures wrt the higher analogs of the SKT condition.

## A3.4

$\epsilon=p=0$

```

-- restart : with(DifferentialGeometry) : with(LieAlgebras) : with(Tensor) : with(Tools) :
-- with(LinearAlgebra) :
-- We let  $u=u_1 \cdot i + u_2 \cdot j$  (by an endomorphism)
-- StructureEquations := [ [ee, e] =  $\alpha \cdot ee$ , [ii, e] =  $\alpha \cdot ii$ , [jj, e] =  $\alpha \cdot jj$ , [kk, e] =  $\alpha \cdot kk$ , [ee, ie]
-- =  $\beta \cdot ee + u_1 \cdot ii + u_2 \cdot jj$ , [ii, ie] =  $\beta \cdot ii - u_1 \cdot ee + u_2 \cdot kk$ , [jj, ie] =  $\beta \cdot jj - u_1 \cdot kk + u_2 \cdot ee$ ,
-- [kk, ie] =  $\beta \cdot kk + u_1 \cdot jj + u_2 \cdot ii$  ] :
-- L := LieAlgebraData(StructureEquations, [ee, ii, jj, kk, e, ie], VC) : DGsetup(L, [e], [f])
-- Lie algebra: VC (9.1.1)
-- Query("Jacobi")
-- true (9.1.2)
-- g := evalDG( (f1 &t f1 + f2 &t f2 - f3 &t f3 - f4 &t f4) + b \cdot (f5 &t f5 + f6 &t f6) );
-- g := f1 f1 + f2 f2 - f3 f3 - f4 f4 + b f5 f5 + b f6 f6 (9.1.3)
-- J0 := Matrix( [ [0, -((1 + r^2 + t^2)/(2 t)), -((1 + r^2 - t^2)/(2 t)), -r, 0, 0], [ (

```

$$1 + r^2 + t^2) / (2t), 0, r, -((1 + r^2 - t^2) / (2t)), 0, 0], [ -((1 + r^2 - t^2) / (2t)), r, 0, (1 + r^2 + t^2) / (2t), 0, 0], [-r, -((1 + r^2 - t^2) / (2t)), -((1 + r^2 + t^2) / (2t)), 0, 0, 0], [0, 0, 0, 0, 0, -1], [0, 0, 0, 0, 1, 0]]);$$

$$J0 := \quad (9.1.4)$$

$$\begin{aligned} & \left[ \left[ 0, -\frac{1}{2} \frac{r^2 + t^2 + 1}{t}, -\frac{1}{2} \frac{r^2 - t^2 + 1}{t}, -r, 0, 0 \right], \right. \\ & \left[ \frac{1}{2} \frac{r^2 + t^2 + 1}{t}, 0, r, -\frac{1}{2} \frac{r^2 - t^2 + 1}{t}, 0, 0 \right], \\ & \left[ -\frac{1}{2} \frac{r^2 - t^2 + 1}{t}, r, 0, \frac{1}{2} \frac{r^2 + t^2 + 1}{t}, 0, 0 \right], \\ & \left[ -r, -\frac{1}{2} \frac{r^2 - t^2 + 1}{t}, -\frac{1}{2} \frac{r^2 + t^2 + 1}{t}, 0, 0, 0 \right], \\ & \left[ 0, 0, 0, 0, 0, -1 \right], \\ & \left. \left[ 0, 0, 0, 0, 1, 0 \right] \right] \end{aligned}$$

$$> J := \text{Transformation}(VC, VC, J0) : Jtensor := \text{convert}(J0, DGtensor, [ ["con\_bas", "cov\_bas"], [ ] ]):$$

$$> \omega := \text{convert}(\text{ContractIndices}(Jtensor, g, [[1, 1]]), DGform);$$

$$\begin{aligned} \omega := & \frac{r^2 + t^2 + 1}{2t} f1 \wedge f2 + \frac{r^2 - t^2 + 1}{2t} f1 \wedge f3 + r f1 \wedge f4 - r f2 \wedge f3 \\ & + \frac{r^2 - t^2 + 1}{2t} f2 \wedge f4 + \frac{r^2 + t^2 + 1}{2t} f3 \wedge f4 + b f5 \wedge f6 \end{aligned} \quad (9.1.5)$$

$$> \omega1 := \text{Pullback}(J, \text{ExteriorDerivative}(\omega));$$

$$\begin{aligned} \omega1 := & \frac{r^2 \beta - 2 u2 r t + t^2 \beta + \beta}{t} f1 \wedge f2 \wedge f5 - \frac{\alpha (r^2 + t^2 + 1)}{t} f1 \wedge f2 \wedge f6 \\ & + \frac{r^2 \beta + 2 u1 r t - t^2 \beta + \beta}{t} f1 \wedge f3 \wedge f5 - \frac{\alpha (r^2 - t^2 + 1)}{t} f1 \wedge f3 \wedge f6 \\ & - \frac{r^2 u1 + r^2 u2 - 2 r t \beta - t^2 u1 + t^2 u2 + u1 + u2}{t} f1 \wedge f4 \wedge f5 \\ & - 2 \alpha r f1 \wedge f4 \wedge f6 \\ & + \frac{r^2 u1 + r^2 u2 - 2 r t \beta - t^2 u1 + t^2 u2 + u1 + u2}{t} f2 \wedge f3 \wedge f5 \\ & + 2 \alpha r f2 \wedge f3 \wedge f6 + \frac{r^2 \beta + 2 r t u1 - t^2 \beta + \beta}{t} f2 \wedge f4 \wedge f5 \\ & - \frac{\alpha (r^2 - t^2 + 1)}{t} f2 \wedge f4 \wedge f6 + \frac{r^2 \beta - 2 r t u2 + t^2 \beta + \beta}{t} f3 \wedge f4 \wedge f5 \\ & - \frac{\alpha (r^2 + t^2 + 1)}{t} f3 \wedge f4 \wedge f6 \end{aligned} \quad (9.1.6)$$

$$> \omega2 := \text{Pullback}(J, \text{ExteriorDerivative}(\omega1)) :$$

$$\begin{aligned} &> \omega 3 := \text{Pullback}(J, \text{ExteriorDerivative}(\omega 2)); \\ &\quad \omega 3 := 0 f1 \wedge f2 \wedge f3 \wedge f4 \wedge f5 \end{aligned} \quad (9.1.7)$$

$$\begin{aligned} &> \text{KaehlerEq} := \text{DGinfo}(\text{ExteriorDerivative}(\omega), \text{"CoefficientSet"}); \\ \text{KaehlerEq} &:= \left\{ \frac{r^2 \beta - 2 r t u1 - t^2 \beta + \beta}{t}, \frac{r^2 \beta + 2 r t u2 + t^2 \beta + \beta}{t}, \right. \\ &\quad \frac{r^2 u1 + r^2 u2 + 2 r t \beta - t^2 u1 + t^2 u2 + u1 + u2}{t}, \frac{\alpha (r^2 - t^2 + 1)}{t}, \\ &\quad \left. \frac{\alpha (r^2 + t^2 + 1)}{t}, -2 \alpha r, 2 \alpha r, -\frac{r^2 u1 + r^2 u2 + 2 r t \beta - t^2 u1 + t^2 u2 + u1 + u2}{t} \right\} \end{aligned} \quad (9.1.8)$$

$$\begin{aligned} &> \text{use RealDomain in sols} := \text{solve}(\{op(\text{KaehlerEq}), u1^2 + u2^2 + \alpha^2 + \beta^2 \neq 0\}) \text{ end use} \\ \text{sols} &:= \left\{ r=0, t=t, u1 = \frac{u2 (t^2 + 1)}{t^2 - 1}, u2 = u2, \alpha = 0, \beta = 0 \right\}, \{r=0, t=1, u1 = u1, u2 \\ &= 0, \alpha = 0, \beta = 0\}, \{r=0, t=-1, u1 = u1, u2 = 0, \alpha = 0, \beta = 0\} \end{aligned} \quad (9.1.9)$$

$$\begin{aligned} \text{VC} &> \text{simplify} \left( - \left( \frac{u2 (t^2 + 1)}{t^2 - 1} \right)^2 + u2^2 \right) \\ &\quad - \frac{4 t^2 u2^2}{(t^2 - 1)^2} \end{aligned} \quad (9.1.10)$$

$$\begin{aligned} &> \text{use RealDomain in sols} := \text{solve}(\{op(\text{KaehlerEq}), u2 = 0, u1^2 + \alpha^2 + \beta^2 \neq 0\}) \text{ end use} \\ \text{sols} &:= \{r=0, t=1, u1 = u1, u2 = 0, \alpha = 0, \beta = 0\}, \{r=0, t=-1, u1 = u1, u2 = 0, \alpha = 0, \beta \\ &= 0\} \end{aligned} \quad (9.1.11)$$

This gives the Kahler structure for A3.4 (we used endomorphism freedom to rotate u to R\*i, i.e. to have u2=0, since u^2<0). Up to endomorphism freedom (we can fix now q=i, i.e. r=0,t=1) we get: q=i, u=r\*i, all other parameters are zero.

$$\begin{aligned} &> \text{SumKaehlerEq} := \text{add}(\text{KaehlerEq}[i]^2, i = 1 .. \text{nops}(\text{KaehlerEq})); \\ \text{SumKaehlerEq} &:= \frac{(r^2 \beta - 2 r t u1 - t^2 \beta + \beta)^2}{t^2} + \frac{(r^2 \beta + 2 r t u2 + t^2 \beta + \beta)^2}{t^2} \\ &\quad + \frac{2 (r^2 u1 + r^2 u2 + 2 r t \beta - t^2 u1 + t^2 u2 + u1 + u2)^2}{t^2} + \frac{\alpha^2 (r^2 - t^2 + 1)^2}{t^2} \\ &\quad + \frac{\alpha^2 (r^2 + t^2 + 1)^2}{t^2} + 8 r^2 \alpha^2 \end{aligned} \quad (9.1.12)$$

$$\begin{aligned} &> \text{NJ} := \text{TensorBrackets}(\text{Jtensor}, \text{Jtensor}, \text{"Frolicher-Nijenhuis"}); \\ &> \text{use RealDomain in sols} := \text{solve}(\{op(\text{DGinfo}(\omega 2, \text{"CoefficientSet"})), op(\text{DGinfo}(\text{NJ}, \\ &\quad \text{"CoefficientSet"})), \text{SumKaehlerEq} \neq 0\}) \text{ end use} \\ &\quad \text{sols} := \end{aligned} \quad (9.1.13)$$

No solutions

$\epsilon=1, [p,u]=p, p^2=0, \alpha=0$

> restart : with(DifferentialGeometry) : with(LieAlgebras) : with(Tensor) : with(Tools) :  
with(LinearAlgebra) :

Use the endomorphism freedom to rotate  $q$  to  $i$ . The remaining freedom is the rotation in the  $\langle j, k \rangle$  plane. We use this to fix the projection of  $p$  to  $\langle j, k \rangle$  along  $i$  to be in the direction  $\langle j \rangle$ . Thus we fix the parameters:  $p=p*(i+j), u=u0*(i+j)-(1/2)*k$  (the last condition is coming from the constraint  $[p,u]=p$  provided  $p \neq 0$ ).

> StructureEquations :=  $\left[ [ee, e] = p \cdot (ii + jj), [ii, e] = -p \cdot (ee - kk), [jj, e] = p \cdot (ee - kk), \right.$   
 $[kk, e] = p \cdot (ii + jj), [ee, ie] = \beta \cdot ee + u0 \cdot (ii + jj) - \frac{1}{2} \cdot kk, [ii, ie] = \beta \cdot ii - u0 \cdot (ee$   
 $- kk) + \frac{1}{2} \cdot jj, [jj, ie] = \beta \cdot jj + u0 \cdot (ee - kk) + \frac{1}{2} \cdot ii, [kk, ie] = \beta \cdot kk + u0 \cdot (ii + jj)$   
 $\left. - \frac{1}{2} \cdot ee, [e, ie] = e \right] :$

> L := LieAlgebraData(StructureEquations, [ee, ii, jj, kk, e, ie], VC) : DGsetup(L, [e],  
[f]) : Query("Jacobi")

true (9.2.1)

> g := evalDG((f1 &t f1 + f2 &t f2 - f3 &t f3 - f4 &t f4) + b \cdot (f5 &t f5 + f6 &t f6));  
g := f1 f1 + f2 f2 - f3 f3 - f4 f4 + b f5 f5 + b f6 f6 (9.2.2)

> J0 := subs({r=0, t=1}, Matrix([ [0, -((1 + r^2 + t^2)/(2 t)), -((1 + r^2 - t^2)/(2 t)), -r, 0, 0], [ (1 + r^2 + t^2)/(2 t), 0, r, -((1 + r^2 - t^2)/(2 t)), 0, 0], [ -((1 + r^2 - t^2)/(2 t)), r, 0, (1 + r^2 + t^2)/(2 t), 0, 0], [ -r, -((1 + r^2 - t^2)/(2 t)), -((1 + r^2 + t^2)/(2 t)), 0, 0, 0], [0, 0, 0, 0, 0, -1], [0, 0, 0, 0, 1, 0]]))

$$J0 := \begin{bmatrix} 0 & -1 & 0 & 0 & 0 & 0 \\ 1 & 0 & 0 & 0 & 0 & 0 \\ 0 & 0 & 0 & 1 & 0 & 0 \\ 0 & 0 & -1 & 0 & 0 & 0 \\ 0 & 0 & 0 & 0 & 0 & -1 \\ 0 & 0 & 0 & 0 & 1 & 0 \end{bmatrix} \quad (9.2.3)$$

> J := Transformation(VC, VC, J0) : Jtensor := convert(J0, DGtensor, [ ["con\_bas",  
"cov\_bas"], [ ]]) :

>  $\omega := \text{convert}(\text{ContractIndices}(Jtensor, g, [[1, 1]]), DGform);$

$\omega := f1 \wedge f2 + f3 \wedge f4 + b f5 \wedge f6$  (9.2.4)

>  $\omega1 := \text{Pullback}(J, \text{ExteriorDerivative}(\omega));$

$\omega1 := 2 \beta f1 \wedge f2 \wedge f5 - f1 \wedge f3 \wedge f5 - 2 u0 f1 \wedge f4 \wedge f5 + 2 p f1 \wedge f4 \wedge f6$   
 $+ 2 u0 f2 \wedge f3 \wedge f5 - 2 p f2 \wedge f3 \wedge f6 - f2 \wedge f4 \wedge f5 + 2 \beta f3 \wedge f4 \wedge f5$  (9.2.5)

>  $\omega2 := \text{Pullback}(J, \text{ExteriorDerivative}(\omega1));$

$\omega2 := (4 p^2 + 4 u0^2 - 4 \beta^2 - 2 \beta + 1) f1 \wedge f2 \wedge f5 \wedge f6 + (4 p^2 + 4 u0^2$   
 $- 1) f1 \wedge f3 \wedge f5 \wedge f6 - 4 u0 f1 \wedge f4 \wedge f5 \wedge f6 + 4 u0 f2 \wedge f3 \wedge f5 \wedge f6 + (4 p^2$  (9.2.6)

$$\begin{aligned}
& + 4 u^2 - 1) f_2 \wedge f_4 \wedge f_5 \wedge f_6 + (4 p^2 + 4 u^2 - 4 \beta^2 - 2 \beta \\
& + 1) f_3 \wedge f_4 \wedge f_5 \wedge f_6 \\
& \omega_3 := \text{Pullback}(J, \text{ExteriorDerivative}(\omega_2)); \\
& \omega_3 := 0 f_1 \wedge f_2 \wedge f_3 \wedge f_4 \wedge f_5
\end{aligned} \tag{9.2.7}$$

$$\begin{aligned}
& NJ := \text{TensorBrackets}(J\text{tensor}, J\text{tensor}, \text{"Frolicher-Nijenhuis"}) \\
& NJ := -4 u_0 e_3 f_2 f_5 - 4 u_0 e_3 f_1 f_6 - (4 p - 2) e_3 f_1 f_5 + (4 p - 2) e_4 f_5 f_2 \\
& - 4 u_0 e_4 f_5 f_1 - 4 u_0 e_4 f_2 f_6 - (4 p - 2) e_1 f_3 f_5 + (4 p - 2) e_1 f_5 f_3 - (4 p \\
& - 2) e_1 f_4 f_6 + 4 u_0 e_2 f_6 f_4 - (4 p - 2) e_2 f_6 f_3 + 4 u_0 e_1 f_4 f_5 - 4 u_0 e_1 f_3 f_6 \\
& - (4 p - 2) e_2 f_4 f_5 + (4 p - 2) e_2 f_3 f_6 - 4 u_0 e_1 f_5 f_4 + (4 p - 2) e_2 f_5 f_4 \\
& + 4 u_0 e_2 f_5 f_3 - 4 u_0 e_2 f_4 f_6 - (4 p - 2) e_3 f_6 f_2 + 4 u_0 e_3 f_6 f_1 + 4 u_0 e_4 f_6 f_2 \\
& + (4 p - 2) e_4 f_6 f_1 + 4 u_0 e_3 f_5 f_2 - 4 u_0 e_2 f_3 f_5 + (4 p - 2) e_3 f_5 f_1 + (4 p \\
& - 2) e_3 f_2 f_6 - (4 p - 2) e_4 f_2 f_5 - (4 p - 2) e_4 f_1 f_6 + 4 u_0 e_4 f_1 f_5 + (4 p \\
& - 2) e_1 f_6 f_4 + 4 u_0 e_1 f_6 f_3
\end{aligned} \tag{9.2.8}$$

$$\begin{aligned}
& KaehlerEq := DGinfo(\text{ExteriorDerivative}(\omega), \text{"CoefficientSet"}); \\
& KaehlerEq := \{1, -2 p, 2 p, -2 u_0, 2 u_0, 2 \beta\}
\end{aligned} \tag{9.2.9}$$

$$\begin{aligned}
& \text{use RealDomain in sols} := \text{solve}(\{op(DGinfo(\omega_2, \text{"CoefficientSet"})), op(DGinfo(NJ, \\
& \text{"CoefficientSet"}))\}) \text{ end use} \\
& sols := \left\{ p = \frac{1}{2}, u_0 = 0, \beta = -1 \right\}, \left\{ p = \frac{1}{2}, u_0 = 0, \beta = \frac{1}{2} \right\}
\end{aligned} \tag{9.2.10}$$

Thus the SKT case (here we have no Kahler structure) corresponds to ( $\beta$  has two possibilities):  
 $p = \frac{1}{2}(i+j), u = \frac{-1}{2}k, \alpha = 0, \left[ \beta = -1 \text{ or } \beta = \frac{1}{2} \right], \varepsilon = 1, J = i.$

Now we consider the final case  $p=0, \varepsilon=1$ , when  $u$  can be transformed by an endomorphism to  $u_1 \cdot ii + u_2 \cdot j$ . The complex structure continues to be  $q=i$ .

$$\begin{aligned}
& \text{StructureEquations} := [[ee, ie] = \beta \cdot ee + u_1 \cdot ii + u_2 \cdot jj, [ii, ie] = \beta \cdot ii - u_1 \cdot ee + u_2 \cdot kk, [jj, \\
& ie] = \beta \cdot jj + u_2 \cdot ee - u_1 \cdot kk, [kk, ie] = \beta \cdot kk + u_2 \cdot ii + u_1 \cdot jj, [e, ie] = e]: \\
& L := \text{LieAlgebraData}(\text{StructureEquations}, [ee, ii, jj, kk, e, ie], VC) : DGsetup(L, [e], \\
& [f]) : \text{Query}(\text{"Jacobi"})
\end{aligned} \tag{9.2.11}$$

$$\begin{aligned}
& g := \text{evalDG}((f_1 \&t f_1 + f_2 \&t f_2 - f_3 \&t f_3 - f_4 \&t f_4) + b \cdot (f_5 \&t f_5 + f_6 \&t f_6)); \\
& g := f_1 f_1 + f_2 f_2 - f_3 f_3 - f_4 f_4 + b f_5 f_5 + b f_6 f_6
\end{aligned} \tag{9.2.12}$$

$$\begin{aligned}
& J0 := \text{subs}(\{r=0, t=1\}, \text{Matrix}([ [0, -((1 + r^2 + t^2)/(2 t)), -((1 + r^2 - t^2) \\
& / (2 t)), -r, 0, 0], [ ( \\
& 1 + r^2 + t^2)/(2 t), 0, r, -((1 + r^2 - t^2)/(2 t)), 0, 0], [ -((1 + r^2 - t^2)/(2 t)), r, 0, (1 + r^2 + t^2)/(2 t), 0, 0], [ -r, -((1 + r^2 - t^2)/(2 t)), -((1 + r^2 \\
& + t^2)/(2 t)), 0, 0, 0], [0, 0, 0, 0, 0, -1], [0, 0, 0, 0, 1, 0]]))
\end{aligned} \tag{9.2.13}$$



$$J0 := \begin{bmatrix} 0 & -1 & 0 & 0 & 0 & 0 \\ 1 & 0 & 0 & 0 & 0 & 0 \\ 0 & 0 & 0 & 1 & 0 & 0 \\ 0 & 0 & -1 & 0 & 0 & 0 \\ 0 & 0 & 0 & 0 & 0 & -1 \\ 0 & 0 & 0 & 0 & 1 & 0 \end{bmatrix} \quad (9.2.13)$$

```
> J := Transformation(VC, VC, J0) : Jtensor := convert(J0, DGtensor, [ ["con_bas",
"cov_bas"], [ ]]) :
```

```
> ω := convert(ContractIndices(Jtensor, g, [[1, 1]]), DGform);
ω := f1 ∧ f2 + f3 ∧ f4 + b f5 ∧ f6 (9.2.14)
```

```
> ω1 := Pullback(J, ExteriorDerivative(ω));
ω1 := 2 β f1 ∧ f2 ∧ f5 - 2 u2 f1 ∧ f4 ∧ f5 + 2 u2 f2 ∧ f3 ∧ f5 + 2 β f3 ∧ f4 ∧ f5 (9.2.15)
```

```
> ω2 := Pullback(J, ExteriorDerivative(ω1))
ω2 := (4 u2^2 - 4 β^2 - 2 β) f1 ∧ f2 ∧ f5 ∧ f6 + 4 u1 u2 f1 ∧ f3 ∧ f5 ∧ f6
- 2 u2 f1 ∧ f4 ∧ f5 ∧ f6 + 2 u2 f2 ∧ f3 ∧ f5 ∧ f6 + 4 u1 u2 f2 ∧ f4 ∧ f5 ∧ f6
+ (4 u2^2 - 4 β^2 - 2 β) f3 ∧ f4 ∧ f5 ∧ f6 (9.2.16)
```

```
> ω3 := Pullback(J, ExteriorDerivative(ω2));
ω3 := 0 f1 ∧ f2 ∧ f3 ∧ f4 ∧ f5 (9.2.17)
```

```
> NJ := TensorBrackets(Jtensor, Jtensor, "Frolicher-Nijenhuis")
NJ := -4 u2 e1 f3 f6 + 4 u2 e1 f4 f5 - 4 u2 e1 f5 f4 + 4 u2 e1 f6 f3 - 4 u2 e2 f3 f5
- 4 u2 e2 f4 f6 + 4 u2 e2 f5 f3 + 4 u2 e2 f6 f4 - 4 u2 e3 f1 f6 - 4 u2 e3 f2 f5
+ 4 u2 e3 f5 f2 + 4 u2 e3 f6 f1 + 4 u2 e4 f1 f5 - 4 u2 e4 f2 f6 - 4 u2 e4 f5 f1
+ 4 u2 e4 f6 f2 (9.2.18)
```

```
> KaehlerEq := DGinfo(ExteriorDerivative(ω), "CoefficientSet");
KaehlerEq := {-2 u2, 2 u2, 2 β} (9.2.19)
```

```
> use RealDomain in sols := solve( {op(DGinfo(ω1, "CoefficientSet")), op(DGinfo(NJ,
"CoefficientSet"))} ) end use
sols := {u2 = 0, β = 0} (9.2.20)
```

This is a case of the Kahler structure

```
> use RealDomain in sols := solve( {op(DGinfo(ω2, "CoefficientSet")), op(DGinfo(NJ,
"CoefficientSet"))} ) end use
sols := {u1 = u1, u2 = 0, β = 0}, {u1 = u1, u2 = 0, β = -1/2} (9.2.21)
```

The first case is Kahler, the second is SKT

```
>
```

> restart : with(DifferentialGeometry) : with(LieAlgebras) : with(Tensor) : with(Tools) :  
with(LinearAlgebra) :

$p = \frac{1}{2} \cdot \left( \left( l + \frac{\epsilon}{l} \right) \cdot i + \left( \frac{\epsilon}{l} - l \right) \cdot j \right), \epsilon = -p^2 = \pm 1$ . The quaternion notations for the isotropy are:  
 $u=i, k=j, m=k$ .

> StructureEquations := [ [LAI, LAj] = 2 \* LAK, [LAI, LAK] = -2 \* LAj, [LAj, LAK] = -2 \* LAi,  
[LAI, ee] = ii, [LAI, ii] = -ee, [LAI, jj] = kk, [LAI, kk] = -jj, [LAj, ee] = jj, [LAj, ii] = -kk,  
[LAj, jj] = ee, [LAj, kk] = -ii, [LAK, ee] = kk, [LAK, ii] = jj, [LAK, jj] = ii, [LAK, kk] = ee,  
[ee, ii] = (epsilon/l + l) \* e - LAi, [ee, jj] = (-epsilon/l + l) \* e - LAj, [ee, kk] = -LAK, [ii, jj] =  
-LAK, [ii, kk] = (-epsilon/l + l) \* e + LAj, [jj, kk] = (epsilon/l + l) \* e + LAi, [ee, e] = 3 \* epsilon \* ( (1  
/ 4 \* (epsilon/l + l) ) \* ii + (1/4 \* (epsilon/l - l) ) \* jj ), [ii, e] = 3 \* epsilon \* ( -(1/4 \* (epsilon/l + l) ) \* ee  
+ (1/4 \* (epsilon/l - l) ) \* kk ), [jj, e] = 3 \* epsilon \* ( -(1/4 \* (epsilon/l + l) ) \* kk + (1/4 \* (epsilon/l  
- l) ) \* ee ), [kk, e] = 3 \* epsilon \* ( (1/4 \* (epsilon/l + l) ) \* jj + (1/4 \* (epsilon/l - l) ) \* ii ), [LAI,  
LAj, LAK, ee, ii, jj, kk, e, ie] :

L := LieAlgebraData(StructureEquations, VC) :

> DGsetup(L, [e], [f]) : factor(Query({epsilon, l}, "Jacobi")[2])  
 $\{0, -3(\epsilon - 1)(\epsilon + 1), 3(\epsilon - 1)(\epsilon + 1)\}$  (10.1)

> g := evalDG(temp \* (-f1 &t f1 + f2 &t f2 + f3 &t f3) + ((f4 &t f4 + f5 &t f5) - (f6 &t f6  
+ f7 &t f7)) + b \* (f8 &t f8 + f9 &t f9)) :

> J0 := Matrix([ [0, 0, 0, 0, 0, 0, 0, 0, 0], [0, 0, 0, 0, 0, 0, 0, 0, 0], [0, 0, 0, 0, 0, 0, 0, 0, 0], [0,  
0, 0, 0, -((1 + r^2 + t^2)/(2 t)), -((1 + r^2 - t^2)/(2 t)), -r, 0, 0], [0, 0, 0, (1 + r  
^2 + t^2)/(2 t), 0, r, -((1 + r^2 - t^2)/(2 t)), 0, 0], [0, 0, 0, -((1 + r^2 - t^2)/(2  
t)), r, 0, (1 + r^2 + t^2)/(2 t), 0, 0], [0, 0, 0, -r, -((1 + r^2 - t^2)/(2 t)), -((1 + r  
^2 + t^2)/(2 t)), 0, 0, 0], [0, 0, 0, 0, 0, 0, 0, 0, -1], [0, 0, 0, 0, 0, 0, 0, 1, 0]])

J0 := (10.2)

$$\begin{bmatrix} [0, 0, 0, 0, 0, 0, 0, 0, 0], \\ [0, 0, 0, 0, 0, 0, 0, 0, 0], \\ [0, 0, 0, 0, 0, 0, 0, 0, 0], \\ [0, 0, 0, 0, -\frac{1}{2} \frac{r^2 + t^2 + 1}{t}, -\frac{1}{2} \frac{r^2 - t^2 + 1}{t}, -r, 0, 0], \\ [0, 0, 0, \frac{1}{2} \frac{r^2 + t^2 + 1}{t}, 0, r, -\frac{1}{2} \frac{r^2 - t^2 + 1}{t}, 0, 0], \\ [0, 0, 0, -\frac{1}{2} \frac{r^2 - t^2 + 1}{t}, r, 0, \frac{1}{2} \frac{r^2 + t^2 + 1}{t}, 0, 0], \\ [0, 0, 0, -r, -\frac{1}{2} \frac{r^2 - t^2 + 1}{t}, -\frac{1}{2} \frac{r^2 + t^2 + 1}{t}, 0, 0, 0], \\ [0, 0, 0, 0, 0, 0, 0, 0, -1], \\ [0, 0, 0, 0, 0, 0, 0, 1, 0] \end{bmatrix}$$

>  $J := \text{convert}(J0, \text{DGtensor}, [[\text{"con\_bas"}, \text{"cov\_bas"}], [ ])] : Jt := \text{Transformation}(\text{VC}, \text{VC}, J0) :$

>  $w := \text{convert}(\text{ContractIndices}(J, g, [[1, 1]]), \text{DGform}) ;$

$$w := \frac{r^2 + t^2 + 1}{2t} f4 \wedge f5 + \frac{r^2 - t^2 + 1}{2t} f4 \wedge f6 + r f4 \wedge f7 - r f5 \wedge f6 \\ + \frac{r^2 - t^2 + 1}{2t} f5 \wedge f7 + \frac{r^2 + t^2 + 1}{2t} f6 \wedge f7 + b f8 \wedge f9 \quad (10.3)$$

>  $w1 := \text{Pullback}(Jt, \text{ExteriorDerivative}(w))$

$$w1 := - \frac{b (l^2 r^2 t^2 + l^2 t^4 + r^4 \epsilon + r^2 t^2 \epsilon + 2 r^2 \epsilon + \epsilon)}{l t^2} f4 \wedge f5 \wedge f8 \\ - \frac{3 \epsilon (l^2 - \epsilon) r}{2 l} f4 \wedge f5 \wedge f9 \\ - \frac{b (l^2 r^2 t^2 - l^2 t^4 + r^4 \epsilon - r^2 t^2 \epsilon + 2 r^2 \epsilon + \epsilon)}{l t^2} f4 \wedge f6 \wedge f8 \\ - \frac{3 \epsilon (l^2 + \epsilon) r}{2 l} f4 \wedge f6 \wedge f9 - \frac{2 b r (l^2 t^2 + r^2 \epsilon + \epsilon)}{l t} f4 \wedge f7 \wedge f8 \\ - \frac{3 \epsilon (l^2 t^2 - r^2 \epsilon - \epsilon)}{2 l t} f4 \wedge f7 \wedge f9 + \frac{2 b r (l^2 t^2 + r^2 \epsilon + \epsilon)}{l t} f5 \wedge f6 \wedge f8 \\ + \frac{3 \epsilon (l^2 t^2 - r^2 \epsilon - \epsilon)}{2 l t} f5 \wedge f6 \wedge f9 \\ - \frac{b (l^2 r^2 t^2 - l^2 t^4 + r^4 \epsilon - r^2 t^2 \epsilon + 2 r^2 \epsilon + \epsilon)}{l t^2} f5 \wedge f7 \wedge f8 \\ - \frac{3 \epsilon (l^2 + \epsilon) r}{2 l} f5 \wedge f7 \wedge f9 \\ - \frac{b (l^2 r^2 t^2 + l^2 t^4 + r^4 \epsilon + r^2 t^2 \epsilon + 2 r^2 \epsilon + \epsilon)}{l t^2} f6 \wedge f7 \wedge f8 \\ - \frac{3 \epsilon (l^2 - \epsilon) r}{2 l} f6 \wedge f7 \wedge f9 \quad (10.4)$$

>  $w2 := \text{Pullback}(Jt, \text{ExteriorDerivative}(w1))$

$$w2 := \frac{4 b (l^4 t^4 + 2 \epsilon r^2 l^2 t^2 + r^4 \epsilon^2 + 2 r^2 \epsilon^2 + \epsilon^2)}{l^2 t^2} f4 \wedge f5 \wedge f6 \wedge f7 \\ + \frac{1}{4 l^2 t^3} (9 \epsilon^2 (l^4 r^2 t^4 + l^4 t^6 + 2 l^2 r^4 t^2 \epsilon + 2 l^2 r^2 t^4 \epsilon + r^6 \epsilon^2 + r^4 t^2 \epsilon^2 + \epsilon r^2 l^2 t^2 \\ - l^2 t^4 \epsilon + 3 r^4 \epsilon^2 + r^2 t^2 \epsilon^2 - l^2 t^2 \epsilon + 3 r^2 \epsilon^2 + \epsilon^2)) f4 \wedge f5 \wedge f8 \wedge f9 \\ + \frac{1}{4 l^2 t^3} (9 \epsilon^2 (l^4 r^2 t^4 - l^4 t^6 + 2 l^2 r^4 t^2 \epsilon - 2 l^2 r^2 t^4 \epsilon + r^6 \epsilon^2 - r^4 t^2 \epsilon^2 + \epsilon r^2 l^2 t^2 \\ + l^2 t^4 \epsilon + 3 r^4 \epsilon^2 - r^2 t^2 \epsilon^2 - l^2 t^2 \epsilon + 3 r^2 \epsilon^2 + \epsilon^2)) f4 \wedge f6 \wedge f8 \wedge f9 \quad (10.5)$$

$$\begin{aligned}
& + \frac{9 \varepsilon^2 r (l^4 t^4 + 2 \varepsilon r^2 l^2 t^2 + r^4 \varepsilon^2 + 2 r^2 \varepsilon^2 + \varepsilon^2)}{2 l^2 t^2} f4 \wedge f7 \wedge f8 \wedge f9 \\
& - \frac{9 \varepsilon^2 r (l^4 t^4 + 2 \varepsilon r^2 l^2 t^2 + r^4 \varepsilon^2 + 2 r^2 \varepsilon^2 + \varepsilon^2)}{2 l^2 t^2} f5 \wedge f6 \wedge f8 \wedge f9 \\
& + \frac{1}{4 l^2 t^3} (9 \varepsilon^2 (l^4 r^2 t^4 - l^4 t^6 + 2 l^2 r^4 t^2 \varepsilon - 2 l^2 r^2 t^4 \varepsilon + r^6 \varepsilon^2 - r^4 t^2 \varepsilon^2 + \varepsilon r^2 l^2 t^2 \\
& + l^2 t^4 \varepsilon + 3 r^4 \varepsilon^2 - r^2 t^2 \varepsilon^2 - l^2 t^2 \varepsilon + 3 r^2 \varepsilon^2 + \varepsilon^2)) f5 \wedge f7 \wedge f8 \wedge f9 \\
& + \frac{1}{4 l^2 t^3} (9 \varepsilon^2 (l^4 r^2 t^4 + l^4 t^6 + 2 l^2 r^4 t^2 \varepsilon + 2 l^2 r^2 t^4 \varepsilon + r^6 \varepsilon^2 + r^4 t^2 \varepsilon^2 + \varepsilon r^2 l^2 t^2 \\
& - l^2 t^4 \varepsilon + 3 r^4 \varepsilon^2 + r^2 t^2 \varepsilon^2 - l^2 t^2 \varepsilon + 3 r^2 \varepsilon^2 + \varepsilon^2)) f6 \wedge f7 \wedge f8 \wedge f9
\end{aligned}$$

> w3 := Pullback(Jt, ExteriorDerivative(w2))

$$\begin{aligned}
w3 := & -\frac{1}{l^3 t^3} (9 \varepsilon^2 (l^6 t^6 + 3 l^4 r^2 t^4 \varepsilon + 3 l^2 r^4 t^2 \varepsilon^2 - l^4 t^4 \varepsilon + r^6 \varepsilon^3 + 2 l^2 r^2 t^2 \varepsilon^2 + 3 r^4 \varepsilon^3 \\
& - l^2 t^2 \varepsilon^2 + 3 \varepsilon^3 r^2 + \varepsilon^3)) f4 \wedge f5 \wedge f6 \wedge f7 \wedge f8
\end{aligned} \quad (10.6)$$

> w4 := Pullback(Jt, ExteriorDerivative(w3))

$$w4 := 0 f1 \wedge f2 \wedge f3 \wedge f4 \wedge f5 \wedge f6 \quad (10.7)$$

> solve({op(DGinfo(w2, "CoefficientSet")), b ≠ 0})

$$\begin{aligned}
> \text{solve}(\text{subs}(\{l=1, \varepsilon=1\}, l^6 t^6 + 3 l^4 r^2 t^4 \varepsilon + 3 l^2 r^4 t^2 \varepsilon^2 - l^4 t^4 \varepsilon + r^6 \varepsilon^3 + 2 l^2 r^2 t^2 \varepsilon^2 + 3 r^4 \varepsilon^3 \\
- l^2 t^2 \varepsilon^2 + 3 \varepsilon^3 r^2 + \varepsilon^3), t) \\
\sqrt{-r^2-1}, -\sqrt{-r^2-1}, \sqrt{-r^2+1+2Ir}, -\sqrt{-r^2+1+2Ir}, \sqrt{-r^2+1-2Ir}, \\
-\sqrt{-r^2+1-2Ir}
\end{aligned} \quad (10.8)$$

$$\begin{aligned}
> \text{factor}(\text{subs}(\{r=0, l=1, \varepsilon=1\}, l^6 t^6 + 3 l^4 r^2 t^4 \varepsilon + 3 l^2 r^4 t^2 \varepsilon^2 - l^4 t^4 \varepsilon + r^6 \varepsilon^3 + 2 l^2 r^2 t^2 \varepsilon^2 \\
+ 3 r^4 \varepsilon^3 - l^2 t^2 \varepsilon^2 + 3 \varepsilon^3 r^2 + \varepsilon^3)) \\
(t^2 + 1)(t - 1)^2(t + 1)^2
\end{aligned} \quad (10.9)$$

> use RealDomain in solve({op(DGinfo(w3, "CoefficientSet")), b ≠ 0, ε = 1, l = 1, r ≠ 0})  
end use

$$\{b=b, l=1, r=\text{RootOf}(\_Z^2 + t^2 + 1), t=t, \varepsilon=1\} \quad (10.10)$$

> use RealDomain in solve({op(DGinfo(w3, "CoefficientSet")), b ≠ 0, ε = 1, l = 1, r = 0})  
end use

$$\{b=b, l=1, r=0, t=1, \varepsilon=1\}, \{b=b, l=1, r=0, t=-1, \varepsilon=1\} \quad (10.11)$$

This is q=±i and 3-SKT

$$\begin{aligned}
> \text{solve}(\text{subs}(\{l=-1, \varepsilon=-1\}, l^6 t^6 + 3 l^4 r^2 t^4 \varepsilon + 3 l^2 r^4 t^2 \varepsilon^2 - l^4 t^4 \varepsilon + r^6 \varepsilon^3 + 2 l^2 r^2 t^2 \varepsilon^2 \\
+ 3 r^4 \varepsilon^3 - l^2 t^2 \varepsilon^2 + 3 \varepsilon^3 r^2 + \varepsilon^3), t) \\
\sqrt{r^2+1}, -\sqrt{r^2+1}, \sqrt{2Ir+r^2-1}, -\sqrt{2Ir+r^2-1}, \sqrt{-2Ir+r^2-1}, \\
-\sqrt{-2Ir+r^2-1}
\end{aligned} \quad (10.12)$$

$$\begin{aligned} &> \text{factor}\left(\text{subs}\left(\{r=0, l=-1, \varepsilon=-1\}, t^6 t^6 + 3 t^4 r^2 t^4 \varepsilon + 3 t^2 r^4 t^2 \varepsilon^2 - t^4 t^4 \varepsilon + r^6 \varepsilon^3 + 2 t^2 r^2 t^2 \varepsilon^2 \right. \right. \\ &\quad \left. \left. + 3 r^4 \varepsilon^3 - t^2 t^2 \varepsilon^2 + 3 \varepsilon^3 r^2 + \varepsilon^3\right)\right) \\ &\quad (t-1)(t+1)(t^2+1)^2 \end{aligned} \quad (10.13)$$

$$\begin{aligned} &> \text{use RealDomain in solve}\left(\{op(DGinfo(w3, "CoefficientSet")), b \neq 0, \varepsilon=-1, l=-1, r \neq 0\}\right) \\ &\quad \text{end use} \\ &\quad \{b=b, l=-1, r=\text{RootOf}(\_Z^2 - t^2 + 1), t=t, \varepsilon=-1\} \end{aligned} \quad (10.14)$$

$$\begin{aligned} &> \text{use RealDomain in solve}\left(\{op(DGinfo(w3, "CoefficientSet")), b \neq 0, \varepsilon=-1, l=-1, r=0\}\right) \\ &\quad \text{end use} \\ &\quad \{b=b, l=-1, r=0, t=1, \varepsilon=-1\}, \{b=b, l=-1, r=0, t=-1, \varepsilon=-1\} \end{aligned} \quad (10.15)$$

This is a circle of 3-SKT solutions

>

Thus no real solutions (also for the Kahler condition) for SKT, but there are 3-SKT solutions

## A4.2

$$\begin{aligned} &> \text{restart : with(DifferentialGeometry) : with(LieAlgebras) : with(Tensor) : with(Tools) :} \\ &\quad \text{with(LinearAlgebra) :} \\ &> \text{StructureEquations := } [[i, j]=k, [i, k]=-j, [j, k]=-i, [i, j2]=k2, [i, k2]=-j2, [j, k2]=- \\ &\quad -i2, [i2, j]=k2, [i2, k]=-j2, [j2, k]=-i2, [i2, j2]=-k, [i2, k2]=j, [j2, k2]=i, [i, j, k, \\ &\quad i2, j2, k2] : \\ &\quad L := \text{LieAlgebraData(StructureEquations, Dsu) :} \\ &> \text{DGsetup(L, [e], [f]) :} \\ &> w := \text{evalDG}(-f1 \&w f4 + f2 \&w f5 + f3 \&w f6) : \\ &> J0 := \text{Matrix}\left(\left[\left[\begin{matrix} r, 0, 0, -\frac{(1+r^2)}{t}, 0, 0 \end{matrix}\right], \left[\begin{matrix} 0, r, 0, 0, -\frac{(1+r^2)}{t}, 0 \end{matrix}\right], \left[\begin{matrix} 0, 0, r, 0, 0, -\frac{(1+r^2)}{t} \end{matrix}\right], \right. \right. \\ &\quad \left. \left. \left[\begin{matrix} t, 0, 0, -r, 0, 0 \end{matrix}\right], \left[\begin{matrix} 0, t, 0, 0, -r, 0 \end{matrix}\right], \left[\begin{matrix} 0, 0, t, 0, 0, -r \end{matrix}\right] \right] \right) : \\ &> J := \text{convert}(J0, DGtensor, [[ "con_bas", "cov_bas"], [ ]]); \\ &\quad J := r e1 f1 - \frac{r^2+1}{t} e1 f4 + r e2 f2 - \frac{r^2+1}{t} e2 f5 + r e3 f3 - \frac{r^2+1}{t} e3 f6 + t e4 f1 \\ &\quad - r e4 f4 + t e5 f2 - r e5 f5 + t e6 f3 - r e6 f6 \end{aligned} \quad (11.1)$$

$$\begin{aligned} &> Jt := \text{Transformation}(Dsu, Dsu, J0); \\ &\quad Jt := \left[ [e1, r e1 + t e4], [e2, r e2 + t e5], [e3, r e3 + t e6], \left[ e4, -\frac{r^2+1}{t} e1 - r e4 \right], \left[ e5, \right. \right. \\ &\quad \left. \left. -\frac{r^2+1}{t} e2 - r e5 \right], \left[ e6, -\frac{r^2+1}{t} e3 - r e6 \right] \right] \end{aligned} \quad (11.2)$$

$$\begin{aligned} &> w1 := \text{Pullback}(Jt, \text{ExteriorDerivative}(w)); \\ &\quad w1 := (3 r^2 t + 3 t^3) f1 \wedge f2 \wedge f3 - (3 r^3 + 3 t^2 r + 2 r) f1 \wedge f2 \wedge f6 + (3 r^3 + 3 t^2 r \\ &\quad + 2 r) f1 \wedge f3 \wedge f5 + \frac{3 r^4 + 3 r^2 t^2 + 4 r^2 + 1}{t} f1 \wedge f5 \wedge f6 - (3 r^3 + 3 t^2 r \\ &\quad + 2 r) f2 \wedge f3 \wedge f4 - \frac{3 r^4 + 3 r^2 t^2 + 4 r^2 + 1}{t} f2 \wedge f4 \wedge f6 \end{aligned} \quad (11.3)$$

$$+ \frac{3r^4 + 3r^2t^2 + 4r^2 + 1}{t} f_3 \wedge f_4 \wedge f_5 - \frac{3r(r^4 + r^2t^2 + 2r^2 + 1)}{t^2} f_4 \wedge f_5 \wedge f_6$$

> w2 := Pullback(Jt, ExteriorDerivative(w1))

$$w2 := \frac{3r^4 + 6r^2t^2 + 3t^4 + 4r^2 + 1}{t} f_1 \wedge f_2 \wedge f_4 \wedge f_5 \quad (11.4)$$

$$+ \frac{3r^4 + 6r^2t^2 + 3t^4 + 4r^2 + 1}{t} f_1 \wedge f_3 \wedge f_4 \wedge f_6$$

$$- \frac{3r^4 + 6r^2t^2 + 3t^4 + 4r^2 + 1}{t} f_2 \wedge f_3 \wedge f_5 \wedge f_6$$

> w3 := Pullback(Jt, ExteriorDerivative(w2))

$$w3 := 0 f_1 \wedge f_2 \wedge f_3 \wedge f_4 \wedge f_5 \quad (11.5)$$

> w4 := Pullback(Jt, ExteriorDerivative(w3))

$$w4 := 0 f_1 \wedge f_2 \wedge f_3 \wedge f_4 \wedge f_5 \wedge f_6 \quad (11.6)$$

> DGinfo(w2, "CoefficientSet");

$$\left\{ \frac{3r^4 + 6r^2t^2 + 3t^4 + 4r^2 + 1}{t}, -\frac{3r^4 + 6r^2t^2 + 3t^4 + 4r^2 + 1}{t} \right\} \quad (11.7)$$

No real solutions (also for the Kahler condition)
