# Supplementary material for: Homogeneous almost complex structures in dimension 6 with semi-simple isotropy
Source: arXiv:1401.8187 ancillary file (2014-02-12)
Supplement: Supplementary file 4 [file SNPK.pdf]

# Strictly Nearly Pseudo-Kähler

We test the relation  $\nabla \omega \in \Lambda^3 m^*$   
on our homogeneous almost pseudo-Hermitian structures with nondegenerate Nijenhuis tensor  $N_J$ .

We focus on indefinite signature Hermitian structures, since the definite case is already known  
. We consider only those cases, where nondegenerate  $NJ$  occurs

## A1.1

```
> restart : with(DifferentialGeometry) : with(LieAlgebras) : with(Tensor) : with(Tools) :  
with(LinearAlgebra) :
```

$$\begin{aligned} > \text{StructureEquations} := \left[ [ee, ii] = \alpha * e, [jj, kk] = -\alpha * e, [ee, ie] = \frac{\epsilon}{2} * ee + r * ii, [ii, ie] = \frac{\epsilon}{2} \right. \\ &\quad * ii - r * ee, [jj, ie] = \frac{\epsilon}{2} * jj - r * kk, [kk, ie] = \frac{\epsilon}{2} * kk + r * jj, [e, ie] = \epsilon * e \left. \right], [ee, ii, jj, \\ &\quad kk, e, ie] : L := \text{LieAlgebraData}(\text{StructureEquations}, VC); \\ L := \left[ [e1, e2] = \alpha e5, [e1, e6] = \frac{1}{2} \epsilon e1 + r e2, [e2, e6] = -r e1 + \frac{1}{2} \epsilon e2, [e3, e4] = \right. & (1.1) \\ &\quad \left. -\alpha e5, [e3, e6] = \frac{1}{2} \epsilon e3 - r e4, [e4, e6] = r e3 + \frac{1}{2} \epsilon e4, [e5, e6] = \epsilon e5 \right] \end{aligned}$$

```
> DGsetup(L, [e], [f]) :
```

$$\begin{aligned} > g := \text{evalDG}(t \cdot (f1 \&t f1 + f2 \&t f2 + f3 \&t f3 + f4 \&t f4) + (f5 \&t f5 + f6 \&t f6)); \\ &\quad g := t f1 f1 + t f2 f2 + t f3 f3 + t f4 f4 + f5 f5 + f6 f6 & (1.2) \end{aligned}$$

$$\begin{aligned} > EC := \text{evalDG}(\text{RaiseLowerIndices}(g, \text{EinsteinTensor}(g), [1, 2]) + \Lambda \cdot g) \\ EC := (\Lambda t + 4 \epsilon^2 t) f1 f1 + (\Lambda t + 4 \epsilon^2 t) f2 f2 + (\Lambda t + 4 \epsilon^2 t) f3 f3 + (\Lambda t + 4 \epsilon^2 t) f4 f4 & (1.3) \\ + \frac{1}{2} \frac{(2 \Lambda t^2 + 5 \epsilon^2 t^2 + 3 \alpha^2) f5 f5}{t^2} + \frac{1}{2} \frac{(2 \Lambda t^2 + 7 \epsilon^2 t^2 + \alpha^2) f6 f6}{t^2} \end{aligned}$$

$$\begin{aligned} > \text{solve}(\text{DGinfo}(EC, \text{"CoefficientSet"})) \\ \{\Lambda = -4 \epsilon^2, \alpha = t \epsilon, \epsilon = \epsilon, t = t\}, \{\Lambda = -4 \epsilon^2, \alpha = -t \epsilon, \epsilon = \epsilon, t = t\} & (1.4) \end{aligned}$$

$$\begin{aligned} > J0 := \text{Matrix}([ [0, -\cos(a) \sin(b), -\sin(a) \sin(b), -\cos(b), 0, 0], [\cos(a) \sin(b), 0, \\ \cos(b), -\sin(a) \sin(b), 0, 0], [\sin(a) \sin(b), -\cos(b), 0, \cos(a) \sin(b), 0, 0], \\ \cos(a) \sin(b), 0, 0], [\cos(b), \sin(a) \sin(b), -\cos(a) \sin(b), 0, 0, 0], [0, 0, 0, 0, 0, -1], & \\ [0, 0, 0, 0, 1, 0]]); \end{aligned}$$

$$J0 := \begin{bmatrix} 0 & -\cos(a) \sin(b) & -\sin(a) \sin(b) & -\cos(b) & 0 & 0 \\ \cos(a) \sin(b) & 0 & \cos(b) & -\sin(a) \sin(b) & 0 & 0 \\ \sin(a) \sin(b) & -\cos(b) & 0 & \cos(a) \sin(b) & 0 & 0 \\ \cos(b) & \sin(a) \sin(b) & -\cos(a) \sin(b) & 0 & 0 & 0 \\ 0 & 0 & 0 & 0 & 0 & -1 \\ 0 & 0 & 0 & 0 & 1 & 0 \end{bmatrix} \quad (1.5)$$

```

> J := convert(J0, DGtensor, [ ["con_bas", "cov_bas"], [ ] ] ) :
> NJ := TensorBrackets(J, J, "Frolicher-Nijenhuis") :
> solve(DGinfo(NJ, "CoefficientSet")) ;

$$\{a = a, \alpha = 0, b = b, r = 0\}, \left\{a = 0, \alpha = \alpha, b = \frac{1}{2} \pi, r = r\right\} \quad (1.6)$$


```

```

> w := ContractIndices(J, g, [ [1, 1] ] );
w := cos(a) sin(b) t f1 f2 + sin(a) sin(b) t f1 f3 + cos(b) t f1 f4 - cos(a) sin(b) t f2 f1
- cos(b) t f2 f3 + sin(a) sin(b) t f2 f4 - sin(a) sin(b) t f3 f1 + cos(b) t f3 f2
- cos(a) sin(b) t f3 f4 - cos(b) t f4 f1 - sin(a) sin(b) t f4 f2 + cos(a) sin(b) t f4 f3
+ f5 f6 - f6 f5

```

```

> nabla := Christoffel(g) :
> NablaOmega := DGsimplify(CovariantDerivative(w, nabla)) :
> SkewNablaOmega := SymmetrizeIndices(NablaOmega, [1, 2, 3], "SkewSymmetric") :
> slv := solve( { op(DGinfo(evalDG(NablaOmega - SkewNablaOmega), "CoefficientSet")), t
≠ 0, r2 + α2 ≠ 0 } );
slv := { a = 0, α = t ε, b = 1/2 π, ε = ε, r = r, t = t }, { a = 0, α = -t ε, b = -1/2 π, ε = ε, r = r, t
= t }, { a = π, α = -t ε, b = 1/2 π, ε = ε, r = r, t = t }, { a = π, α = t ε, b = -1/2 π, ε = ε, r = r, t
= t }

```

```

> for i to nops( {slv} ) do print(DGsimplify(subs(slv[i], NJ)) ) od
0 e1 f1 f1
0 e1 f1 f1
0 e1 f1 f1
0 e1 f1 f1

```

Thus these solutions all imply NJ=0 and so must be discarded.

## A1.4

```

> restart : with(DifferentialGeometry) : with(LieAlgebras) : with(Tensor) : with(Tools) :
with(LinearAlgebra) :
> StructureEquations := [ [LAI, LAj] = 2 * LAK, [LAI, LAK] = -2 * LAj, [LAj, LAK] = 2 * LAi,
[LAI, ee] = ii, [LAI, ii] = -ee, [LAI, jj] = kk, [LAI, kk] = -jj, [LAj, ee] = jj, [LAj, ii] =
-kk, [LAj, jj] = -ee, [LAj, kk] = ii, [LAK, ee] = kk, [LAK, ii] = jj, [LAK, jj] = -ii, [LAK,
kk] = -ee, [ee, ii] = -e + ε * LAi, [ee, jj] = ε * LAj, [ee, kk] = ε * LAK, [ii, jj] = ε * LAK,
[ii, kk] = -ε * LAj, [jj, kk] = e + ε * LAi, [ee, e] = 3 ε * ii, [ii, e] = -3 ε * ee, [jj, e] = -3 ε
* kk, [kk, e] = 3 ε * jj ], [LAI, LAj, LAK, ee, ii, jj, kk, e, ie] :
L := LieAlgebraData(StructureEquations, VC);
L := [ [e1, e2] = 2 e3, [e1, e3] = -2 e2, [e1, e4] = e5, [e1, e5] = -e4, [e1, e6] = e7, [e1, e7]
= -e6, [e2, e3] = 2 e1, [e2, e4] = e6, [e2, e5] = -e7, [e2, e6] = -e4, [e2, e7] = e5, [e3,
e4] = e7, [e3, e5] = e6, [e3, e6] = -e5, [e3, e7] = -e4, [e4, e5] = e1 ε - e8, [e4, e6]

```

$$= \varepsilon e_2, [e_4, e_7] = \varepsilon e_3, [e_4, e_8] = 3 \varepsilon e_5, [e_5, e_6] = \varepsilon e_3, [e_5, e_7] = -\varepsilon e_2, [e_5, e_8] = -3 \varepsilon e_4, [e_6, e_7] = e_1 \varepsilon + e_8, [e_6, e_8] = -3 \varepsilon e_7, [e_7, e_8] = 3 \varepsilon e_6]$$

> DGsetup(L, [e], [f]) :

> Query("Jacobi");

true

(2.2)

> g := evalDG(temp·(f1 &t f1 + f2 &t f2 + f3 &t f3) + r·(f4 &t f4 + f5 &t f5 + f6 &t f6 + f7 &t f7) + t·(f8 &t f8 + f9 &t f9));

g := temp f1 f1 + temp f2 f2 + temp f3 f3 + r f4 f4 + r f5 f5 + r f6 f6 + r f7 f7 + t f8 f8 + t f9 f9 (2.3)

> J0 := Matrix([ [0, 0, 0, 0, 0, 0, 0, 0, 0], [0, 0, 0, 0, 0, 0, 0, 0, 0], [0, 0, 0, 0, 0, 0, 0, 0, 0], [0, 0, 0, 0, -cos(a) sin(b), -sin(a) sin(b), -cos(b), 0, 0], [0, 0, 0, cos(a) sin(b), 0, cos(b), -sin(a) sin(b), 0, 0], [0, 0, 0, sin(a) sin(b), -cos(b), 0, cos(a) sin(b), 0, 0], [0, 0, 0, cos(b), sin(a) sin(b), -cos(a) sin(b), 0, 0, 0], [0, 0, 0, 0, 0, 0, 0, 0, -1], [0, 0, 0, 0, 0, 0, 0, 1, 0]]);

$$J0 := \begin{bmatrix} 0 & 0 & 0 & 0 & 0 & 0 & 0 & 0 & 0 \\ 0 & 0 & 0 & 0 & 0 & 0 & 0 & 0 & 0 \\ 0 & 0 & 0 & 0 & 0 & 0 & 0 & 0 & 0 \\ 0 & 0 & 0 & 0 & -\cos(a) \sin(b) & -\sin(a) \sin(b) & -\cos(b) & 0 & 0 \\ 0 & 0 & 0 & \cos(a) \sin(b) & 0 & \cos(b) & -\sin(a) \sin(b) & 0 & 0 \\ 0 & 0 & 0 & \sin(a) \sin(b) & -\cos(b) & 0 & \cos(a) \sin(b) & 0 & 0 \\ 0 & 0 & 0 & \cos(b) & \sin(a) \sin(b) & -\cos(a) \sin(b) & 0 & 0 & 0 \\ 0 & 0 & 0 & 0 & 0 & 0 & 0 & 0 & -1 \\ 0 & 0 & 0 & 0 & 0 & 0 & 0 & 1 & 0 \end{bmatrix} \quad (2.4)$$

> J := convert(J0, DGtensor, [[ "con\_bas", "cov\_bas"], [ ]]) :

> NJ := TensorBridges(J, J, "Frolicher-Nijenhuis") :

> w := ContractIndices(J, g, [[1, 1]]);

w := cos(a) sin(b) rf4 f5 + sin(a) sin(b) rf4 f6 + cos(b) rf4 f7 - cos(a) sin(b) rf5 f4 - cos(b) rf5 f6 + sin(a) sin(b) rf5 f7 - sin(a) sin(b) rf6 f4 + cos(b) rf6 f5 - cos(a) sin(b) rf6 f7 - cos(b) rf7 f4 - sin(a) sin(b) rf7 f5 + cos(a) sin(b) rf7 f6 + t f8 f9 - t f9 f8 (2.5)

> nabla := Christoffel(g) :

> NablaOmega := DGsimplify(subs({temp=0}, CovariantDerivative(w, nabla))) :

> SkewNablaOmega := SymmetrizeIndices(NablaOmega, [1, 2, 3], "SkewSymmetric") :

> solve({op(DGinfo(evalDG(NablaOmega-SkewNablaOmega), "CoefficientSet")), t ≠ 0});

No solutions

### A3.1

> restart : with(DifferentialGeometry) : with(LieAlgebras) : with(Tensor) : with(Tools) :  
with(LinearAlgebra) :

We take  $p=p_1 \cdot i + p_2 \cdot j$  (always possible by an endomorphism)

> StructureEquations :=  $\left[ [ee, ii] = p_1 \cdot e, [ee, jj] = -p_2 \cdot e, [ii, kk] = -p_2 \cdot e, [jj, kk] = p_1 \cdot e, \right.$

$$\begin{aligned}
[ee, ie] &= \frac{\varepsilon}{2} \cdot ee + R \cdot p1 \cdot ii + R \cdot p2 \cdot jj, [ii, ie] = \frac{\varepsilon}{2} \cdot ii - R \cdot p1 \cdot ee + R \cdot p2 \cdot kk, [jj, ie] \\
&= \frac{\varepsilon}{2} \cdot jj - R \cdot p1 \cdot kk + R \cdot p2 \cdot ee, [kk, ie] = \frac{\varepsilon}{2} \cdot kk + R \cdot p1 \cdot jj + R \cdot p2 \cdot ii, [e, ie] = \varepsilon \cdot e \\
&[ee, ii, jj, kk, e, ie] :
\end{aligned}$$

$L := \text{LieAlgebraData}(\text{StructureEquations}, \text{VC});$

$$\begin{aligned}
L := \left[ [e1, e2] = p1 \cdot e5, [e1, e3] = -p2 \cdot e5, [e1, e6] = R \cdot p2 \cdot e3 + R \cdot p1 \cdot e2 + \frac{1}{2} \varepsilon \cdot e1, [e2, e4] = \right. \\
\left. -p2 \cdot e5, [e2, e6] = R \cdot p2 \cdot e4 + \frac{1}{2} \varepsilon \cdot e2 - R \cdot p1 \cdot e1, [e3, e4] = p1 \cdot e5, [e3, e6] = -R \cdot p1 \cdot e4 \right. \\
\left. + \frac{1}{2} \varepsilon \cdot e3 + R \cdot p2 \cdot e1, [e4, e6] = \frac{1}{2} \varepsilon \cdot e4 + R \cdot p2 \cdot e2 + R \cdot p1 \cdot e3, [e5, e6] = \varepsilon \cdot e5 \right] \quad (3.1)
\end{aligned}$$

$$\begin{aligned}
> \text{DGsetup}(L, [e], [f]) : \text{Query}(\text{"Jacobi"}); \\
&\text{true} \quad (3.2)
\end{aligned}$$

$$\begin{aligned}
> g := \text{evalDG}(b \cdot (f1 \&t f1 + f2 \&t f2 - f3 \&t f3 - f4 \&t f4) + (f5 \&t f5 + f6 \&t f6)); \\
&g := b f1 f1 + b f2 f2 - b f3 f3 - b f4 f4 + f5 f5 + f6 f6 \quad (3.3)
\end{aligned}$$

We can always normalize by an endomorphism  $q=i$  on  $V$ . This is equivalent to  $\{r=0, t=1\}$  in the general parametrization of  $J$  below

$$\begin{aligned}
> J0 := \text{subs}(\{r=0, t=1\}, \text{Matrix}([ [0, -((1 + r^2 + t^2)/(2t)), -((1 + r^2 - t^2)/(2t)), -r, 0, 0], [ ( \\
&1 + r^2 + t^2)/(2t), 0, r, -((1 + r^2 - t^2)/(2t)), 0, 0], [ -((1 + r^2 - t^2)/(2t)), r, 0, (1 + r^2 + t^2)/(2t), 0, 0], [ -r, -((1 + r^2 - t^2)/(2t)), -((1 + r^2 + t^2)/(2t)), 0, 0, 0], [0, 0, 0, 0, 0, -1], [0, 0, 0, 0, 1, 0]])); \\
&J0 := \begin{bmatrix} 0 & -1 & 0 & 0 & 0 & 0 \\ 1 & 0 & 0 & 0 & 0 & 0 \\ 0 & 0 & 0 & 1 & 0 & 0 \\ 0 & 0 & -1 & 0 & 0 & 0 \\ 0 & 0 & 0 & 0 & 0 & -1 \\ 0 & 0 & 0 & 0 & 1 & 0 \end{bmatrix} \quad (3.4)
\end{aligned}$$

$$\begin{aligned}
> J := \text{convert}(J0, \text{DGtensor}, [ ["con_bas", "cov_bas"], [ ]]); \\
> w := \text{ContractIndices}(J, g, [ [1, 1]]); \\
&w := b f1 f2 - b f2 f1 + b f3 f4 - b f4 f3 + f5 f6 - f6 f5 \quad (3.5)
\end{aligned}$$

$$\begin{aligned}
> \text{nabla} := \text{Christoffel}(g) : \\
> \text{NablaOmega} := \text{DGsimplify}(\text{subs}(\{temp=0\}, \text{CovariantDerivative}(w, \text{nabla}))) : \\
> \text{SkewNablaOmega} := \text{SymmetrizeIndices}(\text{NablaOmega}, [1, 2, 3], \text{"SkewSymmetric"}) : \\
> \text{solve}(\text{DGinfo}(\text{evalDG}(\text{NablaOmega} - \text{SkewNablaOmega}), \text{"CoefficientSet"})); \\
&\{R=R, b=b, p1=b \varepsilon, p2=0, \varepsilon=\varepsilon\} \quad (3.6)
\end{aligned}$$

$$\begin{aligned}
> NJ := \text{TensorBrackets}(J, J, \text{"Frolicher-Nijenhuis"}) : \\
> \text{DGsimplify}(\text{subs}(\{R=R, b=b, \varepsilon=\varepsilon, p1=b \varepsilon, p2=0\}, NJ)); \\
&0 e1 f1 f1 \quad (3.7)
\end{aligned}$$

Not SNPK because NJ is zero.

>

## A3.2

**r≠0**

> restart : with(DifferentialGeometry) : with(LieAlgebras) : with(Tensor) : with(Tools) :

We normalize  $\mathbf{p} = t \cdot (ii + jj)$ ,  $r = r/t$ ,  $u =$

$-\frac{\varepsilon}{2} \cdot kk + \lambda \cdot (ii + jj)$ . This we can do using the endomorphism freedom,  
and furthermore we can fix  $q = i$  by the same endom.

> StructureEquations :=  $\left[ [ee, ii] = t \cdot e, [ee, jj] = -t \cdot e, [ii, kk] = -t \cdot e, [jj, kk] = t \cdot e, [ee, e] = r \cdot (ii + jj), [ii, e] = -r \cdot (ee - kk), [jj, e] = r \cdot (ee - kk), [kk, e] = r \cdot (ii + jj), [ee, ie] = \varepsilon \cdot ee + \lambda \cdot (ii + jj) - \frac{\varepsilon}{2} \cdot kk, [ii, ie] = \varepsilon \cdot ii - \lambda \cdot (ee - kk) + \frac{\varepsilon}{2} \cdot jj, [jj, ie] = \varepsilon \cdot jj + \lambda \cdot (ee - kk) + \frac{\varepsilon}{2} \cdot ii, [kk, ie] = \varepsilon \cdot kk + \lambda \cdot (ii + jj) - \frac{\varepsilon}{2} \cdot ee, [e, ie] = \varepsilon \cdot e \right], [ee, ii, jj, kk, e, ie] : L := LieAlgebraData(StructureEquations, VC);$

$$L := \left[ [e1, e2] = t e5, [e1, e3] = -t e5, [e1, e5] = e2 r + e3 r, [e1, e6] = -\frac{1}{2} \varepsilon e4 + \varepsilon e1 \right. \quad (4.1.1) \\ \left. + \lambda e2 + \lambda e3, [e2, e4] = -t e5, [e2, e5] = -e1 r + e4 r, [e2, e6] = \lambda e4 + \frac{1}{2} \varepsilon e3 \right. \\ \left. - \lambda e1 + \varepsilon e2, [e3, e4] = t e5, [e3, e5] = e1 r - e4 r, [e3, e6] = -\lambda e4 + \varepsilon e3 \right. \\ \left. + \frac{1}{2} \varepsilon e2 + \lambda e1, [e4, e5] = e2 r + e3 r, [e4, e6] = \varepsilon e4 + \lambda e3 + \lambda e2 - \frac{1}{2} \varepsilon e1, \right. \\ \left. [e5, e6] = \varepsilon e5 \right]$$

> DGsetup(L, [e], [f]) : Query("Jacobi"); true (4.1.2)

> g := evalDG(b · (f1 &t f1 + f2 &t f2 - f3 &t f3 - f4 &t f4) + (f5 &t f5 + f6 &t f6));  
 $g := b f1 f1 + b f2 f2 - b f3 f3 - b f4 f4 + f5 f5 + f6 f6$  (4.1.3)

> J0 := Matrix([ [0, -1, 0, 0, 0, 0], [1, 0, 0, 0, 0, 0], [0, 0, 0, 1, 0, 0], [0, 0, -1, 0, 0, 0],  
[0, 0, 0, 0, 0, -1], [0, 0, 0, 0, 1, 0]])

$$J0 := \begin{bmatrix} 0 & -1 & 0 & 0 & 0 & 0 \\ 1 & 0 & 0 & 0 & 0 & 0 \\ 0 & 0 & 0 & 1 & 0 & 0 \\ 0 & 0 & -1 & 0 & 0 & 0 \\ 0 & 0 & 0 & 0 & 0 & -1 \\ 0 & 0 & 0 & 0 & 1 & 0 \end{bmatrix} \quad (4.1.4)$$

> J := Transformation(VC, VC, J0) : Jtensor := convert(J0, DGtensor, [ ["con\_bas",  
"cov\_bas"], [ ]]) : ContractIndices(Jtensor, Jtensor, [[2, 1]])  
 $-e1 f1 - e2 f2 - e3 f3 - e4 f4 - e5 f5 - e6 f6$  (4.1.5)

```

> NJ := TensorBrackets(Jtensor, Jtensor, "Frolicher-Nijenhuis") :
> ω := convert(ContractIndices(Jtensor, g, [[1, 1]]), DGform);
      ω := b f1 ∧ f2 + b f3 ∧ f4 + f5 ∧ f6

```

(4.1.6)

```

> nabla := Christoffel(g) :
> NablaOmega := DGsimplify(subs({temp=0}, CovariantDerivative(ω, nabla))) :
> SkewNablaOmega := SymmetrizeIndices(NablaOmega, [1, 2, 3], "SkewSymmetric") :
> use RealDomain in slv := solve({op(DGinfo(evalDG(NablaOmega
    - SkewNablaOmega), "CoefficientSet")), ε=0, b ≠ 0}) end use
      slv := {b=b, r=0, t=0, ε=0, λ=0}

```

(4.1.7)

```

> simplify(DGinfo(subs(slv, NJ), "CoefficientSet"));
      {0}

```

(4.1.8)

This is not SNPK structure because NJ=0

```

> slv := solve({op(DGinfo(evalDG(NablaOmega-SkewNablaOmega),
    "CoefficientSet")), ε=1, b ≠ 0});
      slv := {b=b, r=-3/2, t=2 b, ε=1, λ=0}

```

(4.1.9)

```

>
> simplify(subs(slv, NJ))
-8 b e5 f3 f1 - 8 b e5 f4 f2 + 8 b e5 f1 f3 + 0 e4 f6 f2 - 8 e4 f6 f1 - 8 e4 f5 f2
+ 0 e4 f5 f1 + 0 e4 f2 f6 + 8 e4 f2 f5 + 8 e4 f1 f6 + 0 e4 f1 f5 + 8 e3 f6 f2
+ 0 e3 f6 f1 + 0 e3 f5 f2 - 8 e3 f5 f1 - 8 e3 f2 f6 + 0 e3 f2 f5 + 0 e3 f1 f6
+ 8 e3 f1 f5 + 0 e2 f6 f4 + 8 e2 f6 f3 - 8 e2 f5 f4 + 0 e2 f5 f3 + 0 e2 f4 f6
+ 8 e2 f4 f5 - 8 e2 f3 f6 + 0 e2 f3 f5 - 8 e1 f6 f4 + 0 e1 f6 f3 + 8 b e5 f2 f4
+ 0 e1 f5 f4 - 8 e1 f5 f3 + 8 e1 f4 f6 + 0 e1 f4 f5 + 0 e1 f3 f6 + 8 e1 f3 f5
- 8 b e6 f4 f1 + 8 b e6 f3 f2 - 8 b e6 f2 f3 + 8 b e6 f1 f4

```

(4.1.10)

```

> NT := (i, j) → ContractIndices(e || i &t e || j, DGsimplify(subs(slv[2], NJ)), [[1, 2], [2,
    3]]):
S := { } : for i to 5 do for j from i + 1 to 6 do S := {op(S), NT(i, j)} : od: od: S
{-4 t e6, 0 e1, 4 t e5, 4 t e6, (2 ε + 6) e1 - 4 λ e2, (2 ε + 6) e3 + 4 λ e4, 4 λ e1 + (2 ε
+ 6) e2, -(2 ε + 6) e3 - 4 λ e4, -4 λ e1 - (2 ε + 6) e2, -4 λ e3 + (2 ε
+ 6) e4}

```

(4.1.11)

```

> NT := (k, i, j) → ContractIndices(f || k &t e || i &t e || j, DGsimplify(subs(slv[2], NJ)),
    [[1, 1], [2, 2], [3, 3]]):
S := { } : for i to 5 do for j from i + 1 to 6 do S := {op(S), NT(5, i, j)} : od: od: S
      {0, 4 t}

```

(4.1.12)

This is an SNPK structure! (NJ is NDG)

▼ **r=0**

```

> restart : with(DifferentialGeometry) : with(LieAlgebras) : with(Tensor) : with(Tools) :
    with(LinearAlgebra) :

```

```

> StructureEquations := [ [ee, ii] = p·e, [ee, jj] = -p·e, [ii, kk] = -p·e, [jj, kk] = p·e, [ee, ie]

```

$$\begin{aligned}
&= (\varepsilon + s) \cdot ee + \lambda \cdot (ii + jj) - \frac{\varepsilon + 2s}{2} \cdot kk, [ii, ie] = (\varepsilon + s) \cdot ii - \lambda \cdot (ee - kk) \\
&+ \frac{\varepsilon + 2s}{2} \cdot jj, [jj, ie] = (\varepsilon + s) \cdot jj + \lambda \cdot (ee - kk) + \frac{\varepsilon + 2s}{2} \cdot ii, [kk, ie] = (\varepsilon + s) \cdot kk \\
&+ \lambda \cdot (ii + jj) - \frac{\varepsilon + 2s}{2} \cdot ee, [e, ie] = \varepsilon \cdot e \Big], [ee, ii, jj, kk, e, ie] : L \\
&:= \text{LieAlgebraData}(\text{StructureEquations}, \text{VC})
\end{aligned}$$

$$\begin{aligned}
L := & \left[ [e1, e2] = p \, e5, [e1, e3] = -p \, e5, [e1, e6] = \left( -\frac{1}{2} \varepsilon - s \right) e4 + \lambda \, e3 + \lambda \, e2 + (\varepsilon + s) \, e1, \right. \\
& [e2, e4] = -p \, e5, [e2, e6] = \lambda \, e4 + \left( \frac{1}{2} \varepsilon + s \right) e3 + (\varepsilon + s) \, e2 - \lambda \, e1, \\
& [e3, e4] = p \, e5, [e3, e6] = -\lambda \, e4 + (\varepsilon + s) \, e3 + \left( \frac{1}{2} \varepsilon + s \right) e2 + \lambda \, e1, [e4, e6] = (\varepsilon + s) \, e4 \\
& \left. + \lambda \, e3 + \lambda \, e2 + \left( -\frac{1}{2} \varepsilon - s \right) e1, [e5, e6] = \varepsilon \, e5 \right]
\end{aligned} \tag{4.2.1}$$

$$> \text{DGsetup}(L, [e], [f]) : \text{Query}(\text{"Jacobi"}); \tag{4.2.2}$$

$$\begin{aligned}
> g := \text{evalDG}(b \cdot (f1 \&t f1 + f2 \&t f2 - f3 \&t f3 - f4 \&t f4) + (f5 \&t f5 + f6 \&t f6)); \\
& g := b \, f1 \, f1 + b \, f2 \, f2 - b \, f3 \, f3 - b \, f4 \, f4 + f5 \, f5 + f6 \, f6
\end{aligned} \tag{4.2.3}$$

By the same endomorphism freedom reason as above we fix  $q=i$

$$> J0 := \text{Matrix}([ [0, -1, 0, 0, 0, 0], [1, 0, 0, 0, 0, 0], [0, 0, 0, 1, 0, 0], [0, 0, -1, 0, 0, 0], \\ [0, 0, 0, 0, 0, -1], [0, 0, 0, 0, 1, 0] ])$$

$$J0 := \begin{bmatrix} 0 & -1 & 0 & 0 & 0 & 0 \\ 1 & 0 & 0 & 0 & 0 & 0 \\ 0 & 0 & 0 & 1 & 0 & 0 \\ 0 & 0 & -1 & 0 & 0 & 0 \\ 0 & 0 & 0 & 0 & 0 & -1 \\ 0 & 0 & 0 & 0 & 1 & 0 \end{bmatrix} \tag{4.2.4}$$

$$> J0 := \text{Matrix}([ [0, -(R^2 + t^2 + 1)/(2 \cdot t), -(R^2 - t^2 + 1)/(2 \cdot t), -R, 0, 0], [(R^2 + t^2 + 1)/(2 \cdot t), 0, R, -(R^2 - t^2 + 1)/(2 \cdot t), 0, 0], [-(R^2 - t^2 + 1)/(2 \cdot t), R, 0, (R^2 + t^2 + 1)/(2 \cdot t), 0, 0], [-R, -(R^2 - t^2 + 1)/(2 \cdot t), -(R^2 + t^2 + 1)/(2 \cdot t), 0, 0, 0], [0, 0, 0, 0, 0, -1], [0, 0, 0, 0, 1, 0] ]);$$

$$J0 := \tag{4.2.5}$$

$$\begin{aligned}
& \left[ \left[ 0, -\frac{1}{2} \frac{R^2 + t^2 + 1}{t}, -\frac{1}{2} \frac{R^2 - t^2 + 1}{t}, -R, 0, 0 \right], \right. \\
& \left[ \frac{1}{2} \frac{R^2 + t^2 + 1}{t}, 0, R, -\frac{1}{2} \frac{R^2 - t^2 + 1}{t}, 0, 0 \right], \\
& \left[ -\frac{1}{2} \frac{R^2 - t^2 + 1}{t}, R, 0, \frac{1}{2} \frac{R^2 + t^2 + 1}{t}, 0, 0 \right], \\
& \left. \left[ -R, -\frac{1}{2} \frac{R^2 - t^2 + 1}{t}, -\frac{1}{2} \frac{R^2 + t^2 + 1}{t}, 0, 0, 0 \right] \right]
\end{aligned}$$

$$\begin{bmatrix} 0, 0, 0, 0, 0, -1 \\ 0, 0, 0, 0, 1, 0 \end{bmatrix}$$

>  $J := \text{Transformation}(\text{VC}, \text{VC}, J0) : \text{Jtensor} := \text{convert}(J0, \text{DGtensor}, [ ["\text{con\_bas}",$   
 $\text{"cov\_bas"}], [ []]) :$

>  $\omega := \text{convert}(\text{ContractIndices}(\text{Jtensor}, g, [[1, 1]]), \text{DGform});$

$$\omega := b f1 \wedge f2 + b f3 \wedge f4 + f5 \wedge f6 \quad (4.2.6)$$

>  $\text{nabla} := \text{Christoffel}(g) :$

>  $\text{Nabla}\Omega := \text{DGsimplify}(\text{subs}(\{\text{temp} = 0\}, \text{CovariantDerivative}(\omega, \text{nabla}))) :$

>  $\text{SkewNabla}\Omega := \text{SymmetrizeIndices}(\text{Nabla}\Omega, [1, 2, 3], \text{"SkewSymmetric"}) :$

>  $\text{solve}(\text{DGinfo}(\text{evalDG}(\text{Nabla}\Omega - \text{SkewNabla}\Omega), \text{"CoefficientSet"})) ;$   
 $\{b = 0, p = 0, s = s, \epsilon = \epsilon, \lambda = \lambda\}, \{b = b, p = 0, s = 0, \epsilon = 0, \lambda = 0\}$  (4.2.7)

These solutions are both not admissible due to  $b=0$  or  $p=0$  (in fact the latter solution is Kahler but not SNPK).

### A3.5

>  $\text{restart} : \text{with}(\text{DifferentialGeometry}) : \text{with}(\text{LieAlgebras}) : \text{with}(\text{Tensor}) : \text{with}(\text{Tools}) :$   
 $\text{with}(\text{LinearAlgebra}) :$

>  $\text{StructureEquations} := [[\text{LAI}, \text{LAj}] = 2 * \text{LAK}, [\text{LAI}, \text{LAK}] = -2 * \text{LAj}, [\text{LAj}, \text{LAK}] = -2 * \text{LAI},$   
 $[\text{LAI}, \text{ee}] = \text{ii}, [\text{LAI}, \text{ii}] = -\text{ee}, [\text{LAI}, \text{jj}] = \text{kk}, [\text{LAI}, \text{kk}] = -\text{jj}, [\text{LAj}, \text{ee}] = \text{jj}, [\text{LAj}, \text{ii}] = -\text{kk},$   
 $[\text{LAj}, \text{jj}] = \text{ee}, [\text{LAj}, \text{kk}] = -\text{ii}, [\text{LAK}, \text{ee}] = \text{kk}, [\text{LAK}, \text{ii}] = \text{jj}, [\text{LAK}, \text{jj}] = \text{ii}, [\text{LAK}, \text{kk}] = \text{ee},$   
 $[\text{ee}, \text{ii}] = (\epsilon/l + l) * e - \text{LAI}, [\text{ee}, \text{jj}] = (-\epsilon/l + l) * e - \text{LAj}, [\text{ee}, \text{kk}] = -\text{LAK}, [\text{ii}, \text{jj}] =$   
 $-\text{LAK}, [\text{ii}, \text{kk}] = (-\epsilon/l + l) * e + \text{LAj}, [\text{jj}, \text{kk}] = (\epsilon/l + l) * e + \text{LAI}, [\text{ee}, e] = 3 * \epsilon * ((1$   
 $/4 * (\epsilon/l + l)) * \text{ii} + (1/4 * (\epsilon/l - l)) * \text{jj}), [\text{ii}, e] = 3 * \epsilon * (-(1/4 * (\epsilon/l + l)) * \text{ee}$   
 $+ (1/4 * (\epsilon/l - l)) * \text{kk}), [\text{jj}, e] = 3 * \epsilon * (-(1/4 * (\epsilon/l + l)) * \text{kk} + (1/4 * (\epsilon/l$   
 $- l)) * \text{ee}), [\text{kk}, e] = 3 * \epsilon * ((1/4 * (\epsilon/l + l)) * \text{jj} + (1/4 * (\epsilon/l - l)) * \text{ii}), [\text{LAI},$   
 $\text{LAj}, \text{LAK}, \text{ee}, \text{ii}, \text{jj}, \text{kk}, e, \text{ie}] :$

$L := \text{LieAlgebraData}(\text{StructureEquations}, \text{VC}) :$

>  $\text{DGsetup}(L, [e], [f]) : \text{Query}(\{\epsilon, l\}, \text{"Jacobi"}) ;$

$\text{true}, \{0, -3\epsilon^2 + 3, 3\epsilon^2 - 3\}, \{\{\epsilon = 1, l = l\}, \{\epsilon = -1, l = l\}\}, \left[ \left[ [e1, e2] = 2 e3, [e1, e3] = \right. \right. \quad (5.1)$

$$-2 e2, [e1, e4] = e5, [e1, e5] = -e4, [e1, e6] = e7, [e1, e7] = -e6, [e2, e3] = -2 e1,$$

$$[e2, e4] = e6, [e2, e5] = -e7, [e2, e6] = e4, [e2, e7] = -e5, [e3, e4] = e7, [e3, e5] = e6,$$

$$[e3, e6] = e5, [e3, e7] = e4, [e4, e5] = \left(\frac{1}{l} + l\right) e8 - e1, [e4, e6] = \left(-\frac{1}{l} + l\right) e8$$

$$- e2, [e4, e7] = -e3, [e4, e8] = \left(\frac{3}{4l} - \frac{3}{4} l\right) e6 + \left(\frac{3}{4l} + \frac{3}{4} l\right) e5, [e5, e6] = -e3,$$

$$[e5, e7] = \left(-\frac{1}{l} + l\right) e8 + e2, [e5, e8] = \left(\frac{3}{4l} - \frac{3}{4} l\right) e7 + \left(-\frac{3}{4l} - \frac{3}{4} l\right) e4, [e6,$$



$$\begin{aligned}
e7] &= \left( \frac{1}{l} + l \right) e8 + e1, [e6, e8] = \left( -\frac{3}{4l} - \frac{3}{4} l \right) e7 + \left( \frac{3}{4l} - \frac{3}{4} l \right) e4, [e7, e8] \\
&= \left( \frac{3}{4l} + \frac{3}{4} l \right) e6 + \left( \frac{3}{4l} - \frac{3}{4} l \right) e5, \left[ [e1, e2] = 2 e3, [e1, e3] = -2 e2, [e1, e4] \right. \\
&= e5, [e1, e5] = -e4, [e1, e6] = e7, [e1, e7] = -e6, [e2, e3] = -2 e1, [e2, e4] = e6, [e2, \\
&e5] = -e7, [e2, e6] = e4, [e2, e7] = -e5, [e3, e4] = e7, [e3, e5] = e6, [e3, e6] = e5, [e3, \\
&e7] = e4, [e4, e5] = \left( -\frac{1}{l} + l \right) e8 - e1, [e4, e6] = \left( \frac{1}{l} + l \right) e8 - e2, [e4, e7] = -e3, \\
&[e4, e8] = \left( \frac{3}{4l} + \frac{3}{4} l \right) e6 + \left( \frac{3}{4l} - \frac{3}{4} l \right) e5, [e5, e6] = -e3, [e5, e7] = \left( \frac{1}{l} \right. \\
&+ l \left. \right) e8 + e2, [e5, e8] = \left( \frac{3}{4l} + \frac{3}{4} l \right) e7 + \left( -\frac{3}{4l} + \frac{3}{4} l \right) e4, [e6, e7] = \left( -\frac{1}{l} \right. \\
&+ l \left. \right) e8 + e1, [e6, e8] = \left( -\frac{3}{4l} + \frac{3}{4} l \right) e7 + \left( \frac{3}{4l} + \frac{3}{4} l \right) e4, [e7, e8] = \left( \frac{3}{4l} \right. \\
&\left. - \frac{3}{4} l \right) e6 + \left( \frac{3}{4l} + \frac{3}{4} l \right) e5 \left. \right]
\end{aligned}$$

- > g := evalDG(temp·(-f1 &t f1 + f2 &t f2 + f3 &t f3) + ((f4 &t f4 + f5 &t f5) - (f6 &t f6 + f7 &t f7)) + b·(f8 &t f8 + f9 &t f9)) :
  - > J0 := Matrix([ [0, 0, 0, 0, 0, 0, 0, 0, 0], [0, 0, 0, 0, 0, 0, 0, 0, 0], [0, 0, 0, 0, -((1 + r^2 + t^2)/(2 t)), -((1 + r^2 - t^2)/(2 t)), -r, 0, 0], [0, 0, 0, 0, (1 + r^2 + t^2)/(2 t), 0, r, -((1 + r^2 - t^2)/(2 t)), 0, 0], [0, 0, 0, 0, -(1 + r^2 - t^2)/(2 t), r, 0, (1 + r^2 + t^2)/(2 t), 0, 0], [0, 0, 0, 0, -r, -(1 + r^2 - t^2)/(2 t), -(1 + r^2 + t^2)/(2 t), 0, 0, 0], [0, 0, 0, 0, 0, 0, 0, 0, 0, -1], [0, 0, 0, 0, 0, 0, 0, 0, 1, 0] ]):
  - > J := convert(J0, DGtensor, [ ["con\_bas", "cov\_bas"], [ ] ]);
- $$\begin{aligned}
J := & -\frac{r^2 + t^2 + 1}{2 t} e4 f5 - \frac{r^2 - t^2 + 1}{2 t} e4 f6 - r e4 f7 + \frac{r^2 + t^2 + 1}{2 t} e5 f4 + r e5 f6 \\
& - \frac{r^2 - t^2 + 1}{2 t} e5 f7 - \frac{r^2 - t^2 + 1}{2 t} e6 f4 + r e6 f5 + \frac{r^2 + t^2 + 1}{2 t} e6 f7 - r e7 f4 \\
& - \frac{r^2 - t^2 + 1}{2 t} e7 f5 - \frac{r^2 + t^2 + 1}{2 t} e7 f6 - e8 f9 + e9 f8
\end{aligned} \tag{5.2}$$
- > w := ContractIndices(J, g, [[1, 1]]);
- $$\begin{aligned}
w := & \frac{r^2 + t^2 + 1}{2 t} f4 f5 + \frac{r^2 - t^2 + 1}{2 t} f4 f6 + r f4 f7 - \frac{r^2 + t^2 + 1}{2 t} f5 f4 - r f5 f6 \\
& + \frac{r^2 - t^2 + 1}{2 t} f5 f7 - \frac{r^2 - t^2 + 1}{2 t} f6 f4 + r f6 f5 + \frac{r^2 + t^2 + 1}{2 t} f6 f7 - r f7 f4 \\
& - \frac{r^2 - t^2 + 1}{2 t} f7 f5 - \frac{r^2 + t^2 + 1}{2 t} f7 f6 + b f8 f9 - b f9 f8
\end{aligned} \tag{5.3}$$
- > nabla := Christoffel(g) :
  - > NablaOmega := DGsimplify(subs({temp=0}, CovariantDerivative(w, nabla))) :
  - > SkewNablaOmega := SymmetrizeIndices(NablaOmega, [1, 2, 3], "SkewSymmetric") :
  - > solve(DGinfo(evalDG(NablaOmega-SkewNablaOmega), "CoefficientSet"));

$$\{b=0, \varepsilon=l^2 t^2, l=l, r=0, t=t\}, \{b=0, \varepsilon=0, l=l, r=r, t=t\} \quad (5.4)$$

$$\begin{aligned} &> \text{DGinfo}(\text{evalDG}(\text{NablaOmega} - \text{SkewNablaOmega}), \text{"CoefficientSet"}); \\ &\left\{ \frac{r a (b^2 - 4)}{b}, -\frac{1}{3} b^2, -\frac{1}{6} b^2, \frac{1}{3} b^2, \frac{1}{6} b^2, -\frac{1}{3} b a, -\frac{1}{6} b a, \frac{1}{3} b a, \frac{1}{6} b a, \right. \\ &\quad -\frac{1}{2} \frac{b^3 t^2 + 2 a r^2 - 2 b t^2 + 2 a}{b t}, \frac{1}{2} \frac{b^3 t^2 + 2 a r^2 - 2 b t^2 + 2 a}{b t}, \\ &\quad -\frac{1}{2} \frac{a b^2 r^2 + a b^2 - 2 a r^2 + 2 b t^2 - 2 a}{b t}, \frac{1}{2} \frac{a b^2 r^2 + a b^2 - 2 a r^2 + 2 b t^2 - 2 a}{b t}, \\ &\quad -\frac{1}{2} \frac{a b^2 r^2 - b^3 t^2 + a b^2 - 4 a r^2 + 4 b t^2 - 4 a}{b t}, \\ &\quad \frac{1}{2} \frac{a b^2 r^2 - b^3 t^2 + a b^2 - 4 a r^2 + 4 b t^2 - 4 a}{b t}, -\frac{r a (b^2 - 4)}{b}, -\frac{1}{2} \frac{r a (b^2 - 4)}{b}, \\ &\quad \left. \frac{1}{2} \frac{r a (b^2 - 4)}{b}, -2 r + \frac{1}{2} b^2 r, 2 r - \frac{1}{2} b^2 r, -b^2 r + 4 r, b^2 r - 4 r \right\} \end{aligned} \quad (5.5)$$

No Solutions

## A4.1

$$\begin{aligned} &> \text{restart} : \text{with}(\text{DifferentialGeometry}) : \text{with}(\text{LieAlgebras}) : \text{with}(\text{Tensor}) : \text{with}(\text{Tools}) : \\ &\quad \text{with}(\text{LinearAlgebra}) : \\ &> \text{StructureEquations} := [[i, j] = k, [i, k] = -j, [j, k] = -i, [i2, j2] = k2, [i2, k2] = -j2, [j2, k2] = \\ &\quad -i2], [i, j, k, i2, j2, k2] : \\ &\quad L := \text{LieAlgebraData}(\text{StructureEquations}, \text{Dsu11}) : \\ &> \text{DGsetup}(L, [e], [f]) : \\ &> w := \text{evalDG}(-f1 \&w f4 + f2 \&w f5 + f3 \&w f6) : \\ &> J0 := \text{Matrix}\left(\left[\left[\begin{matrix} r, 0, 0, -\frac{(1+r^2)}{t}, 0, 0 \end{matrix}\right], \left[\begin{matrix} 0, r, 0, 0, -\frac{(1+r^2)}{t}, 0 \end{matrix}\right], \left[\begin{matrix} 0, 0, r, 0, 0, 0 \end{matrix}\right], \right. \right. \\ &\quad \left. \left. -\frac{(1+r^2)}{t}\right], \left[\begin{matrix} t, 0, 0, -r, 0, 0 \end{matrix}\right], \left[\begin{matrix} 0, t, 0, 0, -r, 0 \end{matrix}\right], \left[\begin{matrix} 0, 0, t, 0, 0, -r \end{matrix}\right]\right] \right) : \\ &> J := \text{convert}(J0, \text{DGtensor}, [[\text{"con\_bas"}, \text{"cov\_bas"}], []); \\ &\quad J := r e1 f1 - \frac{r^2 + 1}{t} e1 f4 + r e2 f2 - \frac{r^2 + 1}{t} e2 f5 + r e3 f3 - \frac{r^2 + 1}{t} e3 f6 + t e4 f1 \\ &\quad - r e4 f4 + t e5 f2 - r e5 f5 + t e6 f3 - r e6 f6 \quad (6.1) \\ &> g := \text{ContractIndices}(J, w, [[1, 1]]); \\ &\quad g := t f1 f1 - r f1 f4 - t f2 f2 + r f2 f5 - t f3 f3 + r f3 f6 - r f4 f1 + \frac{r^2 + 1}{t} f4 f4 + r f5 f2 \\ &\quad - \frac{r^2 + 1}{t} f5 f5 + r f6 f3 - \frac{r^2 + 1}{t} f6 f6 \quad (6.2) \\ &> nabla := \text{Christoffel}(g) : \\ &> \text{NablaOmega} := \text{DGsimplify}(\text{subs}(\{\text{temp} = 0\}, \text{CovariantDerivative}(w, nabla))) : \\ &> \text{SkewNablaOmega} := \text{SymmetrizeIndices}(\text{NablaOmega}, [1, 2, 3], \text{"SkewSymmetric"}) : \\ &> \text{solve}(\text{DGinfo}(\text{evalDG}(\text{NablaOmega} - \text{SkewNablaOmega}), \text{"CoefficientSet"})); \\ &\quad \{r = \text{RootOf}(3 \_Z^2 - 1), t = 2 \text{RootOf}(3 \_Z^2 - 1)\} \quad (6.3) \end{aligned}$$

This solution is SNPK. Using the diffeomorphism  $SL_2 \approx S^1 \times R^2$ , it is supported on  $(S^1 \times R^2) \times (S^1 \times R^2)$  and has signature  $(4,2)=(2,1)+(2,1)$ . The corresponding definite signature solution is supported on  $S^3 \times S^3$ .

## A4.2

```

> restart : with(DifferentialGeometry) : with(LieAlgebras) : with(Tensor) : with(Tools) :
  with(LinearAlgebra) :
> StructureEquations := [[i, j] = k, [i, k] = -j, [j, k] = -i, [i, j2] = k2, [i, k2] = -j2, [j, k2] =
  -i2, [i2, j] = k2, [i2, k] = -j2, [j2, k] = -i2, [i2, j2] = -k, [i2, k2] = j, [j2, k2] = i], [i, j, k,
  i2, j2, k2] :
  L := LieAlgebraData(StructureEquations, Dsu11) :
> DGsetup(L, [e], [f]) :
> w := evalDG(-f1 &w f4 + f2 &w f5 + f3 &w f6) :
> J0 := Matrix([[ [r, 0, 0, - (1 + r^2)/t, 0, 0], [0, r, 0, 0, - (1 + r^2)/t, 0], [0, 0, r, 0, 0, 0,
  - (1 + r^2)/t], [t, 0, 0, -r, 0, 0], [0, t, 0, 0, -r, 0], [0, 0, t, 0, 0, -r]]]) :
> J := convert(J0, DGtensor, [[ "con_bas", "cov_bas"], [ ]]);
J := r e1 f1 - (r^2 + 1)/t e1 f4 + r e2 f2 - (r^2 + 1)/t e2 f5 + r e3 f3 - (r^2 + 1)/t e3 f6 + t e4 f1
      - r e4 f4 + t e5 f2 - r e5 f5 + t e6 f3 - r e6 f6
> g := ContractIndices(J, w, [[1, 1]]);
g := t f1 f1 - r f1 f4 - t f2 f2 + r f2 f5 - t f3 f3 + r f3 f6 - r f4 f1 + (r^2 + 1)/t f4 f4 + r f5 f2
      - (r^2 + 1)/t f5 f5 + r f6 f3 - (r^2 + 1)/t f6 f6
> nabla := Christoffel(g) :
> NablaOmega := DGsimplify(subs({temp = 0}, CovariantDerivative(w, nabla))) :
> SkewNablaOmega := SymmetrizeIndices(NablaOmega, [1, 2, 3], "SkewSymmetric") :
> solve(DGinfo(evalDG(NablaOmega - SkewNablaOmega), "CoefficientSet"));
      {r = 0, t = RootOf(3 _Z^2 + 1)}

```

This solution is not real

## A4.3

```

> restart : with(DifferentialGeometry) : with(LieAlgebras) : with(Tensor) : with(Tools) :
  with(LinearAlgebra) :
> StructureEquations := [[i, j] = k, [i, k] = -j, [j, k] = -i, [i, j, k, i2, j2, k2] :
  L := LieAlgebraData(StructureEquations, Dsu11) :
> DGsetup(L, [e], [f]) :
> w := evalDG(-f1 &w f4 + f2 &w f5 + f3 &w f6) :
> J0 := Matrix([[ [r, 0, 0, - (1 + r^2)/t, 0, 0], [0, r, 0, 0, - (1 + r^2)/t, 0], [0, 0, r, 0, 0, 0,
  - (1 + r^2)/t], [t, 0, 0, -r, 0, 0], [0, t, 0, 0, -r, 0], [0, 0, t, 0, 0, -r]]]) :

```

$$J := \text{convert}(J0, \text{DGtensor}, [[\text{"con\_bas"}, \text{"cov\_bas"}], []);$$

$$J := r e1 f1 - \frac{r^2+1}{t} e1 f4 + r e2 f2 - \frac{r^2+1}{t} e2 f5 + r e3 f3 - \frac{r^2+1}{t} e3 f6 + t e4 f1 - r e4 f4 + t e5 f2 - r e5 f5 + t e6 f3 - r e6 f6 \quad (8.1)$$

$$g := \text{ContractIndices}(J, w, [[1, 1]]);$$

$$g := t f1 f1 - r f1 f4 - t f2 f2 + r f2 f5 - t f3 f3 + r f3 f6 - r f4 f1 + \frac{r^2+1}{t} f4 f4 + r f5 f2 - \frac{r^2+1}{t} f5 f5 + r f6 f3 - \frac{r^2+1}{t} f6 f6 \quad (8.2)$$

$$\begin{aligned} & \text{nabla} := \text{Christoffel}(g) : \\ & \text{NablaOmega} := \text{DGsimplify}(\text{subs}(\{\text{temp} = 0\}, \text{CovariantDerivative}(w, \text{nabla}))) : \\ & \text{SkewNablaOmega} := \text{SymmetrizeIndices}(\text{NablaOmega}, [1, 2, 3], \text{"SkewSymmetric"}) : \\ & \text{solve}(\text{DGinfo}(\text{evalDG}(\text{NablaOmega} - \text{SkewNablaOmega}), \text{"CoefficientSet"})); \\ & \text{DGinfo}(\text{evalDG}(\text{NablaOmega} - \text{SkewNablaOmega}), \text{"CoefficientSet"}); \\ & \left\{ \frac{(r^2+1)r}{t}, -\frac{(r^2+1)r}{t}, -\frac{1}{2} \frac{(r^2+1)r}{t}, \frac{1}{2} \frac{(r^2+1)r}{t}, -\frac{1}{3} - r^2, -\frac{1}{6} - \frac{1}{2} r^2, \frac{1}{3} + r^2, \frac{1}{6} + \frac{1}{2} r^2 \right\} \end{aligned} \quad (8.3)$$

No solutions

## A4.4

$$\begin{aligned} & \text{restart} : \text{with}(\text{DifferentialGeometry}) : \text{with}(\text{LieAlgebras}) : \text{with}(\text{Tensor}) : \text{with}(\text{Tools}) : \\ & \quad \text{with}(\text{LinearAlgebra}) : \\ & \text{StructureEquations} := [[i, j] = k2, [i, k] = -j2, [j, k] = -i2, [i, j, k, i2, j2, k2]] : \\ & L := \text{LieAlgebraData}(\text{StructureEquations}, \text{Dsul1}) : \\ & \text{DGsetup}(L, [e], [f]) : \\ & w := \text{evalDG}(-f1 \&w f4 + f2 \&w f5 + f3 \&w f6) : \\ & J0 := \text{Matrix}\left(\left[\left[\begin{matrix} r & 0 & 0 & -\frac{(1+r^2)}{t} & 0 & 0 \end{matrix}\right], \left[\begin{matrix} 0 & r & 0 & 0 & -\frac{(1+r^2)}{t} & 0 \end{matrix}\right], \left[\begin{matrix} 0 & 0 & r & 0 & 0 & 0 \end{matrix}\right], \right. \right. \\ & \quad \left. \left. -\frac{(1+r^2)}{t} \right], [t, 0, 0, -r, 0, 0], [0, t, 0, 0, -r, 0], [0, 0, t, 0, 0, -r] \right] \right) : \\ & J := \text{convert}(J0, \text{DGtensor}, [[\text{"con\_bas"}, \text{"cov\_bas"}], []); \\ & J := r e1 f1 - \frac{r^2+1}{t} e1 f4 + r e2 f2 - \frac{r^2+1}{t} e2 f5 + r e3 f3 - \frac{r^2+1}{t} e3 f6 + t e4 f1 - r e4 f4 + t e5 f2 - r e5 f5 + t e6 f3 - r e6 f6 \quad (9.1) \end{aligned}$$

$$g := \text{ContractIndices}(J, w, [[1, 1]]);$$

$$g := t f1 f1 - r f1 f4 - t f2 f2 + r f2 f5 - t f3 f3 + r f3 f6 - r f4 f1 + \frac{r^2+1}{t} f4 f4 + r f5 f2 - \frac{r^2+1}{t} f5 f5 + r f6 f3 - \frac{r^2+1}{t} f6 f6 \quad (9.2)$$

$$\begin{aligned} & \text{nabla} := \text{Christoffel}(g) : \\ & \text{NablaOmega} := \text{DGsimplify}(\text{subs}(\{\text{temp} = 0\}, \text{CovariantDerivative}(w, \text{nabla}))) : \\ & \text{SkewNablaOmega} := \text{SymmetrizeIndices}(\text{NablaOmega}, [1, 2, 3], \text{"SkewSymmetric"}) : \end{aligned}$$

```

| > solve(DGinfo(evalDG(NablaOmega-SkewNablaOmega), "CoefficientSet"));
|_ {r=RootOf(_Z^2+1), t=t}
|_ Solution is not real.

```

**(9.3)**
